# Supplementary material for: REMS: a unified solution representation, problem modeling and metaheuristic algorithm design for general combinatorial optimization problems
Source: arXiv:2505.17108 source file (2026-03-02)
Supplement: Supplementary file 1 [file Supplementary_material_for_REMS.pdf]

# Supplementary Material

## 1 Problem Model and Setting

1.1 Multi-depot vehicle routing problem with time windows (MDVRPTW)[1]

MDVRPTW is an extension of the Vehicle Routing Problem (VRP), incorporating multiple depots and time window constraints. In MDVRPTW, a fleet of vehicles is stationed at several depots, and the goal is to determine the optimal set of routes for each vehicle.

Assume that there are $n$ customers and $m$ vehicles, which are respectively put into task set $T$ and resource set $R$. For $R_i,\ i\in\mathcal{I}=\{1,\cdots,m\}$, the resource attributions include index $d_i^R$, capacity $A_{i,1}^R$, maximum transportation distance $A_{i,2}^R$, depart and return depot $A_{i,3}^R$, fixed cost $A_{i,4}^R$, and transportation cost $A_{i,5}^R$ for unit distance. Regarding $T_j,\ j\in\mathcal{J}=\{1,\cdots,n\}$, the attributions involve index $d_j^T$, demand $A_{j,1}^T$, earliest allowed service time $A_{j,2}^T$, latest allowed service time $A_{j,3}^T$, and service duration $A_{j,4}^T$. There are also some other problem data like number of depots $np$ and depot capacity $c_i^{depot}, i\in\{1,\cdots,np\}$. Moreover, $d_{j,j'},\ j,j'\in\mathcal{J}\cup\{n+1,\cdots,n+np\}$ is the travel distance from $j$ and $j'$, and $t_{j,j'},\ j,j'\in\mathcal{J}\cup\{n+1,\cdots,n+np\}$ is the travel time from $j$ to $j'$, where $\mathcal{J}$ is the task index set and $\{n+1,\cdots,n+np\}$ corresponds to the index of depots.

About the variables in (6), $X_i,\ i\in\mathcal{I}$ is a sequence variable. $x_{i,k},\ i\in\mathcal{I},k\in\mathcal{K}_i=\{1,\cdots,n_i\}$ is the task arranged in the $k$ th position of $R_i$. The attribute variables include the assignment binary matrix $Y^C$ shown in (7), start serve time $Y^S$ in (8), and end serve time $Y^E$ in (9). Moreover, $Y^U$ is employed to determine whether any task is assigned to a resource, where $y_i^U,\ i\in\mathcal{I}$ is calculated by

$$y_i^U=\begin{cases}0, \text{ if } |X_i|=0\\ 1, \text{ otherwise}\end{cases}, \tag{S-1}$$

Another attribute variable $Y^D$ can denote the cumulative travel distance when arriving at a task, where $y_{i,j,k}^D,\ i\in\mathcal{I},j\in\mathcal{J},k\in\mathcal{K}$ is expressed as

$$y_{i,j,k}^D=\begin{cases} d_{A_{i,3}^R,j}\,y_{i,j,k}^C, \text{ if } k=1\\ \sum_{j'\in\mathcal{J}}(y_{i,j',k-1}^D+d_{j',j})y_{i,j,k}^C, \text{ otherwise}\end{cases}, \tag{S-2}$$

The objective function is to minimize the total cost, which can be denoted as

$$\min\sum_{i\in\mathcal{I}}A_{i,4}^R y_i^U+\sum_{j\in\mathcal{J}}\sum_{i\in\mathcal{I}}A_{i,5}^R(y_{i,j,n_i}^D+d_{j,A_{i,3}^R})y_{i,j,n_i}^C, \tag{S-3}$$

where the first term is the fixed cost and the second term manifests the cost along with transportation distance.

The first constraint, which ensures each task is executed exactly one time on all resources, can be denoted as the form of (20), where $\rho_{i,j,k}^T=1,\ i\in\mathcal{I},j\in\mathcal{J},k\in\mathcal{K}_i$, $\theta_j^T=1,\ j\in\mathcal{J}$, and the relational operator is "=", i.e.,

$$\sum_{k\in\mathcal{K}_i}\sum_{i\in\mathcal{I}}y_{i,j,k}^C=1,\ j\in\mathcal{J}, \tag{S-4}$$

The capacity constraint of vehicles can be expressed by (18), and $\rho_{i,j,k}^R=A_{j,1}^T\ i\in\mathcal{I},k\in\mathcal{K}_i$, $\theta_i^R=A_{i,1}^R,\ i\in\mathcal{I}$, and the relational operator is "$\le$", i.e,

$$\sum_{k\in\mathcal{K}_i}\sum_{j\in\mathcal{J}}A_{j,1}^T y_{i,j,k}^C\le A_{i,1}^R,\ i\in\mathcal{I}, \tag{S-5}$$

The transportation distance constraint of vehicles can be presented as

$$\sum_{j\in\mathcal{J}}(y^{D}_{i,j,n_i}+d_{j,A^{R}_{i,3}})y^{C}_{i,j,n_i}\le A^{R}_{i,2},\ i\in\mathcal{I} \tag{S-6}$$

The capacity constraint of depots is expressed as

$$\sum\{\sum_{k\in\mathcal{K}_i}\sum_{j\in\mathcal{J}}A^{T}_{j,1}y^{C}_{i,j,k}\,|\,\text{if }A^{R}_{i,3}=r,i\in\mathcal{I}\}\le c^{depot}_{r},\ r\in\{1,\cdots,np\} \tag{S-7}$$

The time window constraint can be

$$y^{S}_{i,j,k}\ge A^{T}_{j,2},y^{E}_{i,j,k}\le A^{T}_{j,3},\ i\in\mathcal{I},j\in\mathcal{J},k\in\mathcal{K}_i \tag{S-8}$$

The parameters in MDVRPTW[1] are presented in Table S-1 including the number of depots *ND*, the number of vehicles in each depot *NV*, the number of customers *NC*, as well as maximum transportation distance *MD* and maximum capacity *MC* for each vehicle. The running time MaxTime(s) is also presented in Table S-1, which changes with the problem scale and complexity. Furthermore, the fixed cost for each vehicle is set to 1,000, and the transportation cost of unit distance is set to 5.

**Table S-1** Brief information on 20 MDVRPTW problems.

| Pro. | *ND* | *NV* | *NC* | *MD* | *MC* | MaxTime(s) |
|---|---|---|---|---|---|---|
| MDVRPTW01 | 4 | 2 | 48 | 500 | 200 | 1 800 |
| MDVRPTW02 | 4 | 3 | 96 | 480 | 195 | 3 600 |
| MDVRPTW03 | 4 | 4 | 144 | 460 | 190 | 3 600 |
| MDVRPTW04 | 4 | 5 | 192 | 440 | 185 | 12 000 |
| MDVRPTW05 | 4 | 6 | 240 | 420 | 180 | 18 000 |
| MDVRPTW06 | 4 | 7 | 288 | 400 | 175 | 18 000 |
| MDVRPTW07 | 6 | 2 | 72 | 500 | 200 | 1 800 |
| MDVRPTW08 | 6 | 3 | 144 | 475 | 190 | 7 200 |
| MDVRPTW09 | 6 | 4 | 216 | 450 | 180 | 12 000 |
| MDVRPTW10 | 6 | 5 | 288 | 425 | 170 | 24 000 |
| MDVRPTW11 | 4 | 1 | 48 | 500 | 200 | 3 600 |
| MDVRPTW12 | 4 | 2 | 96 | 480 | 195 | 3 600 |
| MDVRPTW13 | 4 | 3 | 144 | 460 | 190 | 7 200 |
| MDVRPTW14 | 4 | 4 | 192 | 440 | 185 | 7 200 |
| MDVRPTW15 | 4 | 5 | 240 | 420 | 180 | 36 000 |
| MDVRPTW16 | 4 | 6 | 288 | 400 | 175 | 36 000 |
| MDVRPTW17 | 6 | 1 | 72 | 500 | 200 | 3 600 |
| MDVRPTW18 | 6 | 2 | 144 | 475 | 190 | 5 400 |
| MDVRPTW19 | 6 | 3 | 216 | 450 | 180 | 36 000 |
| MDVRPTW20 | 6 | 4 | 288 | 425 | 170 | 36 000 |

1.2 Vehicle routing problem with pickup and delivery (VRPPD)[2]

VRPPD belongs to a variant of VRP, similar to MDVRPTW, we still regard $n$ customers and $m$ vehicles as tasks and resources, respectively. The attributes of $R_i$, $i\in\mathcal{I}$ include index $d^{R}_{i}$, capacity $A^{R}_{i,1}$, and maximum transportation distance $A^{R}_{i,2}$. The attributes of $T_j$, $j\in\mathcal{J}$ involve index $d^{T}_{j}$, demand $A^{T}_{j,1}$, pickup or delivery index $A^{T}_{j,2}$ ($A^{T}_{j,2}=0$ denotes $T_j$ has a pickup requirement; otherwise, $T_j$ possesses a delivery demand). In addition, $d_{j,j'}, j, j'\in\{0,\cdots,n\}$ is the travel distance from $j$ and $j'$, where 0 is the index of the depot and $\{1,\cdots,n\}$ is corresponds to the task index.

For the variables in (6), $X_i$, $i\in\mathcal{I}$ is a sequence variable. Similarly, the assignment binary

[1] The test suit comes from http://neumann.hec.ca/chairedistributique/data/mdvrptw/.

matrix $Y^C$ is expressed by (7) and $Y^D$ denotes the cumulative travel distance when arriving at a task, where $y^D_{i,j,k}$, $i \in \mathcal{I}, j \in \mathcal{J}, k \in \mathcal{K}$ is calculated by

$$y^D_{i,j,k} = \begin{cases} d_{0,j} y^C_{i,j,k}, \text{ if } k=1 \\ \sum_{j' \in \mathcal{J}} (y^D_{i,j',k-1} + d_{j',j}) y^C_{i,j,k}, \text{ otherwise} \end{cases}, \tag{S-9}$$

The objective is to minimize the total travel distance and is expressed as

$$\min \sum_{j \in \mathcal{J}} \sum_{i \in \mathcal{I}} A^R_{i,5} (y^U_{i,j,n_i} + d_{j,0}) y^C_{i,j,n_i} \tag{S-10}$$

The constraint that ensures each task is executed exactly one time on all resources, can be denoted as (S-4) and the capacity constraint of vehicles can be expressed by (S-5). Moreover, the transportation distance constraint of vehicles can be denoted like (S-6), i.e.,

$$\sum_{j \in \mathcal{J}} (y^D_{i,j,n_i} + d_{j,0}) y^C_{i,j,n_i} \le A^R_{i,2},\ i \in \mathcal{I} \tag{S-11}$$

Another important constraint guarantees the pickup occurs before delivery for a pair pick-up and delivery demand, which can be represented by (22).

Concerning VRPPD, we randomly select 30 VRPPD problems from the original test suit [2]. Each instance contains 100 customers, and the number of vehicles is set at 15. The maximum transportation distance and capacity for each vehicle are established at 400 and 100, respectively. Additionally, the maximum iteration number MaxIter for all VRPPD instances is set to 10,000. The maximum running time MaxTime for each VRPPD is equal to 7,200s.

### 1.3 Generalized assignment problem (GAP)[3]

GAP aims to assign jobs to agents to minimize the total cost. We consider $m$ agents and $n$ jobs as resources and tasks, separately. The attribues of $R_i$ $i \in \mathcal{I}$ contain index $d^R_i$ and capacity $A^R_{i,1}$. The attribute of $T_j$ contains index $d^T_j$ and weight $A^T_{j,1}$. Moreover, assigning $T_j$ to $R_i$ will generate a cost $c_{i,j}$ and a consume $cs_{i,j}$.

For the variables in (6), $X_i$, $i \in \mathcal{I}$ is an assignment variable. The assignment binary matrix $Y^C$ is expressed by (7). The objective function is to minimize the total cost, which can be denoted by

$$\min \sum_{k \in \mathcal{K}_i} \sum_{j \in \mathcal{J}} \sum_{i \in \mathcal{I}} c_{i,j} y^C_{i,j,k} \tag{S-12}$$

The constraint, that ensures each task is executed exactly one time on all resources, can be denoted by (S-4). Moreover, the capacity constraint for agents can be presented by (S-5).

There are 57 GAP problems in the test suit[3], where the number of agents *NA*, number of jobs *NJ*, and maximum running time MaxTime(s) are illustrated in Table S-2.

**Table S-2** Brief information on 57 GAP problems.

| Pro. | *NA* | *NJ* | MaxTime(s) | Pro. | *NA* | *NJ* | MaxTime(s) | Pro. | *NA* | *NJ* | MaxTime(s) |
|---|---|---|---|---|---|---|---|---|---|---|---|
| GAP01 | 5 | 100 | 360 | GAP20 | 20 | 200 | 720 | GAP39 | 60 | 900 | 36 000 |
| GAP02 | 5 | 200 | 360 | GAP21 | 20 | 400 | 3 600 | GAP40 | 20 | 1600 | 36 000 |
| GAP03 | 10 | 100 | 360 | GAP22 | 30 | 900 | 72 00 | GAP41 | 40 | 1600 | 36 000 |
| GAP04 | 10 | 200 | 360 | GAP23 | 40 | 400 | 3 600 | GAP42 | 80 | 1600 | 36 000 |
| GAP05 | 20 | 100 | 360 | GAP24 | 60 | 900 | 36 000 | GAP43 | 5 | 100 | 360 |
| GAP06 | 20 | 200 | 360 | GAP25 | 20 | 1600 | 36 000 | GAP44 | 5 | 200 | 360 |
| GAP07 | 5 | 100 | 360 | GAP26 | 40 | 1600 | 36 000 | GAP45 | 10 | 100 | 360 |
| GAP08 | 5 | 200 | 360 | GAP27 | 80 | 1600 | 36 000 | GAP46 | 10 | 200 | 360 |
| GAP09 | 10 | 100 | 360 | GAP28 | 5 | 100 | 360 | GAP47 | 10 | 400 | 3 600 |

[2] The test suit comes from https://neo.lcc.uma.es/vrp/vrp-instances/vehicle-routing-problem-with-pick-up-and-deliveries/ (P1 test suit).

[3] The test suit is from https://people.brunel.ac.uk/~mastjjb/jeb/orlib/gapinfo.html.

| | | | | | | | | | | | |
|---|---|---|---|---|---|---|---|---|---|---|---|
| GAP10 | 10 | 200 | 360 | GAP29 | 5 | 200 | 360 | GAP48 | 15 | 900 | 36 000 |
| GAP11 | 20 | 100 | 360 | GAP30 | 10 | 100 | 360 | GAP49 | 20 | 100 | 360 |
| GAP12 | 20 | 200 | 360 | GAP31 | 10 | 200 | 360 | GAP50 | 20 | 200 | 720 |
| GAP13 | 5 | 100 | 360 | GAP32 | 10 | 400 | 3 600 | GAP51 | 20 | 400 | 3 600 |
| GAP14 | 5 | 200 | 360 | GAP33 | 15 | 900 | 18 000 | GAP52 | 30 | 900 | 18 000 |
| GAP15 | 10 | 100 | 360 | GAP34 | 20 | 100 | 360 | GAP53 | 40 | 400 | 18 000 |
| GAP16 | 10 | 200 | 360 | GAP35 | 20 | 200 | 360 | GAP54 | 60 | 900 | 36 000 |
| GAP17 | 10 | 400 | 3 600 | GAP36 | 20 | 400 | 3 600 | GAP55 | 20 | 1600 | 36 000 |
| GAP18 | 15 | 900 | 3 600 | GAP37 | 30 | 900 | 18 000 | GAP56 | 40 | 1600 | 36 000 |
| GAP19 | 20 | 100 | 720 | GAP38 | 40 | 400 | 3 600 | GAP57 | 80 | 1600 | 36 000 |

1.4 Capacitated facility location problem (CFLP)[4]

CFLP, which is a variant of location problem, concentrates on selecting locations from a set of possible locations. Considering that the problem has $m$ available locations and $n$ customers, we deem them as resources and tasks, separately. The attributes of $R_i$ comprises index $d_i^R$, capacity $A_{i,1}^R$, fixed cost $A_{i,2}^R$, and maximum value $A_{i,3}^R$. The attributes of $T_j$ involves index $d_j^T$ and demand $A_{j,1}^T$. Furthermore, assigning $T_j$ to $R_i$ will generate a cost $c_{i,j}$ and a value $v_{i,j}$.

Concerning the variables in (6), $X_i$, $i \in \mathcal{I}$ is an assignment variable. Likewise, the assignment binary matrix $Y^C$ is expressed by (7). Moreover, attribute variable $Y^U$ is employed to determine whether any task is assigned to a resource, where $y_i^U$, $i \in \mathcal{I}$ is calculated by (S-1). The optimal objective is to minimize the total cost, which can be represented by

$$\min \sum_{i \in \mathcal{I}} A_{i,2}^R y_i^U + \sum_{k \in \mathcal{K}_i} \sum_{j \in \mathcal{J}} \sum_{i \in \mathcal{I}} c_{i,j} y_{i,j,k}^C \tag{S-13}$$

The constraint, that ensures each task is executed exactly one time on all resources, can be denoted as (S-4) and the capacity constraints for resources can be denoted by (S-5). For the value constraints for resources can be expressed as

$$\sum_{k \in \mathcal{K}_i} \sum_{j \in \mathcal{J}} v_{i,j} y_{i,j,k}^C \le A_{i,3}^R,\ i \in \mathcal{I} \tag{S-14}$$

The number of facilities, the number of clients/facilities *NC/NF*, capacity for each facility *FC*, as well as maximum running time MaxTime for CFLP are presented in Table S-3[4].

**Table S-3** Brief information on 40 CFLP problems.

| Pro. | *NF/NC* | *FC* | MaxTime(s) |
|---|---|---|---|
| CFLP01-08 | | 10 | |
| CFLP09-16 | | 20 | |
| CFLP17-24 | 100 | 30 | 3 600 |
| CFLP25-32 | | 40 | |
| CFLP33-40 | | 50 | |

1.5 Bin packing problem with conflicts (BPPC)[5]

BPPC is a variant of Bin Pack Problem (BPP), where several items cannot be packed into the same bin. We consider $n$ items and $m$ bins as tasks and resources. The attributes of $R_i$ comprise index $d_i^R$ and capacity $A_{i,1}^R$. The attributes of $T_j$ possess index $d_j^T$, weight $A_{j,1}^T$, and conflict item set $A_{j,2}^T$.

[4] The test suit is from http://old.math.nsc.ru/AP/benchmarks/CFLP/cflp-eng.html.

Concerning the variables in (6), $X_i$, $i \in \mathcal{I}$ is an assignment variable. In addition, the assignment binary matrix $Y^C$ is expressed by (7). Moreover, another attribute variable $Y^U$ is used to determine whether any task is assigned to a resource, where $y_i^U$, $i \in \mathcal{I}$ is calculated by (S-1). The objective is to minimize the number of used bins, which can be denoted by

$$\min \sum_{i \in \mathcal{I}} y_i^U \tag{S-15}$$

The constraint, which ensures each task is executed exactly one time on all resources, can also be denoted as (S-4) and the capacity constraint can be expressed by (S-5). Moreover, the item conflict constraint can be represented by (21), i.e,

$$\sum_{k \in \mathcal{K}_i} y_{i,j',k}^C = 0, \text{ if } \sum_{k \in \mathcal{K}_i} y_{i,j,k}^C = 1, j \in \mathcal{J}, j' \in A_{j,2}^T, i \in \mathcal{I} \tag{S-16}$$

The brief information for 60 BPPC problems, that are randomly selected from a test suit[5], is shown in Table S-4, including the number of items *NT*, the capacity of bins *MC*, and the number of bins *NB*, as well as maximum running time MaxTime(s).

**Table S-4** Brief information on 60 BPPC problems.

| Pro. | *NF* | *MC* | *NB* | MaxTime(s) | Pro. | *NF* | *MC* | *NB* | MaxTime(s) |
|---|---|---|---|---|---|---|---|---|---|
| BPPC1 | 250 | 150 | 150 | 3 600 | BPPC31 | 120 | 1000 | 60 | 360 |
| BPPC2 | 250 | 150 | 150 | 3 600 | BPPC32 | 120 | 1000 | 60 | 360 |
| BPPC3 | 250 | 150 | 150 | 3 600 | BPPC33 | 120 | 1000 | 60 | 360 |
| BPPC4 | 250 | 150 | 150 | 3 600 | BPPC34 | 120 | 1000 | 60 | 360 |
| BPPC5 | 250 | 150 | 150 | 3 600 | BPPC35 | 120 | 1000 | 60 | 360 |
| BPPC6 | 250 | 150 | 220 | 3 600 | BPPC36 | 120 | 1000 | 80 | 360 |
| BPPC7 | 250 | 150 | 220 | 3 600 | BPPC37 | 120 | 1000 | 100 | 360 |
| BPPC8 | 250 | 150 | 220 | 3 600 | BPPC38 | 120 | 1000 | 100 | 360 |
| BPPC9 | 250 | 150 | 220 | 3 600 | BPPC39 | 120 | 1000 | 120 | 360 |
| BPPC10 | 250 | 150 | 240 | 3 600 | BPPC40 | 120 | 1000 | 120 | 360 |
| BPPC11 | 500 | 150 | 320 | 3 600 | BPPC41 | 249 | 1000 | 124 | 1 800 |
| BPPC12 | 500 | 150 | 320 | 3 600 | BPPC42 | 249 | 1000 | 124 | 1 800 |
| BPPC13 | 500 | 150 | 320 | 3 600 | BPPC43 | 249 | 1000 | 124 | 1 800 |
| BPPC14 | 500 | 150 | 320 | 3 600 | BPPC44 | 249 | 1000 | 124 | 1 800 |
| BPPC15 | 500 | 150 | 320 | 3 600 | BPPC45 | 249 | 1000 | 124 | 1 800 |
| BPPC16 | 500 | 150 | 320 | 3 600 | BPPC46 | 249 | 1000 | 166 | 1 800 |
| BPPC17 | 500 | 150 | 370 | 3 600 | BPPC47 | 249 | 1000 | 207 | 1 800 |
| BPPC18 | 500 | 150 | 400 | 3 600 | BPPC48 | 249 | 1000 | 207 | 1 800 |
| BPPC19 | 500 | 150 | 450 | 3 600 | BPPC49 | 249 | 1000 | 249 | 1 800 |
| BPPC20 | 500 | 150 | 500 | 3 600 | BPPC50 | 249 | 1000 | 249 | 1 800 |
| BPPC21 | 60 | 1000 | 30 | 180 | BPPC51 | 510 | 1000 | 250 | 3 600 |
| BPPC22 | 60 | 1000 | 30 | 180 | BPPC52 | 510 | 1000 | 250 | 3 600 |
| BPPC23 | 60 | 1000 | 30 | 180 | BPPC53 | 510 | 1000 | 250 | 3 600 |
| BPPC24 | 60 | 1000 | 30 | 180 | BPPC54 | 510 | 1000 | 250 | 3 600 |
| BPPC25 | 60 | 1000 | 30 | 180 | BPPC55 | 510 | 1000 | 334 | 3 600 |
| BPPC26 | 60 | 1000 | 40 | 180 | BPPC56 | 510 | 1000 | 334 | 3 600 |
| BPPC27 | 60 | 1000 | 50 | 180 | BPPC57 | 510 | 1000 | 417 | 3 600 |
| BPPC28 | 60 | 1000 | 50 | 180 | BPPC58 | 510 | 1000 | 417 | 3 600 |
| BPPC29 | 60 | 1000 | 50 | 180 | BPPC59 | 510 | 1000 | 501 | 3 600 |
| BPPC30 | 60 | 1000 | 60 | 180 | BPPC60 | 510 | 1000 | 501 | 3 600 |

[5] The test suit is from https://site.unibo.it/operations-research/en/research/library-of-codes-and-instances-1.

1.6 Generalized bin packing problem (GBPPI)[6]

GBPPI is also an extension of BPP, where the items can be classified into compulsory and non-compulsory. It should put all compulsory items into bins and determine whether non-compulsory items are selected to maximize the profit. Similarly, we consider $n$ items and $m$ bins as tasks and resources. The attributes of $R_i$ comprises index $d_i^R$, capacity $A_{i,1}^R$, and cost $A_{i,2}^R$. The attributes of $T_j$ include index $d_j^T$, weight $A_{j,1}^T$, and compulsory or non-compulsory index $A_{j,2}^T$ ( $A_{j,2}^T = 0$ denotes $T_j$ is compulsory; otherwise, $T_j$ is non-compulsory). Furthermore, assigning $T_j$ to $R_i$ will generate a profit $p_{i,j}$

Regarding the variables presented in (6), $X_i$, $i \in \mathcal{I}$ is an assignment variable. The attribute variable $Y^C$ is expressed by (7). Moreover, another attribute variable $Y^U$ is used to determine whether any task is assigned to a resource, where $y_i^U$, $i \in \mathcal{I}$ is calculated by (S-1). The objective function is to maximize the total profit, i.e.,

$$\max \sum_{i\in\mathcal{I}} \sum_{j\in\mathcal{J}} \sum_{k\in\mathcal{K}_i} p_{i,j} y_{i,j,k}^C - \sum_{i\in\mathcal{I}} \sum_{j\in\mathcal{J}} \sum_{k\in\mathcal{K}_i} A_{i,2}^R y_i^U \tag{S-17}$$

The capacity constraint for bins can be expressed as (S-5). Additionaly, the constraint that each compulsory task should be put into one of the bins and each non-compulsory task can be placed in at most one bin can be denoted by

$$\begin{cases} \sum_{k\in\mathcal{K}_i} \sum_{i\in\mathcal{I}} y_{i,j,k}^C = 1, \text{ if } A_{j,2}^T = 0, j \in \mathcal{J} \\ \sum_{k\in\mathcal{K}_i} \sum_{i\in\mathcal{I}} y_{i,j,k}^C \le 1, \text{ otherwise}, j \in \mathcal{J} \end{cases}, \tag{S-18}$$

The number of bins *NB*, the number of items *NT*, as well as the maximum running time MaxTime are illustrated in Table S-5, where the problems are randomly selected from a test suit[6]. Moreover, for each problem, 50% of items are randomly set to compulsory items.

**Table S-5** Brief information on 40 GBPPI problems.

| Pro. | *NT* | *NB* | *NI* | MaxTime(s) | Pro. | *NT* | *NB* | *NI* | MaxTime(s) |
|---|---|---|---|---|---|---|---|---|---|
| GBPPI01 | 3 | 33 | 25 | 360 | GBPPI26 | 3 | 33 | 25 | 360 |
| GBPPI02 | 3 | 48 | 25 | 360 | GBPPI27 | 3 | 51 | 25 | 360 |
| GBPPI03 | 3 | 38 | 25 | 360 | GBPPI28 | 3 | 45 | 25 | 360 |
| GBPPI04 | 3 | 65 | 50 | 720 | GBPPI29 | 3 | 68 | 50 | 360 |
| GBPPI05 | 3 | 82 | 50 | 720 | GBPPI30 | 3 | 72 | 50 | 360 |
| GBPPI06 | 3 | 94 | 50 | 720 | GBPPI31 | 3 | 95 | 50 | 360 |
| GBPPI07 | 3 | 130 | 100 | 3 600 | GBPPI32 | 3 | 120 | 100 | 1 800 |
| GBPPI08 | 3 | 154 | 100 | 3 600 | GBPPI33 | 3 | 155 | 100 | 1 800 |
| GBPPI09 | 3 | 190 | 100 | 3 600 | GBPPI34 | 3 | 188 | 100 | 1 800 |
| GBPPI10 | 3 | 248 | 200 | 12 000 | GBPPI35 | 3 | 261 | 200 | 3 600 |
| GBPPI11 | 3 | 310 | 200 | 12 000 | GBPPI36 | 3 | 288 | 200 | 3 600 |
| GBPPI12 | 3 | 372 | 200 | 12 000 | GBPPI37 | 3 | 385 | 200 | 3 600 |
| GBPPI13 | 3 | 627 | 500 | 36 000 | GBPPI38 | 3 | 663 | 500 | 36 000 |
| GBPPI14 | 3 | 758 | 500 | 36 000 | GBPPI39 | 3 | 745 | 500 | 36 000 |
| GBPPI15 | 3 | 949 | 500 | 36 000 | GBPPI40 | 3 | 963 | 500 | 36 000 |
| GBPPI16 | 5 | 70 | 25 | 720 | GBPPI41 | 5 | 65 | 25 | 720 |
| GBPPI17 | 5 | 88 | 25 | 720 | GBPPI42 | 5 | 82 | 25 | 720 |
| GBPPI18 | 5 | 142 | 50 | 3 600 | GBPPI43 | 5 | 156 | 50 | 720 |
| GBPPI19 | 5 | 174 | 50 | 3 600 | GBPPI44 | 5 | 157 | 50 | 720 |
| GBPPI20 | 5 | 299 | 100 | 18 000 | GBPPI45 | 5 | 277 | 100 | 3 600 |

[6] The test suit comes from https://bitbucket.org/ORGroup/gbppi_instances/src/master/.

| | | | | | | | | | |
|---|---|---|---|---|---|---|---|---|---|
| GBPPI21 | 5 | 322 | 100 | 18 000 | GBPPI46 | 5 | 346 | 100 | 3 600 |
| GBPPI22 | 5 | 655 | 200 | 36 000 | GBPPI47 | 5 | 623 | 200 | 36 000 |
| GBPPI23 | 5 | 551 | 200 | 21 000 | GBPPI48 | 5 | 552 | 200 | 12 000 |
| GBPPI24 | 5 | 1398 | 500 | 36 000 | GBPPI49 | 5 | 1664 | 500 | 36 000 |
| GBPPI25 | 5 | 1665 | 500 | 36 000 | GBPPI50 | 5 | 1633 | 500 | 36 000 |

### 1.7 Quadratic multiple knapsack problem (QMKP)[7]

QMKP aims to pack items into knapsacks to maximize profit. Different from the classical knapsack problem, QMKP takes into account the additional profit generated when two items are placed in the same knapsack.

We regard $m$ knapsacks and $n$ items as resources and tasks, respectively. The attributes of $R_i$ have index $d_i^R$ and capacity $A_{i,1}^R$. The attributes of $T_j$ include index $d_j^T$ and weight $A_{j,1}^T$. Moreover, $p_{i,j}$, $i \in \mathcal{I}, j \in \mathcal{J}$ is the profit for assigning $T_j$ to $R_i$ and $cp_{j,j'}$, $j, j' \in \mathcal{J}$ is the additional profit when putting $T_j$ and $T_j$ into the same knapsack.

For the variables shown in (6), $X_i$, $i \in \mathcal{I}$ is an assignment variable. Let $Y^C$ expressed by (7) denote the assignment binary matrix. Moreover, an attribute variable $Y^P$ is used to reflect whether any two tasks are put into the same bins, and $y_{i,j,j'}^P$, $i \in \mathcal{I}, j, j' \in \mathcal{J}$ is calculated as

$$y_{i,j,j'}^P = \begin{cases} 1, \text{ if } \sum_{k \in \mathcal{K}_i} y_{i,j,k}^C = \sum_{k \in \mathcal{K}_i} y_{i,j',k}^C = 1 \\ 0, \text{ otherwise} \end{cases} \quad \text{(S-19)}$$

The objective function is to maximize the total profit, i.e.,

$$\max \sum_{i \in \mathcal{I}} \sum_{j \in \mathcal{J}} p_{i,j} y_{i,j,k}^C + \sum_{i \in \mathcal{I}} \sum_{j \in \mathcal{J}} \sum_{j' \in \mathcal{J}} cp_{j,j'} y_{i,j,j'}^P \quad \text{(S-20)}$$

The constraint, which ensures each task is executed exactly one time on all resources, can be denoted as (S-4) and the capacity constraint can be expressed by (S-5).

The brief information on 45 QMKP problems is presented in Table S-6[7] including the number of items *NT* and the number of knapsacks. Furthermore, the maximum running time MaxTime is set to 360s.

**Table S-6** Brief information on 45 QMKP problems.

| Pro. | *NI* | *NK* | Pro. | *NI* | *NK* | Pro. | *NI* | *NK* |
|---|---|---|---|---|---|---|---|---|
| QMKP01 | 40 | 3 | QMKP16 | 45 | 10 | QMKP31 | 55 | 5 |
| QMKP02 | 40 | 2 | QMKP17 | 45 | 2 | QMKP32 | 55 | 4 |
| QMKP03 | 40 | 4 | QMKP18 | 45 | 3 | QMKP33 | 55 | 4 |
| QMKP04 | 40 | 10 | QMKP19 | 50 | 2 | QMKP34 | 55 | 2 |
| QMKP05 | 40 | 13 | QMKP20 | 50 | 7 | QMKP35 | 55 | 14 |
| QMKP06 | 40 | 2 | QMKP21 | 50 | 8 | QMKP36 | 55 | 2 |
| QMKP07 | 40 | 6 | QMKP22 | 50 | 9 | QMKP37 | 60 | 2 |
| QMKP08 | 40 | 2 | QMKP23 | 50 | 17 | QMKP38 | 60 | 3 |
| QMKP09 | 40 | 12 | QMKP24 | 50 | 6 | QMKP39 | 60 | 15 |
| QMKP10 | 45 | 15 | QMKP25 | 50 | 2 | QMKP40 | 60 | 19 |
| QMKP11 | 45 | 3 | QMKP26 | 50 | 4 | QMKP41 | 60 | 2 |
| QMKP12 | 45 | 2 | QMKP27 | 50 | 4 | QMKP42 | 60 | 6 |
| QMKP13 | 45 | 11 | QMKP28 | 55 | 8 | QMKP43 | 60 | 2 |
| QMKP14 | 45 | 3 | QMKP29 | 55 | 2 | QMKP44 | 60 | 2 |
| QMKP15 | 45 | 9 | QMKP30 | 55 | 5 | QMKP45 | 60 | 4 |

[7] The test suit comes from https://site.unibo.it/operations-research/en/research/library-of-codes-and-instances-1.

1.8 High school timetabling problem (HTS)[8]

HTS involves assigning teachers and classes to time slots. We regard $m$ teachers as resources with a certain number of positions (timeslot). The classes should be assigned to the positions of teachers. Since a teacher may be unoccupied at a timeslot, we employ a virtual task $T_1$ to denote unoccupied status. The virtual task and $nc$ classes will be regarded as tasks and are put in set $T$, where $T_j, j \in \mathcal{J} = \{1,\cdots,n\}, n = nc+1$. The indexes of $R_i$ and $T_j$ are $d_i^R$ and $d_j^T$, respectively. Additionally, $A_{i,k}^M,\ i \in \mathcal{I}, k \in \mathcal{K}_i$ denotes whether resource $R_i$ is available at the $k$ th position. $C_{i,j}^M,\ i \in \mathcal{I}, j \in \mathcal{J}$ is the number of times task $T_j$ needs to be executed on $R_i$ and $P_i^{in},\ i \in \mathcal{I}$ is the set of unavailable positions for $R_i$. Moreover, $D_{i,j}^M,\ i \in \mathcal{I}, j \in \mathcal{J}$ is the maximum daily meeting times and $C_{i,j}^D,\ i \in \mathcal{I}, j \in \mathcal{J}$ is the minimum double lesson number for task $T_j$ on $R_i$. In the problem, a day is divided into 5 periods and we should arrange classes for teachers within 5 working days.

About the variables in (6), $X_i,\ i \in \mathcal{I}$ is a sequence variable and $n_i = 25,\ i \in \mathcal{I}$. We employ $Y^C$ in (7) to denote the assignment binary matrix. Moreover, the number of double lessons extracted from a solution can be denoted by an attribute variable $Y^L$, where $y_{i,j}^L,\ i \in \mathcal{I}, j \in \mathcal{J}$ is the number of double lesson number for task $T_j$ on $R_i$. $y_i^A,\ i \in \mathcal{I}$ is the number of idle periods of $R_i$. $y_i^B,\ i \in \mathcal{I}$ represents the number of days, that are arranged for at least one task from $T_j, j \in \{2,\cdots,n\}$, for $R_i$. In addition, an attribute variable $y_{i,j,r}^F,\ i \in \mathcal{I}, j \in \mathcal{J}, r \in \{1,\cdots,5\}$ reflects the number of meeting times for $R_i$ and $T_j$ on the $r$ th day.

According to reference [8], the objective function can be denoted as:

$$\min \sum_{j\in\mathcal{J}}\sum_{i\in\mathcal{I}} y_{i,j}^L - 3\sum_{i\in\mathcal{I}} y_i^A + 9\sum_{i\in\mathcal{I}} y_i^B \tag{S-21}$$

The constraint that limits the number of times a task executed on a resource can be denoted by:

$$\begin{aligned} &\sum_{k\in\mathcal{K}_i} y_{i,j,k}^C \le C_{i,j}^M,\ j=1, i\in\mathcal{I} \\ &\sum_{k\in\mathcal{K}_i} y_{i,j,k}^C = C_{i,j}^M,\ j>1, i\in\mathcal{I} \end{aligned} \tag{S-22}$$

The unavailable positions in resources should be assigned $T_1$, which can be expressed as

$$y_{i,1,k}^C = 1,\ \text{if } i\in\mathcal{I}, k\in P_i^{in} \tag{S-23}$$

Lastly, the daily meeting times for a resource on a task must not have more than the maximum daily meeting times can be denoted as

$$y_{i,j,r}^F \le D_{i,j}^M,\ i\in\mathcal{I}, j\in\mathcal{J}, r\in\{1,\cdots,5\} \tag{S-24}$$

Table S-7 shows some information on 37 HTS problems[8], involving the number of classes *NC*, the number of teachers *NT*, and the maximum running time MaxTime(s).

**Table S-7** Brief information on 37 HTS problems.

| Pro. | *NC* | *NT* | MaxTime(s) | Pro. | *NC* | *NT* | MaxTime(s) | Pro. | *NC* | *NT* | MaxTime(s) |
|---|---|---|---|---|---|---|---|---|---|---|---|
| HTS01 | 12 | 27 | 3 600 | HTS13 | 3 | 15 | 1 800 | HTS24 | 32 | 75 | 21 000 |
| HTS02 | 12 | 27 | 3 600 | HTS14 | 16 | 34 | 7 200 | HTS25 | 16 | 35 | 7 200 |
| HTS03 | 13 | 31 | 3 600 | HTS15 | 4 | 12 | 3 600 | HTS26 | 10 | 21 | 3 600 |
| HTS04 | 13 | 31 | 3 600 | HTS16 | 8 | 19 | 3 600 | HTS27 | 9 | 20 | 3 600 |
| HTS05 | 9 | 28 | 3 600 | HTS17 | 7 | 21 | 3 600 | HTS28 | 18 | 45 | 3 600 |
| HTS06 | 14 | 29 | 3 600 | HTS18 | 5 | 18 | 3 600 | HTS29 | 18 | 44 | 3 600 |

[8] The test suit comes from https://www.gpea.uem.br/benchmark.html.

| | | | | | | | | | | | |
|---|---|---|---|---|---|---|---|---|---|---|---|
| HTS07 | 20 | 51 | 12 000 | HTS19 | 4 | 15 | 3 600 | HTS30 | 18 | 45 | 3 600 |
| HTS08 | 8 | 30 | 360 | HTS20 | 5 | 18 | 3 600 | HTS31 | 18 | 45 | 3 600 |
| HTS09 | 13 | 34 | 360 | HTS21 | 19 | 37 | 12 000 | HTS32 | 16 | 44 | 3 600 |
| HTS10 | 5 | 17 | 360 | HTS22 | 12 | 31 | 7 200 | HTS33 | 16 | 43 | 3 600 |
| HTS11 | 16 | 35 | 360 | HTS23 | 31 | 62 | 21 000 | HTS34 | 16 | 43 | 3 600 |
| HTS12 | 16 | 38 | 12 000 | | | | | | | | |

1.9 Job shop scheduling problem (JSSP)[9]

The Job Shop Scheduling Problem involves assigning jobs to machines. We treat $m$ machines and $n$ jobs as resources and tasks, separately. The indexes of $R_i$ and $T_j$ are $d_i^R$ and $d_j^T$, respectively. Moreover, $p_{i,j}^T,\ i\in\mathcal{I}, j\in\mathcal{J}$ represents the processing time and $P_i^O,\ i\in\mathcal{I}$ is the processing order for tasks on resource $R_i$, where $p_{i,j}^O\in T, j\in\mathcal{J}$.

For the variables in (6), $X_i,\ i\in\mathcal{I}$ is a sequence variable. The attribute variable $Y^C$ is expressed by (7). Moreover, $y_{i,j,k}^S,\ i\in\mathcal{I}, j\in\mathcal{J}, k\in\mathcal{K}_i$ and $y_{i,j,k}^E,\ i\in\mathcal{I}, j\in\mathcal{J}, k\in\mathcal{K}_i$ respectively denote the start and end process time, which can also be obtained from $X$. The objective is to minimize the makespan and is denoted as

$$\min\max(\{y_{i,j,k}^E \mid i\in\mathcal{I}, j\in\mathcal{J}, k\in\mathcal{K}_i\}) \tag{S-25}$$

The constraint, which ensures each task is executed exactly one time on a resource, can be denoted as

$$\sum_{k\in\mathcal{K}_i} y_{i,j,k}^C = 1,\ \ j\in\mathcal{J}, i\in\mathcal{I}. \tag{S-26}$$

Furthermore, the process order constraint and lock constraint also can be derived accordingly.

The number of jobs *NJ*, the number of machines *NM*, and MaxTime(s) are summarized in Table S-8.

**Table S-8** Brief information on 35 JSSP problems.

| Pro. | *NJ* | *NM* | MaxTime(s) |
|---|---|---|---|
| JSSP01-05 | 15 | 15 | 3 600 |
| JSSP06-10 | 20 | 15 | 3 600 |
| JSSP11-15 | 20 | 20 | 7 200 |
| JSSP16-20 | 30 | 15 | 18 000 |
| JSSP21-25 | 30 | 20 | 18 000 |
| JSSP26-30 | 50 | 15 | 36 000 |
| JSSP31-35 | 50 | 20 | 36 000 |

1.10 Graph coloring problem (GC)[10]

We identify $m$ colors and $n$ nodes as resources and tasks, respectively. The indexes of $R_i$ and $T_j$ are $d_i^R$ and $d_j^T$, separately. Furthermore, $e_{j,j'}, j, j'\in\mathcal{J}$ represents whether $T_j$ and $T_{j'}$ has a connection (when there is a connection between $T_j$ and $T_{j'}$, $e_{j,j'}=1$; otherwise, $e_{j,j'}=0$).

Regarding the variables presented in (6), $X_i,\ i\in\mathcal{I}$ is an assignment variable. Let $Y^C$ expressed by (7) denote the assignment binary matrix. Moreover, another attribute variable $Y^U$ is used to determine whether any task is assigned to a resource, where $y_i^U,\ i\in\mathcal{I}$ is calculated by (S-1). The objective function is to minimize the number of used resources, which can be denoted by

$$\min\sum_{i\in\mathcal{I}} y_i^U \tag{S-27}$$

The constraint ensuring that each task is executed exactly once on all resources is represented

as (S-4). Additionally, the constraint, that the two nodes connected by an edge should be assigned to two different resources, can be calculated as

$$\sum_{k\in\mathcal{K}_i} y_{i,j,k}^{C} + \sum_{k\in\mathcal{K}_i} y_{i,j',k}^{C} \le 1,\ \text{if } e_{j,j'} = 1, i \in \mathcal{I}, j, j' \in \mathcal{J} \tag{S-28}$$

Table S-9 shows the information on 30 GC problems[9] , including the number of nodes *NO*, the number of edges *NE*, the number of colors *NC*, and MaxTime.

**Table S-9** Brief information on 30 GC problems.

| Pro. | *NO* | *NE* | *NC* | MaxTime(s) | Pro. | *NO* | *NE* | *NC* | MaxTime(s) |
|---|---|---|---|---|---|---|---|---|---|
| GC01 | 100 | 2487 | 30 | 1 800 | GC16 | 100 | 2493 | 30 | 1 800 |
| GC02 | 100 | 2487 | 30 | 1 800 | GC17 | 100 | 2503 | 30 | 1 800 |
| GC03 | 100 | 2482 | 30 | 1 800 | GC18 | 100 | 2472 | 30 | 1 800 |
| GC04 | 100 | 2503 | 30 | 1 800 | GC19 | 100 | 2527 | 30 | 1 800 |
| GC05 | 100 | 2450 | 30 | 1 800 | GC20 | 100 | 2420 | 30 | 1 800 |
| GC06 | 100 | 2537 | 30 | 1 800 | GC21 | 300 | 22482 | 80 | 36 000 |
| GC07 | 100 | 2505 | 30 | 1 800 | GC22 | 300 | 22569 | 80 | 36 000 |
| GC08 | 100 | 2479 | 30 | 1 800 | GC23 | 300 | 22393 | 80 | 36 000 |
| GC09 | 100 | 2486 | 30 | 1 800 | GC24 | 300 | 22446 | 80 | 36 000 |
| GC10 | 100 | 2506 | 30 | 1 800 | GC25 | 300 | 22360 | 80 | 36 000 |
| GC11 | 100 | 2467 | 30 | 1 800 | GC26 | 300 | 22601 | 80 | 36 000 |
| GC12 | 100 | 2531 | 30 | 1 800 | GC27 | 300 | 22327 | 80 | 36 000 |
| GC13 | 100 | 2467 | 30 | 1 800 | GC28 | 300 | 22472 | 80 | 36 000 |
| GC14 | 100 | 2524 | 30 | 1 800 | GC29 | 300 | 22520 | 80 | 36 000 |
| GC15 | 100 | 2528 | 30 | 1 800 | GC30 | 300 | 22543 | 80 | 36 000 |

## 2 Algorithm Description and Setting

To instantiate the single-point metaheuristic framework, we adopt Simulated Annealing (SA), Variable Neighborhood Search (VNS), Large Neighborhood Search (LNS), and Tabu Search (TS).

Among them, VNS, TS, and SA utilize Algorithm 3 to generate a new solution. Specifically, VNS generates a single new solution per iteration, whereas TS and SA are set to produce multiple new solutions herein. In contrast, LNS employs Algorithm 4 to destroy and repair the current solution and generate a new solution. When Algorithm 4 cannot improve a current solution within *NIter* iterations, Algorithm 3 will be applied in the following multiple iterations for LNS.

Regarding the acceptance criterion in line 16 of Algorithm 6, VNS and LNS accept $S_{\text{subopt}}$ as $S$ when $S_{\text{subopt}}$ is better than $S$. TS employs a tabu set $\mathcal{T}$ to enhance algorithm diversity by prohibiting the solutions in $\mathcal{T}$ from being selected as the current solution. In each iteration, the best solution that is in $C$ and not in $\mathcal{T}$ will be selected as $S$. When the size of $\mathcal{T}$ reaches its predefined limit, the earliest stored solution in $\mathcal{T}$ will be released. When all solutions in $C$ are included in $\mathcal{T}$ or $S_{\text{subopt}}$ is better than $S_{\text{best}}$, we accept $S_{\text{subopt}}$ as $S$. SA accepts $S_{\text{subopt}}$ as $S$ in terms of the acceptance probability in (S-29).

$$p_{S\leftarrow S_{\text{subopt}}} = \begin{cases} 1, & \text{if } S_{\text{subopt}} \text{ is better than or equal to } S \\ 0, & \text{if } S_{\text{subopt}} \text{ is worse than } S \text{ on constraints} \\ e^{(-|\Delta f|/T_{\text{current}})}, & \text{otherwise} \end{cases} \tag{S-29}$$

where $\Delta f = f(X_{\text{subopt}}, Y_{\text{subopt}}) - f(X,Y)$, $X_{\text{subopt}}$, $Y_{\text{subopt}}$ and $X$, $Y$ denote the variables of $S_{\text{subopt}}$ and $S$, respectively. $T_{\text{current}}$ is the current temperature. At the beginning of optimization, $T_{\text{current}}$

[9] The test suit is from https://people.brunel.ac.uk/~mastjjb/jeb/orlib/colourinfo.html.

is set to initial temperature $T_{\text{initial}}$. If the consecutive iteration time reaches a Markov length $L$, then $T_{\text{current}}$ is updated by $T_{\text{current}} = \gamma T_{\text{current}}$, where $\gamma$ is a cooling rate. $L$ is set in terms of the number of resources and tasks, i.e., $L = \lfloor 0.1mn \rfloor$.

The parameter settings for Simulated Annealing (SA), Variable Neighborhood Search (VNS), Large Neighborhood Search (LNS), Tabu Search (TS), Genetic Algorithm (GA), GUROBI, Routing Solver and CP-SAT from OR-TOOLS, and SCIP are shown in Table S-10. To ensure a consistent evaluation across all algorithms, the presolve processes for SCIP, CP-SAT, and GUROBI are disabled.

**Table S-10** Parameter setting for algorithms.

| Algorithm | Parameter setting |
|---|---|
| SA | Initial Temperature $T_{\text{initial}}$ : 100, Cooling rate $\gamma$ : 0.99, Number of neighborhood solutions $N$ : 5; |
| VNS | Number of neighborhood solutions $N$ : 1 |
| LNS | Number of neighborhood solutions $N$ : 1 |
| TS | Number of neighborhood solutions $N$ : 5; |
| GA | Pop size $popsize$ : 10; Crossover rate $\alpha$ :0.9; Mutation rate $\beta$ :0.2; |
| GUROBI | Presolve: 0; Heuristics: 0; |
| Routing Solver | Default; |
| CP-SAT | Presolve: 0; |
| SCIP | Presolve: 0; |

Except for the parameters in Table S-10, in the neighborhood structure displayed in Algorithm 3, the consecutive iteration $\text{MaxIter1}$ for updating the selection rate of neighborhood structures is set to

$$\text{MaxIter1} = \lfloor 0.1mn \rfloor \tag{S-30}$$

where $m$ is the number of resources and $n$ denotes the number of tasks. Similarly, another consecutive iteration $\text{MaxIter2}$ in Algorithm 6 is set as $\lfloor 0.05mn \rfloor$.

Furthermore, the number of removed tasks $nd$ as presented in Algorithm 4 varies with the scale of problems. At the beginning of optimization, $nd$ is initialized as

$$nd_0 = \min(100, \left\lfloor 0.8\sum_{i\in\mathcal{I}} n_i \right\rfloor) \tag{S-31}$$

where $n_i$ is the number of tasks assigned to resource $R_i$. At the current iteration $iter \in \{1, \cdots \text{MaxIter}\}$, $N^D$ is specified as

$$nd_{iter} = \min(5, \left\lfloor nd_{iter-1} e^{-iter/\text{MaxIter}} \right\rfloor) \tag{S-32}$$

For TS, the size of tabu set $\mathcal{T}$ is also set based on the number of resources and tasks, and dynamically decreases as the number of iterations increases, ranging from an initial value of $\lfloor 0.1mn \rfloor$ to $\lfloor 0.02mn \rfloor$. In addition, the maximum iteration number MaxIter is set to

$$\text{MaxIter} = \begin{cases} 10{,}000, & \text{if } mn \le 10{,}000 \\ 10mn, & \text{if } 10{,}000 < mn \le 20{,}000 \\ 20{,}000, & \text{if } mn > 20{,}000 \end{cases} \tag{S-33}$$

Regarding the five metaheuristic algorithms, the termination condition is triggered under either of the following scenarios: (a) the maximum runtime MaxTime is reached, or (b) the number of consecutive iterations without improvement reaches 2,000. For other algorithms, the termination criteria are defined as (a) the maximum runtime, MaxTime, is reached, or (b) the optimal solution is found.

## 3 Detailed Experimental Results

The subsection will provide the experimental results on 10 problems for the compared

algorithms, including the objective value (obj) and the gap value (gap) over 5 runs. The compared algorithms are GUROBI, OR-TOOLS, SCIO, SA, VNS, LNS, TS, and GA. In these tables, "NaN" indicates that an algorithm was unable to find any feasible solutions within the maximum runtime.

3.1 Multi-depot vehicle routing problem with time windows (MDVRPTW)

Table S-11 displays the experimental results for solving MDVRPTW.

**Table S-11** Experimental results on MDVRPTW test suit.

| Pro. | Metric | Status | GUROBI | OR-TOOLS | SCIP | SA | VNS | LNS | TS | GA |
|---|---|---|---|---|---|---|---|---|---|---|
| MDVRPTW01 | obj | Best | NAN | NAN | NAN | 5.34E+03 | 5.31E+03 | **5.27E+03** | 5.38E+03 | 5.31E+03 |
| | | Mean | NAN | NAN | NAN | 5.85E+03 | **5.71E+03** | 6.02E+03 | 6.09E+03 | 5.72E+03 |
| | gap | Best | NAN | NAN | NAN | 4.00% | 3.49% | **2.83%** | 4.69% | 3.55% |
| | | Mean | NAN | NAN | NAN | 11.98% | **9.84%** | 14.55% | 15.48% | 9.93% |
| MDVRPTW02 | obj | Best | NAN | NAN | NAN | 1.00E+04 | 1.01E+04 | **9.99E+03** | 1.02E+04 | 1.03E+04 |
| | | Mean | NAN | NAN | NAN | **1.01E+04** | 1.04E+04 | 1.06E+04 | 1.03E+04 | 1.06E+04 |
| | gap | Best | NAN | NAN | NAN | 22.19% | 22.96% | **21.93%** | 23.67% | 24.21% |
| | | Mean | NAN | NAN | NAN | **22.88%** | 25.20% | 25.92% | 24.59% | 26.18% |
| MDVRPTW03 | obj | Best | NAN | NAN | NAN | **1.39E+04** | 1.40E+04 | 1.39E+04 | 1.44E+04 | 1.51E+04 |
| | | Mean | NAN | NAN | NAN | **1.41E+04** | 1.47E+04 | 1.46E+04 | 1.49E+04 | 1.52E+04 |
| | gap | Best | NAN | NAN | NAN | **74.31%** | 74.52% | 74.48% | 75.26% | 76.47% |
| | | Mean | NAN | NAN | NAN | **74.67%** | 75.77% | 75.68% | 76.14% | 76.61% |
| MDVRPTW04 | obj | Best | NAN | NAN | NAN | 1.84E+04 | **1.83E+04** | 1.83E+04 | 1.88E+04 | 1.90E+04 |
| | | Mean | NAN | NAN | NAN | 1.86E+04 | **1.85E+04** | 1.85E+04 | 1.91E+04 | 1.98E+04 |
| | gap | Best | NAN | NAN | NAN | 79.37% | **79.26%** | 79.27% | 79.77% | 80.01% |
| | | Mean | NAN | NAN | NAN | 79.58% | **79.54%** | 79.54% | 80.12% | 80.79% |
| MDVRPTW05 | obj | Best | NAN | NAN | NAN | **2.35E+04** | 2.38E+04 | 2.38E+04 | 2.44E+04 | 2.49E+04 |
| | | Mean | NAN | NAN | NAN | **2.38E+04** | 2.39E+04 | 2.41E+04 | 2.48E+04 | 2.60E+04 |
| | gap | Best | NAN | NAN | NAN | **87.86%** | 88.00% | 87.99% | 88.28% | 88.54% |
| | | Mean | NAN | NAN | NAN | **88.03%** | 88.08% | 88.15% | 88.47% | 89.01% |
| MDVRPTW06 | obj | Best | NAN | NAN | NAN | 2.71E+04 | **2.68E+04** | 2.94E+04 | 2.80E+04 | 2.90E+04 |
| | | Mean | NAN | NAN | NAN | 2.77E+04 | **2.71E+04** | 2.98E+04 | 2.86E+04 | 3.61E+04 |
| | gap | Best | NAN | NAN | NAN | NAN | NAN | NAN | NAN | NAN |
| | | Mean | NAN | NAN | NAN | NAN | NAN | NAN | NAN | NAN |
| MDVRPTW07 | obj | Best | NAN | 8.56E+03 | 1.35E+04 | 7.99E+03 | 8.63E+03 | 8.51E+03 | 8.86E+03 | **7.92E+03** |
| | | Mean | NAN | 8.64E+03 | 1.35E+04 | **8.49E+03** | 8.68E+03 | 8.56E+03 | 9.03E+03 | 8.66E+03 |
| | gap | Best | NAN | 28.20% | 54.63% | 23.06% | 28.80% | 27.84% | 30.66% | **22.38%** |
| | | Mean | NAN | 28.88% | 54.63% | **27.57%** | 29.22% | 28.22% | 31.93% | 28.92% |
| MDVRPTW08 | obj | Best | NAN | NAN | NAN | 1.40E+04 | **1.37E+04** | 1.44E+04 | 1.48E+04 | 1.45E+04 |
| | | Mean | NAN | NAN | NAN | 1.43E+04 | **1.43E+04** | 1.45E+04 | 1.49E+04 | 1.51E+04 |
| | gap | Best | NAN | NAN | NAN | 66.51% | **65.78%** | 67.42% | 68.27% | 67.59% |
| | | Mean | NAN | NAN | NAN | 67.24% | **67.03%** | 67.54% | 68.56% | 68.96% |
| MDVRPTW09 | obj | Best | NAN | **1.93E+04** | NAN | 1.98E+04 | 1.95E+04 | 1.95E+04 | 2.02E+04 | 2.08E+04 |
| | | Mean | NAN | **1.97E+04** | NAN | 1.99E+04 | 1.99E+04 | 1.99E+04 | 2.04E+04 | 2.11E+04 |
| | gap | Best | NAN | **79.95%** | NAN | 80.50% | 80.22% | 80.17% | 80.89% | 81.42% |

| | | | | | | | | | | |
|---|---|---|---|---|---|---|---|---|---|---|
| | | Mean | NAN | **80.36%** | NAN | 80.63% | 80.64% | 80.59% | 81.04% | 81.70% |
| MDVR PTW10 | obj | Best | NAN | NAN | NAN | 2.88E+04 | 2.89E+04 | **2.83E+04** | 2.94E+04 | 3.23E+04 |
| | | Mean | NAN | NAN | NAN | 2.90E+04 | 2.92E+04 | **2.88E+04** | 2.98E+04 | 3.38E+04 |
| | gap | Best | NAN | NAN | NAN | 88.41% | 88.47% | **88.22%** | 88.66% | 89.67% |
| | | Mean | NAN | NAN | NAN | 88.48% | 88.56% | **88.41%** | 88.81% | 90.13% |
| MDVR PTW11 | obj | Best | NAN | NAN | NAN | **5.03E+03** | 5.15E+03 | 5.08E+03 | 5.08E+03 | 5.11E+03 |
| | | Mean | NAN | NAN | NAN | **5.10E+03** | 5.19E+03 | 5.21E+03 | 5.24E+03 | 5.20E+03 |
| | gap | Best | NAN | NAN | NAN | **4.23%** | 9.96% | 5.06% | 5.13% | 5.74% |
| | | Mean | NAN | NAN | NAN | **5.40%** | 7.09% | 7.40% | 7.93% | 7.30% |
| MDVR PTW12 | obj | Best | NAN | NAN | NAN | 8.79E+03 | 8.96E+03 | **8.64E+03** | 9.39E+03 | 8.94E+03 |
| | | Mean | NAN | NAN | NAN | 9.01E+03 | 9.43E+03 | **8.79E+03** | 9.86E+03 | 9.39E+03 |
| | gap | Best | NAN | NAN | NAN | 8.24% | 9.96% | **6.66%** | 14.12% | 9.78% |
| | | Mean | NAN | NAN | NAN | 10.44% | 14.28% | **8.20%** | 18.15% | 14.01% |
| MDVR PTW13 | obj | Best | NAN | NAN | NAN | 1.34E+04 | 1.37E+04 | **1.24E+04** | 1.41E+04 | 1.30E+04 |
| | | Mean | NAN | NAN | NAN | 1.36E+04 | 9.43E+03 | **1.31E+04** | 1.45E+04 | 1.36E+04 |
| | gap | Best | NAN | NAN | NAN | 76.19% | 76.79% | **74.36%** | 77.47% | 75.55% |
| | | Mean | NAN | NAN | NAN | 76.61% | 77.20% | **75.69%** | 78.01% | 76.60% |
| MDVR PTW14 | obj | Best | NAN | NAN | NAN | 1.70E+04 | 1.70E+04 | **1.68E+04** | 1.74E+04 | 1.74E+04 |
| | | Mean | NAN | NAN | NAN | 1.74E+04 | 1.40E+04 | **1.70E+04** | 1.80E+04 | 1.76E+04 |
| | gap | Best | NAN | NAN | NAN | 85.83% | 85.82% | **85.64%** | 86.13% | 86.14% |
| | | Mean | NAN | NAN | NAN | 86.11% | 77.20% | **85.81%** | 86.58% | 86.32% |
| MDVR PTW15 | obj | Best | NAN | NAN | NAN | 2.28E+04 | 2.30E+04 | **2.21E+04** | 2.37E+04 | 2.35E+04 |
| | | Mean | NAN | NAN | NAN | 2.30E+04 | 1.74E+04 | **2.28E+04** | 2.43E+04 | 2.48E+04 |
| | gap | Best | NAN | NAN | NAN | NAN | NAN | NAN | NAN | NAN |
| | | Mean | NAN | NAN | NAN | NAN | NAN | NAN | NAN | NAN |
| MDVR PTW16 | obj | Best | NAN | **2.54E+04** | NAN | 2.63E+04 | 2.66E+04 | 2.62E+04 | 2.75E+04 | 2.73E+04 |
| | | Mean | NAN | **2.55E+04** | NAN | 2.69E+04 | 2.33E+04 | 2.68E+04 | 2.77E+04 | 2.75E+04 |
| | gap | Best | NAN | **NAN** | NAN | NAN | NAN | NAN | NAN | NAN |
| | | Mean | NAN | **NAN** | NAN | NAN | NAN | NAN | NAN | NAN |
| MDVR PTW17 | obj | Best | NAN | **7.28E+03** | NAN | 7.38E+03 | 7.43E+03 | 7.32E+03 | 7.68E+03 | 7.50E+03 |
| | | Mean | NAN | **7.31E+03** | NAN | 7.53E+03 | 2.70E+04 | 7.46E+03 | 7.81E+03 | 7.60E+03 |
| | gap | Best | NAN | **NAN** | NAN | NAN | NAN | NAN | NAN | NAN |
| | | Mean | NAN | **NAN** | NAN | NAN | NAN | NAN | NAN | NAN |
| MDVR PTW18 | obj | Best | NAN | NAN | NAN | 1.36E+04 | 1.37E+04 | **1.32E+04** | 1.42E+04 | 1.37E+04 |
| | | Mean | NAN | NAN | NAN | 1.39E+04 | 7.69E+03 | **1.33E+04** | 1.47E+04 | 1.40E+04 |
| | gap | Best | NAN | NAN | NAN | NAN | NAN | NAN | NAN | NAN |
| | | Mean | NAN | NAN | NAN | NAN | NAN | NAN | NAN | NAN |
| MDVR PTW19 | obj | Best | NAN | **1.87E+04** | NAN | 1.91E+04 | 1.91E+04 | 1.88E+04 | 1.95E+04 | 1.92E+04 |
| | | Mean | NAN | **1.88E+04** | NAN | 1.93E+04 | 1.39E+04 | 1.91E+04 | 1.99E+04 | 1.96E+04 |
| | gap | Best | NAN | **NAN** | NAN | NAN | NAN | NAN | NAN | NAN |
| | | Mean | NAN | **NAN** | NAN | NAN | NAN | NAN | NAN | NAN |
| MDVR PTW20 | obj | Best | NAN | NAN | NAN | 2.82E+04 | **2.81E+04** | **2.81E+04** | 2.86E+04 | 2.98E+04 |
| | | Mean | NAN | NAN | NAN | 2.87E+04 | 2.90E+04 | **2.84E+04** | 2.94E+04 | 3.17E+04 |

| | | | | | | | | | |
|---|---|---|---|---|---|---|---|---|---|
| gap | Best | NAN | NAN | NAN | NAN | NAN | NAN | NAN | NAN |
| | Mean | NAN | NAN | NAN | NAN | NAN | NAN | NAN | NAN |

3.2 Vehicle routing problem with pickup and delivery (VRPPD)

The relevant experimental results on VRPPD are presented in Table S-12.

**Table S-12** Experimental results on VRPPD test suit.

| Pro. | Metric | Status | GUROBI | OR-TOOLS | SCIP | SA | VNS | LNS | TS | GA |
|---|---|---|---|---|---|---|---|---|---|---|
| VRPPD01 | obj | Best | NAN | **1.12E+03** | NAN | 1.67E+03 | 1.71E+03 | 1.65E+03 | 1.85E+03 | 1.73E+03 |
| | | Mean | NAN | **1.13E+03** | NAN | 1.76E+03 | 1.76E+03 | 1.65E+03 | 1.97E+03 | 1.76E+03 |
| | gap | Best | NAN | **10.44%** | NAN | 39.76% | 41.20% | 39.05% | 45.68% | 42.16% |
| | | Mean | NAN | **11.59%** | NAN | 42.95% | 43.05% | 39.18% | 48.94% | 43.10% |
| VRPPD02 | obj | Best | NAN | **1.12E+03** | NAN | 1.84E+03 | 1.84E+03 | 1.74E+03 | 1.82E+03 | 1.85E+03 |
| | | Mean | NAN | **1.13E+03** | NAN | 1.88E+03 | 1.90E+03 | 1.75E+03 | 1.99E+03 | 1.90E+03 |
| | gap | Best | NAN | **10.02%** | NAN | 44.91% | 45.02% | 41.83% | 44.52% | 45.27% |
| | | Mean | NAN | **10.75%** | NAN | 46.14% | 46.81% | 42.20% | 48.97% | 46.74% |
| VRPPD03 | obj | Best | NAN | **1.19E+03** | NAN | 2.33E+03 | 2.25E+03 | 2.11E+03 | 2.35E+03 | 2.27E+03 |
| | | Mean | NAN | **1.19E+03** | NAN | 2.38E+03 | 2.32E+03 | 2.16E+03 | 2.50E+03 | 2.36E+03 |
| | gap | Best | NAN | **71.21%** | NAN | 85.29% | 84.72% | 83.72% | 85.43% | 84.87% |
| | | Mean | NAN | **71.21%** | NAN | 85.60% | 85.18% | 84.10% | 86.24% | 85.44% |
| VRPPD04 | obj | Best | NAN | **6.03E+02** | NAN | 1.67E+03 | 1.67E+03 | 1.65E+03 | 1.74E+03 | 1.67E+03 |
| | | Mean | NAN | **6.16E+02** | NAN | 1.69E+03 | 1.72E+03 | 1.66E+03 | 1.83E+03 | 1.71E+03 |
| | gap | Best | NAN | **44.71%** | NAN | 80.01% | 80.04% | 79.79% | 80.86% | 80.05% |
| | | Mean | NAN | **45.85%** | NAN | 80.26% | 80.60% | 79.88% | 81.76% | 80.50% |
| VRPPD05 | obj | Best | NAN | **1.12E+03** | NAN | 2.18E+03 | 2.18E+03 | 2.09E+03 | 2.35E+03 | 2.12E+03 |
| | | Mean | NAN | **1.12E+03** | NAN | 2.21E+03 | 2.24E+03 | 2.12E+03 | 2.45E+03 | 2.19E+03 |
| | gap | Best | NAN | **31.66%** | NAN | 64.97% | 65.02% | 63.47% | 67.59% | 64.00% |
| | | Mean | NAN | **31.66%** | NAN | 65.56% | 65.95% | 64.11% | 68.85% | 65.25% |
| VRPPD06 | obj | Best | NAN | **1.26E+03** | NAN | 2.34E+03 | 2.34E+03 | 2.30E+03 | 2.46E+03 | 2.28E+03 |
| | | Mean | NAN | **1.26E+03** | NAN | 2.38E+03 | 2.40E+03 | 2.32E+03 | 2.58E+03 | 2.38E+03 |
| | gap | Best | NAN | **37.72%** | NAN | 66.39% | 66.47% | 65.80% | 68.05% | 65.62% |
| | | Mean | NAN | **37.72%** | NAN | 67.03% | 67.32% | 66.10% | 69.54% | 67.04% |
| VRPPD07 | obj | Best | NAN | **1.42E+03** | NAN | 2.65E+03 | 2.72E+03 | 2.63E+03 | 2.89E+03 | 2.71E+03 |
| | | Mean | NAN | **1.42E+03** | NAN | 2.74E+03 | 2.75E+03 | 2.65E+03 | 2.98E+03 | 2.79E+03 |
| | gap | Best | NAN | **60.59%** | NAN | 78.94% | 79.42% | 78.75% | 80.65% | 79.37% |
| | | Mean | NAN | **60.59%** | NAN | 79.58% | 79.70% | 78.90% | 81.21% | 79.92% |
| VRPPD08 | obj | Best | NAN | **1.11E+03** | NAN | 2.59E+03 | 2.53E+03 | 2.48E+03 | 2.94E+03 | 2.62E+03 |
| | | Mean | NAN | **1.15E+03** | NAN | 2.69E+03 | 2.60E+03 | 2.51E+03 | 3.02E+03 | 2.67E+03 |
| | gap | Best | NAN | **25.35%** | NAN | 68.05% | 67.26% | 66.61% | 71.78% | 68.32% |
| | | Mean | NAN | **27.60%** | NAN | 69.14% | 68.16% | 67.01% | 72.53% | 68.99% |
| VRPPD09 | obj | Best | NAN | **1.12E+03** | NAN | 2.01E+03 | 2.04E+03 | 1.94E+03 | 2.30E+03 | 1.98E+03 |
| | | Mean | NAN | **1.12E+03** | NAN | 2.05E+03 | 2.11E+03 | 1.95E+03 | 2.38E+03 | 2.08E+03 |
| | gap | Best | NAN | **28.13%** | NAN | 59.89% | 60.46% | 58.50% | 64.98% | 59.27% |
| | | Mean | NAN | **28.13%** | NAN | 60.76% | 61.76% | 58.77% | 66.08% | 61.20% |
| VRPPD10 | obj | Best | NAN | **1.12E+03** | NAN | 2.21E+03 | 2.18E+03 | 2.09E+03 | 2.35E+03 | 2.19E+03 |
| | | Mean | NAN | **1.14E+03** | NAN | 2.25E+03 | 2.22E+03 | 2.11E+03 | 2.55E+03 | 2.25E+03 |
| | gap | Best | NAN | **25.62%** | NAN | 62.38% | 61.83% | 60.07% | 64.59% | 61.92% |
| | | Mean | NAN | **27.09%** | NAN | 63.01% | 62.41% | 60.53% | 67.27% | 63.00% |

| Pro. | Metric | Status | GUROBI | OR-TOOLS | SCIP | SA | VNS | LNS | TS | GA |
|---|---|---|---|---|---|---|---|---|---|---|
| VRPPD11 | obj | Best | NAN | **6.92E+02** | NAN | 1.62E+03 | 1.66E+03 | 1.59E+03 | 1.78E+03 | 1.62E+03 |
| | | Mean | NAN | **7.65E+02** | NAN | 1.67E+03 | 1.69E+03 | 1.60E+03 | 1.92E+03 | 1.67E+03 |
| | gap | Best | NAN | **4.40%** | NAN | 59.28% | 60.09% | 58.42% | 62.80% | 59.18% |
| | | Mean | NAN | **13.23%** | NAN | 60.36% | 60.94% | 58.63% | 65.38% | 60.30% |
| VRPPD12 | obj | Best | NAN | **8.72E+02** | NAN | 2.12E+03 | 2.06E+03 | 2.03E+03 | 2.37E+03 | 2.11E+03 |
| | | Mean | NAN | **8.92E+02** | NAN | 2.17E+03 | 2.13E+03 | 2.04E+03 | 2.40E+03 | 2.19E+03 |
| | gap | Best | NAN | **60.02%** | NAN | 83.52% | 83.07% | 82.81% | 85.31% | 83.48% |
| | | Mean | NAN | **60.91%** | NAN | 83.93% | 83.59% | 82.90% | 85.44% | 84.08% |
| VRPPD13 | obj | Best | NAN | **4.24E+02** | NAN | 1.77E+03 | 1.80E+03 | 1.76E+03 | 1.86E+03 | 1.83E+03 |
| | | Mean | NAN | **4.34E+02** | NAN | 1.88E+03 | 1.83E+03 | 1.77E+03 | 2.04E+03 | 1.88E+03 |
| | gap | Best | NAN | **11.75%** | NAN | 71.07% | 71.59% | 70.86% | 72.53% | 72.10% |
| | | Mean | NAN | **18.02%** | NAN | 72.79% | 72.07% | 71.01% | 74.81% | 72.76% |
| VRPPD14 | obj | Best | NAN | **5.65E+02** | NAN | 1.70E+03 | 1.70E+03 | 1.64E+03 | 1.86E+03 | 1.71E+03 |
| | | Mean | NAN | **5.65E+02** | NAN | 1.71E+03 | 1.75E+03 | 1.65E+03 | 1.93E+03 | 1.73E+03 |
| | gap | Best | NAN | **33.46%** | NAN | 77.90% | 77.91% | 77.01% | 79.79% | 77.97% |
| | | Mean | NAN | **33.46%** | NAN | 78.01% | 78.49% | 77.24% | 80.56% | 78.28% |
| VRPPD15 | obj | Best | NAN | **6.64E+02** | NAN | 1.80E+03 | 1.80E+03 | 1.76E+03 | 1.86E+03 | 1.78E+03 |
| | | Mean | NAN | **6.81E+02** | NAN | 1.83E+03 | 1.83E+03 | 1.77E+03 | 2.00E+03 | 1.84E+03 |
| | gap | Best | NAN | **28.04%** | NAN | 73.45% | 73.39% | 72.88% | 74.27% | 73.17% |
| | | Mean | NAN | **29.73%** | NAN | 73.86% | 73.94% | 73.01% | 76.01% | 73.98% |
| VRPPD16 | obj | Best | NAN | **6.07E+02** | NAN | 1.22E+03 | 1.20E+03 | 1.18E+03 | 1.25E+03 | 1.19E+03 |
| | | Mean | NAN | **6.11E+02** | NAN | 1.22E+03 | 1.23E+03 | 1.19E+03 | 1.35E+03 | 1.21E+03 |
| | gap | Best | NAN | **27.15%** | NAN | 63.74% | 63.00% | 62.45% | 64.76% | 62.75% |
| | | Mean | NAN | **27.65%** | NAN | 63.79% | 63.99% | 62.96% | 67.17% | 63.46% |
| VRPPD17 | obj | Best | NAN | **5.65E+02** | NAN | 1.45E+03 | 1.46E+03 | 1.41E+03 | 1.57E+03 | 1.45E+03 |
| | | Mean | NAN | **5.71E+02** | NAN | 1.47E+03 | 1.49E+03 | 1.43E+03 | 1.67E+03 | 1.49E+03 |
| | gap | Best | NAN | **19.74%** | NAN | 68.78% | 68.91% | 67.93% | 71.14% | 68.70% |
| | | Mean | NAN | **20.55%** | NAN | 69.15% | 69.51% | 68.27% | 72.83% | 69.60% |
| VRPPD18 | obj | Best | NAN | **6.17E+02** | NAN | 1.99E+03 | 1.94E+03 | 1.93E+03 | 2.06E+03 | 1.98E+03 |
| | | Mean | NAN | **6.57E+02** | NAN | 2.03E+03 | 2.01E+03 | 1.95E+03 | 2.16E+03 | 2.04E+03 |
| | gap | Best | NAN | **51.59%** | NAN | 85.00% | 84.57% | 84.51% | 85.53% | 84.93% |
| | | Mean | NAN | **54.46%** | NAN | 85.27% | 85.17% | 84.66% | 86.18% | 85.38% |
| VRPPD19 | obj | Best | NAN | **5.38E+02** | NAN | 1.41E+03 | 1.41E+03 | 1.37E+03 | 1.49E+03 | 1.38E+03 |
| | | Mean | NAN | **5.74E+02** | NAN | 1.45E+03 | 1.46E+03 | 1.42E+03 | 1.59E+03 | 1.43E+03 |
| | gap | Best | NAN | **32.55%** | NAN | 74.28% | 74.33% | 73.59% | 75.69% | 73.69% |
| | | Mean | NAN | **36.41%** | NAN | 74.96% | 75.18% | 74.38% | 77.11% | 74.60% |
| VRPPD20 | obj | Best | NAN | **5.73E+02** | NAN | 1.93E+03 | 1.91E+03 | 1.88E+03 | 2.04E+03 | 1.93E+03 |
| | | Mean | NAN | **5.94E+02** | NAN | 1.96E+03 | 1.96E+03 | 1.88E+03 | 2.11E+03 | 1.98E+03 |
| | gap | Best | NAN | **46.60%** | NAN | 84.15% | 83.97% | 83.71% | 84.99% | 84.13% |
| | | Mean | NAN | **48.42%** | NAN | 84.35% | 84.39% | 83.76% | 85.48% | 84.53% |
| VRPPD21 | obj | Best | NAN | **6.94E+02** | NAN | 1.60E+03 | 1.55E+03 | 1.53E+03 | 1.72E+03 | 1.55E+03 |
| | | Mean | NAN | **7.08E+02** | NAN | 1.63E+03 | 1.61E+03 | 1.55E+03 | 1.77E+03 | 1.58E+03 |
| | gap | Best | NAN | **46.64%** | NAN | 76.87% | 76.13% | 75.74% | 78.50% | 76.16% |
| | | Mean | NAN | **47.67%** | NAN | 77.24% | 77.02% | 76.06% | 79.10% | 76.52% |
| VRPPD22 | obj | Best | NAN | **6.40E+02** | NAN | 1.47E+03 | 1.44E+03 | 1.35E+03 | 1.56E+03 | 1.43E+03 |
| | | Mean | NAN | **6.40E+02** | NAN | 1.51E+03 | 1.48E+03 | 1.37E+03 | 1.72E+03 | 1.51E+03 |
| | gap | Best | NAN | **12.69%** | NAN | 62.01% | 61.32% | 58.59% | 64.26% | 61.05% |

| Pro. | Metric | Status | GUROBI | OR-TOOLS | SCIP | SA | VNS | LNS | TS | GA |
|---|---|---|---|---|---|---|---|---|---|---|
| | | Mean | NAN | **12.69%** | NAN | 62.92% | 62.29% | 59.31% | 67.46% | 62.87% |
| VRPPD23 | obj | Best | NAN | **7.10E+02** | NAN | 1.90E+03 | 1.94E+03 | 1.89E+03 | 2.06E+03 | 1.98E+03 |
| | | Mean | NAN | **7.20E+02** | NAN | 1.96E+03 | 2.02E+03 | 1.90E+03 | 2.20E+03 | 2.04E+03 |
| | gap | Best | NAN | **55.24%** | NAN | 83.24% | 83.59% | 83.16% | 84.56% | 83.96% |
| | | Mean | NAN | **55.83%** | NAN | 83.78% | 84.24% | 83.27% | 85.53% | 84.40% |
| VRPPD24 | obj | Best | NAN | **4.41E+02** | NAN | 1.22E+03 | 1.23E+03 | 1.17E+03 | 1.29E+03 | 1.19E+03 |
| | | Mean | NAN | **4.45E+02** | NAN | 1.24E+03 | 1.25E+03 | 1.19E+03 | 1.35E+03 | 1.22E+03 |
| | gap | Best | NAN | **26.61%** | NAN | 73.53% | 73.69% | 72.40% | 74.98% | 72.81% |
| | | Mean | NAN | **27.33%** | NAN | 73.85% | 74.07% | 72.82% | 75.97% | 73.36% |
| VRPPD25 | obj | Best | NAN | **4.60E+02** | NAN | 1.39E+03 | 1.42E+03 | 1.37E+03 | 1.49E+03 | 1.44E+03 |
| | | Mean | NAN | **4.68E+02** | NAN | 1.43E+03 | 1.45E+03 | 1.39E+03 | 1.57E+03 | 1.46E+03 |
| | gap | Best | NAN | **19.95%** | NAN | 73.57% | 74.13% | 73.19% | 75.28% | 74.48% |
| | | Mean | NAN | **21.29%** | NAN | 74.20% | 74.67% | 73.43% | 76.46% | 74.73% |
| VRPPD26 | obj | Best | NAN | **5.42E+02** | NAN | 1.90E+03 | 1.89E+03 | 1.88E+03 | 1.91E+03 | 1.90E+03 |
| | | Mean | NAN | **5.43E+02** | NAN | 1.92E+03 | 1.93E+03 | 1.89E+03 | 2.01E+03 | 1.93E+03 |
| | gap | Best | NAN | **16.41%** | NAN | 76.14% | 76.09% | 75.93% | 76.29% | 76.13% |
| | | Mean | NAN | **16.54%** | NAN | 76.38% | 76.56% | 76.03% | 77.39% | 76.58% |
| VRPPD27 | obj | Best | NAN | **8.97E+02** | NAN | 1.92E+03 | 1.94E+03 | 1.85E+03 | 2.01E+03 | 1.93E+03 |
| | | Mean | NAN | **9.39E+02** | NAN | 1.99E+03 | 2.00E+03 | 1.90E+03 | 2.16E+03 | 1.97E+03 |
| | gap | Best | NAN | **41.98%** | NAN | 72.91% | 73.18% | 71.91% | 74.12% | 72.99% |
| | | Mean | NAN | **44.50%** | NAN | 73.83% | 73.92% | 72.59% | 75.80% | 73.55% |
| VRPPD28 | obj | Best | NAN | **9.56E+02** | NAN | 2.44E+03 | 2.45E+03 | 2.38E+03 | 2.63E+03 | 2.46E+03 |
| | | Mean | NAN | **1.02E+03** | NAN | 2.47E+03 | 2.49E+03 | 2.41E+03 | 2.71E+03 | 2.50E+03 |
| | gap | Best | NAN | **52.35%** | NAN | 81.31% | 81.38% | 80.84% | 82.65% | 81.49% |
| | | Mean | NAN | **55.11%** | NAN | 81.57% | 81.70% | 81.08% | 83.21% | 81.76% |
| VRPPD29 | obj | Best | NAN | **9.11E+02** | NAN | 1.94E+03 | 1.91E+03 | 1.86E+03 | 2.17E+03 | 1.93E+03 |
| | | Mean | NAN | **9.25E+02** | NAN | 1.97E+03 | 1.96E+03 | 1.87E+03 | 2.23E+03 | 2.01E+03 |
| | gap | Best | NAN | **44.34%** | NAN | 73.85% | 73.40% | 72.78% | 76.65% | 73.70% |
| | | Mean | NAN | **45.15%** | NAN | 74.30% | 74.08% | 72.94% | 77.25% | 74.71% |
| VRPPD30 | obj | Best | NAN | **1.04E+03** | NAN | 2.39E+03 | 2.40E+03 | 2.33E+03 | 2.57E+03 | 2.40E+03 |
| | | Mean | NAN | **1.07E+03** | NAN | 2.46E+03 | 2.45E+03 | 2.34E+03 | 2.64E+03 | 2.46E+03 |
| | gap | Best | NAN | **51.20%** | NAN | 78.80% | 78.87% | 78.21% | 80.27% | 78.90% |
| | | Mean | NAN | **52.64%** | NAN | 79.40% | 79.26% | 78.37% | 80.80% | 79.40% |

### 3.3 Generalized assignment problem (GAP)

Table S-13 provides the experimental results for GAP.

**Table S-13** Experimental results on GAP test suit.

| Pro. | Metric | Status | GUROBI | OR-TOOLS | SCIP | SA | VNS | LNS | TS | GA |
|---|---|---|---|---|---|---|---|---|---|---|
| GAP01 | obj | Best | **1.70E+03** | **1.70E+03** | **1.70E+03** | 1.70E+03 | **1.70E+03** | **1.70E+03** | 1.70E+03 | **1.70E+03** |
| | | Mean | **1.70E+03** | **1.70E+03** | **1.70E+03** | 1.70E+03 | 1.70E+03 | **1.70E+03** | 1.70E+03 | 1.70E+03 |
| | gap | Best | **0.00%** | **0.00%** | **0.00%** | 0.12% | **0.00%** | **0.00%** | 0.24% | **0.00%** |
| | | Mean | **0.00%** | **0.00%** | **0.00%** | 0.22% | 0.05% | **0.00%** | 0.28% | 0.15% |
| GAP02 | obj | Best | **3.24E+03** | **3.24E+03** | **3.24E+03** | **3.24E+03** | **3.24E+03** | **3.24E+03** | **3.24E+03** | **3.24E+03** |
| | | Mean | **3.24E+03** | **3.24E+03** | **3.24E+03** | **3.24E+03** | **3.24E+03** | **3.24E+03** | 3.24E+03 | 3.24E+03 |
| | gap | Best | **0.00%** | **0.00%** | **0.00%** | **0.00%** | **0.00%** | **0.00%** | **0.00%** | **0.00%** |
| | | Mean | **0.00%** | **0.00%** | **0.00%** | **0.00%** | **0.00%** | **0.00%** | 0.02% | 0.02% |

| Pro. | Metric | Status | GUROBI | OR-TOOLS | SCIP | SA | VNS | LNS | TS | GA |
|---|---|---|---|---|---|---|---|---|---|---|
| GAP03 | obj | Best | **1.36E+03** | **1.36E+03** | **1.36E+03** | 1.36E+03 | **1.36E+03** | **1.36E+03** | **1.36E+03** | **1.36E+03** |
| | | Mean | **1.36E+03** | **1.36E+03** | **1.36E+03** | 1.36E+03 | 1.36E+03 | **1.36E+03** | 1.36E+03 | 1.36E+03 |
| | gap | Best | **0.00%** | **0.00%** | **0.00%** | 0.07% | **0.00%** | **0.00%** | **0.00%** | **0.00%** |
| | | Mean | **0.00%** | **0.00%** | **0.00%** | 0.19% | 0.06% | **0.00%** | 0.12% | 0.12% |
| GAP04 | obj | Best | **2.62E+03** | **2.62E+03** | **2.62E+03** | 2.62E+03 | 2.62E+03 | **2.62E+03** | 2.63E+03 | **2.62E+03** |
| | | Mean | **2.62E+03** | **2.62E+03** | **2.62E+03** | 2.63E+03 | 2.63E+03 | **2.62E+03** | 2.63E+03 | 2.63E+03 |
| | gap | Best | **0.00%** | **0.00%** | **0.00%** | 0.04% | 0.04% | **0.00%** | 0.15% | **0.00%** |
| | | Mean | **0.00%** | **0.00%** | **0.00%** | 0.12% | 0.15% | **0.00%** | 0.19% | 0.13% |
| GAP05 | obj | Best | **1.16E+03** | **1.16E+03** | **1.16E+03** | **1.16E+03** | **1.16E+03** | **1.16E+03** | **1.16E+03** | **1.16E+03** |
| | | Mean | **1.16E+03** | **1.16E+03** | **1.16E+03** | **1.16E+03** | **1.16E+03** | **1.16E+03** | 1.16E+03 | 1.16E+03 |
| | gap | Best | **0.00%** | **0.00%** | **0.00%** | **0.00%** | **0.00%** | **0.00%** | **0.00%** | **0.00%** |
| | | Mean | **0.00%** | **0.00%** | **0.00%** | **0.00%** | **0.00%** | **0.00%** | 0.12% | 0.03% |
| GAP06 | obj | Best | **2.34E+03** | **2.34E+03** | **2.34E+03** | **2.34E+03** | **2.34E+03** | **2.34E+03** | **2.34E+03** | 2.34E+03 |
| | | Mean | **2.34E+03** | **2.34E+03** | **2.34E+03** | 2.34E+03 | **2.34E+03** | **2.34E+03** | 2.34E+03 | 2.34E+03 |
| | gap | Best | **0.00%** | **0.00%** | **0.00%** | **0.00%** | **0.00%** | **0.00%** | **0.00%** | 0.04% |
| | | Mean | **0.00%** | **0.00%** | **0.00%** | 0.14% | **0.00%** | **0.00%** | 0.09% | 0.16% |
| GAP07 | obj | Best | **1.84E+03** | **1.84E+03** | **1.84E+03** | 2.01E+03 | 1.92E+03 | 1.93E+03 | 2.01E+03 | 1.89E+03 |
| | | Mean | **1.84E+03** | **1.84E+03** | **1.84E+03** | 2.04E+03 | 2.00E+03 | 1.93E+03 | 2.05E+03 | 1.92E+03 |
| | gap | Best | **0.00%** | **0.00%** | **0.00%** | 8.35% | 4.21% | 4.46% | 8.31% | 2.44% |
| | | Mean | **0.00%** | **0.00%** | **0.00%** | 9.49% | 7.79% | 4.64% | 10.08% | 3.94% |
| GAP08 | obj | Best | **3.55E+03** | **3.55E+03** | **3.55E+03** | 3.77E+03 | 3.63E+03 | 3.67E+03 | 3.77E+03 | 3.71E+03 |
| | | Mean | **3.55E+03** | **3.55E+03** | **3.55E+03** | 3.84E+03 | 3.71E+03 | 3.71E+03 | 3.82E+03 | 3.77E+03 |
| | gap | Best | **0.00%** | **0.00%** | **0.00%** | 5.71% | 2.18% | 3.29% | 5.83% | 4.23% |
| | | Mean | **0.00%** | **0.00%** | **0.00%** | 7.53% | 4.32% | 4.18% | 6.99% | 5.77% |
| GAP09 | obj | Best | **1.41E+03** | **1.41E+03** | **1.41E+03** | 1.45E+03 | 1.42E+03 | 1.41E+03 | 1.44E+03 | 1.42E+03 |
| | | Mean | **1.41E+03** | **1.41E+03** | **1.41E+03** | 1.47E+03 | 1.47E+03 | 1.42E+03 | 1.50E+03 | 1.43E+03 |
| | gap | Best | **0.00%** | **0.00%** | **0.00%** | 2.63% | 1.12% | 0.42% | 2.43% | 0.99% |
| | | Mean | **0.00%** | **0.00%** | **0.00%** | 4.56% | 4.05% | 0.94% | 6.18% | 1.51% |
| GAP10 | obj | Best | **2.83E+03** | **2.83E+03** | **2.83E+03** | 3.02E+03 | 2.97E+03 | 2.89E+03 | 2.98E+03 | 2.94E+03 |
| | | Mean | **2.83E+03** | **2.83E+03** | **2.83E+03** | 3.04E+03 | 3.01E+03 | 2.94E+03 | 3.08E+03 | 2.96E+03 |
| | gap | Best | **0.00%** | **0.00%** | **0.00%** | 6.51% | 4.85% | 2.32% | 4.97% | 3.78% |
| | | Mean | **0.00%** | **0.00%** | **0.00%** | 7.11% | 6.21% | 3.72% | 8.20% | 4.37% |
| GAP11 | obj | Best | **1.17E+03** | **1.17E+03** | **1.17E+03** | 1.19E+03 | 1.19E+03 | 1.17E+03 | 1.19E+03 | 1.18E+03 |
| | | Mean | **1.17E+03** | **1.17E+03** | **1.17E+03** | 1.21E+03 | 1.21E+03 | 1.18E+03 | 1.21E+03 | 1.19E+03 |
| | gap | Best | **0.00%** | **0.00%** | **0.00%** | 2.18% | 2.10% | 0.43% | 2.18% | 1.19% |
| | | Mean | **0.00%** | **0.00%** | **0.00%** | 3.45% | 3.69% | 1.28% | 3.41% | 1.98% |
| GAP12 | obj | Best | **2.34E+03** | **2.34E+03** | **2.34E+03** | 2.42E+03 | 2.37E+03 | 2.35E+03 | 2.37E+03 | 2.38E+03 |
| | | Mean | **2.34E+03** | **2.34E+03** | **2.34E+03** | 2.43E+03 | 2.41E+03 | 2.35E+03 | 2.40E+03 | 2.39E+03 |
| | gap | Best | **0.00%** | **0.00%** | **0.00%** | 3.15% | 1.47% | 0.26% | 1.47% | 1.72% |
| | | Mean | **0.00%** | **0.00%** | **0.00%** | 3.81% | 2.76% | 0.48% | 2.37% | 2.17% |
| GAP13 | obj | Best | **1.93E+03** | **1.93E+03** | **1.93E+03** | 2.03E+03 | 1.98E+03 | 1.99E+03 | 2.03E+03 | 1.97E+03 |
| | | Mean | **1.93E+03** | **1.93E+03** | **1.93E+03** | 2.05E+03 | 2.02E+03 | 2.00E+03 | 2.11E+03 | 1.99E+03 |
| | gap | Best | **0.00%** | **0.00%** | **0.00%** | 4.64% | 2.57% | 2.72% | 4.64% | 1.98% |
| | | Mean | **0.00%** | **0.00%** | **0.00%** | 5.84% | 4.53% | 3.66% | 8.31% | 3.12% |
| GAP14 | obj | Best | **3.46E+03** | **3.46E+03** | **3.46E+03** | 3.65E+03 | 3.53E+03 | 3.55E+03 | 3.66E+03 | 3.57E+03 |
| | | Mean | **3.46E+03** | **3.46E+03** | **3.46E+03** | 3.71E+03 | 3.62E+03 | 3.61E+03 | 3.73E+03 | 3.62E+03 |

| Pro. | Metric | Status | GUROBI | OR-TOOLS | SCIP | SA | VNS | LNS | TS | GA |
|---|---|---|---|---|---|---|---|---|---|---|
| | gap | Best | **0.00%** | **0.00%** | **0.00%** | 5.21% | 2.10% | 2.70% | 5.68% | 3.11% |
| | | Mean | **0.00%** | **0.00%** | **0.00%** | 6.82% | 4.52% | 4.28% | 7.38% | 4.63% |
| GAP15 | obj | Best | **1.40E+03** | **1.40E+03** | **1.40E+03** | 1.52E+03 | 1.49E+03 | 1.43E+03 | 1.48E+03 | 1.44E+03 |
| | | Mean | **1.40E+03** | **1.40E+03** | **1.40E+03** | 1.63E+03 | 1.53E+03 | 1.45E+03 | 1.52E+03 | 1.46E+03 |
| | gap | Best | **0.00%** | **0.00%** | **0.00%** | 7.82% | 5.59% | 2.23% | 5.01% | 2.50% |
| | | Mean | **0.00%** | **0.00%** | **0.00%** | 13.88% | 8.50% | 3.24% | 7.64% | 3.95% |
| GAP16 | obj | Best | **2.81E+03** | **2.81E+03** | **2.81E+03** | 3.01E+03 | 2.90E+03 | 2.89E+03 | 3.05E+03 | 2.94E+03 |
| | | Mean | **2.81E+03** | **2.81E+03** | **2.81E+03** | 3.06E+03 | 2.97E+03 | 2.93E+03 | 3.11E+03 | 2.96E+03 |
| | gap | Best | **0.00%** | **0.00%** | **0.00%** | 6.62% | 3.24% | 2.81% | 7.97% | 4.62% |
| | | Mean | **0.00%** | **0.00%** | **0.00%** | 8.40% | 5.35% | 4.30% | 9.72% | 5.35% |
| GAP17 | obj | Best | **5.60E+03** | **5.60E+03** | **5.60E+03** | 5.93E+03 | 5.73E+03 | 5.73E+03 | 5.90E+03 | 6.05E+03 |
| | | Mean | **5.60E+03** | **5.60E+03** | **5.60E+03** | 6.01E+03 | 5.85E+03 | 5.75E+03 | 6.01E+03 | 6.08E+03 |
| | gap | Best | **0.00%** | **0.00%** | **0.00%** | 5.68% | 2.36% | 2.30% | 5.06% | 7.47% |
| | | Mean | **0.00%** | **0.00%** | **0.00%** | 6.91% | 4.37% | 2.69% | 6.87% | 8.00% |
| GAP18 | obj | Best | 1.17E+04 | **1.13E+04** | 1.13E+04 | 1.23E+04 | 1.16E+04 | 1.16E+04 | 1.22E+04 | 1.19E+04 |
| | | Mean | 1.18E+04 | **1.13E+04** | 1.13E+04 | 1.24E+04 | 1.23E+04 | 1.18E+04 | 1.23E+04 | 1.21E+04 |
| | gap | Best | 3.09% | **0.00%** | 0.04% | 7.75% | 2.50% | 2.11% | 6.71% | 5.06% |
| | | Mean | 3.62% | **0.01%** | 0.04% | 8.74% | 7.33% | 3.48% | 7.65% | 6.43% |
| GAP19 | obj | Best | **1.24E+03** | **1.24E+03** | **1.24E+03** | 1.34E+03 | 1.31E+03 | 1.26E+03 | 1.29E+03 | 1.28E+03 |
| | | Mean | **1.24E+03** | **1.24E+03** | **1.24E+03** | 1.37E+03 | 1.32E+03 | 1.27E+03 | 1.34E+03 | 1.28E+03 |
| | gap | Best | **0.00%** | **0.00%** | **0.00%** | 7.03% | 4.75% | 1.66% | 3.49% | 2.51% |
| | | Mean | **0.00%** | **0.00%** | **0.00%** | 9.30% | 5.56% | 2.29% | 6.79% | 3.08% |
| GAP20 | obj | Best | **2.39E+03** | **2.39E+03** | **2.39E+03** | 2.51E+03 | 2.51E+03 | 2.43E+03 | 2.51E+03 | 2.51E+03 |
| | | Mean | **2.39E+03** | **2.39E+03** | **2.39E+03** | 2.59E+03 | 2.55E+03 | 2.46E+03 | 2.57E+03 | 2.52E+03 |
| | gap | Best | **0.00%** | **0.00%** | **0.00%** | 4.67% | 4.82% | 1.65% | 4.70% | 4.59% |
| | | Mean | **0.00%** | **0.00%** | **0.00%** | 7.80% | 6.27% | 2.64% | 6.82% | 5.22% |
| GAP21 | obj | Best | **4.78E+03** | **4.78E+03** | **4.78E+03** | 5.07E+03 | 5.14E+03 | 4.88E+03 | 5.07E+03 | 5.03E+03 |
| | | Mean | **4.78E+03** | **4.78E+03** | **4.78E+03** | 5.19E+03 | 5.26E+03 | 4.91E+03 | 5.21E+03 | 5.10E+03 |
| | gap | Best | **0.00%** | **0.00%** | **0.00%** | 5.59% | 7.02% | 1.99% | 5.61% | 4.87% |
| | | Mean | **0.00%** | **0.00%** | **0.00%** | 7.83% | 8.95% | 2.56% | 8.22% | 6.18% |
| GAP22 | obj | Best | 1.11E+04 | **9.98E+03** | 9.99E+03 | 1.07E+04 | 1.07E+04 | 1.02E+04 | 1.06E+04 | 1.07E+04 |
| | | Mean | 1.11E+04 | **9.98E+03** | 9.99E+03 | 1.09E+04 | 1.10E+04 | 1.04E+04 | 1.07E+04 | 1.15E+04 |
| | gap | Best | 9.85% | **0.01%** | 0.06% | 6.33% | 6.43% | 2.09% | 5.89% | 6.73% |
| | | Mean | 9.85% | **0.02%** | 0.06% | 8.22% | 8.85% | 3.58% | 6.94% | 12.54% |
| GAP23 | obj | Best | **4.24E+03** | **4.24E+03** | **4.24E+03** | 4.37E+03 | 4.34E+03 | 4.27E+03 | 4.36E+03 | 4.38E+03 |
| | | Mean | **4.24E+03** | **4.24E+03** | **4.24E+03** | 4.47E+03 | 4.37E+03 | 4.31E+03 | 4.42E+03 | 4.42E+03 |
| | gap | Best | **0.00%** | **0.00%** | **0.00%** | 2.93% | 2.23% | 0.56% | 2.57% | 3.15% |
| | | Mean | **0.00%** | **0.00%** | **0.00%** | 5.11% | 2.92% | 1.50% | 4.05% | 4.03% |
| GAP24 | obj | Best | 9.43E+03 | **9.33E+03** | 9.34E+03 | 9.62E+03 | 9.52E+03 | 9.41E+03 | 9.62E+03 | 9.65E+03 |
| | | Mean | 9.49E+03 | **9.33E+03** | 9.34E+03 | 9.72E+03 | 9.57E+03 | 9.58E+03 | 9.65E+03 | 1.14E+04 |
| | gap | Best | 1.13% | **0.02%** | 0.12% | 3.08% | 2.01% | 0.91% | 3.08% | 3.37% |
| | | Mean | 1.71% | **0.04%** | 0.12% | 4.08% | 2.50% | 2.62% | 3.34% | 15.58% |
| GAP25 | obj | Best | 1.90E+04 | **1.88E+04** | 1.88E+04 | 2.04E+04 | 2.06E+04 | 1.93E+04 | 2.03E+04 | 2.03E+04 |
| | | Mean | 1.90E+04 | **1.88E+04** | 1.88E+04 | 2.05E+04 | 2.15E+04 | 1.95E+04 | 2.04E+04 | 2.24E+04 |
| | gap | Best | 0.94% | **0.01%** | 0.02% | 7.68% | 8.68% | 2.41% | 7.37% | 7.49% |
| | | Mean | 0.94% | **0.01%** | 0.02% | 8.31% | 12.20% | 3.48% | 7.89% | 15.81% |

| Pro. | Metric | Status | GUROBI | OR-TOOLS | SCIP | SA | VNS | LNS | TS | GA |
|---|---|---|---|---|---|---|---|---|---|---|
| GAP26 | obj | Best | 1.74E+04 | **1.71E+04** | 1.72E+04 | 1.79E+04 | 1.80E+04 | 1.74E+04 | 1.79E+04 | 1.84E+04 |
| | | Mean | 1.74E+04 | **1.71E+04** | 1.72E+04 | 1.83E+04 | 1.82E+04 | 1.75E+04 | 1.83E+04 | 2.09E+04 |
| | gap | Best | 1.34% | **0.02%** | 0.05% | 4.39% | 4.65% | 1.56% | 4.24% | 6.67% |
| | | Mean | 1.34% | **0.02%** | 0.05% | 6.11% | 5.80% | 1.77% | 6.21% | 17.63% |
| GAP27 | obj | Best | NAN | **1.63E+04** | NAN | 1.68E+04 | 1.66E+04 | 1.70E+04 | 1.68E+04 | 2.14E+04 |
| | | Mean | NAN | **1.63E+04** | NAN | 1.68E+04 | 1.68E+04 | 1.70E+04 | 1.68E+04 | 2.16E+04 |
| | gap | Best | NAN | **0.04%** | NAN | 2.92% | 1.66% | 4.05% | 3.00% | 24.08% |
| | | Mean | NAN | **0.04%** | NAN | 3.33% | 2.96% | 4.23% | 3.33% | 24.71% |
| GAP28 | obj | Best | **6.35E+03** | **6.35E+03** | 6.36E+03 | 6.72E+03 | 6.83E+03 | 6.59E+03 | 6.82E+03 | 6.61E+03 |
| | | Mean | **6.35E+03** | 6.35E+03 | 6.36E+03 | 6.78E+03 | 6.86E+03 | 6.64E+03 | 6.86E+03 | 6.62E+03 |
| | gap | Best | **0.00%** | **0.00%** | 0.08% | 5.43% | 7.00% | 3.57% | 6.81% | 3.82% |
| | | Mean | **0.00%** | 0.02% | 0.08% | 6.24% | 7.33% | 4.38% | 7.43% | 3.99% |
| GAP29 | obj | Best | 1.27E+04 | **1.27E+04** | 1.28E+04 | 1.36E+04 | 1.38E+04 | 1.32E+04 | 1.36E+04 | 1.32E+04 |
| | | Mean | 1.27E+04 | **1.27E+04** | 1.28E+04 | 1.36E+04 | 1.39E+04 | 1.32E+04 | 1.37E+04 | 1.33E+04 |
| | gap | Best | 0.05% | **0.02%** | 0.06% | 6.09% | 7.85% | 3.28% | 6.11% | 3.70% |
| | | Mean | 0.05% | **0.03%** | 0.06% | 6.61% | 8.03% | 3.65% | 6.89% | 4.13% |
| GAP30 | obj | Best | 6.38E+03 | **6.36E+03** | 6.38E+03 | 6.81E+03 | 6.91E+03 | 6.73E+03 | 6.88E+03 | 6.69E+03 |
| | | Mean | 6.38E+03 | **6.37E+03** | 6.38E+03 | 6.96E+03 | 6.99E+03 | 6.78E+03 | 6.96E+03 | 6.75E+03 |
| | gap | Best | 0.47% | **0.19%** | 0.56% | 6.80% | 8.20% | 5.63% | 7.75% | 5.13% |
| | | Mean | 0.47% | **0.33%** | 0.56% | 8.74% | 9.20% | 6.35% | 8.77% | 5.90% |
| GAP31 | obj | Best | 1.25E+04 | **1.24E+04** | 1.25E+04 | 1.37E+04 | 1.35E+04 | 1.30E+04 | 1.36E+04 | 1.32E+04 |
| | | Mean | 1.25E+04 | **1.25E+04** | 1.25E+04 | 1.38E+04 | 1.37E+04 | 1.32E+04 | 1.36E+04 | 1.33E+04 |
| | gap | Best | 0.31% | **0.18%** | 0.30% | 9.17% | 8.17% | 4.50% | 8.54% | 5.64% |
| | | Mean | 0.31% | **0.22%** | 0.30% | 9.82% | 9.59% | 5.75% | 8.95% | 6.34% |
| GAP32 | obj | Best | 2.50E+04 | **2.50E+04** | 2.50E+04 | 2.65E+04 | 2.69E+04 | 2.59E+04 | 2.65E+04 | 2.64E+04 |
| | | Mean | 2.50E+04 | **2.50E+04** | 2.50E+04 | 2.67E+04 | 2.73E+04 | 2.60E+04 | 2.70E+04 | 2.64E+04 |
| | gap | Best | 0.11% | **0.04%** | 0.08% | 5.81% | 7.31% | 3.74% | 5.91% | 5.37% |
| | | Mean | 0.11% | **0.05%** | 0.08% | 6.65% | 8.54% | 4.15% | 7.53% | 5.45% |
| GAP33 | obj | Best | 5.56E+04 | **5.54E+04** | 5.55E+04 | 5.93E+04 | 6.14E+04 | 5.78E+04 | 5.96E+04 | 5.92E+04 |
| | | Mean | 5.56E+04 | 5.62E+04 | **5.55E+04** | 5.97E+04 | 6.21E+04 | 5.82E+04 | 5.98E+04 | 5.93E+04 |
| | gap | Best | 0.37% | **0.07%** | 0.11% | 6.59% | 9.77% | 4.20% | 7.10% | 6.39% |
| | | Mean | 0.37% | 1.30% | **0.11%** | 7.23% | 10.71% | 4.74% | 7.38% | 6.57% |
| GAP34 | obj | Best | 6.32E+03 | **6.23E+03** | 6.29E+03 | 6.68E+03 | 6.70E+03 | 6.53E+03 | 6.72E+03 | 6.49E+03 |
| | | Mean | 6.32E+03 | **6.24E+03** | 6.29E+03 | 6.81E+03 | 6.76E+03 | 6.60E+03 | 6.85E+03 | 6.56E+03 |
| | gap | Best | 2.29% | **0.82%** | 1.73% | 7.56% | 7.85% | 5.45% | 8.11% | 4.84% |
| | | Mean | 2.29% | **0.99%** | 1.73% | 9.28% | 8.66% | 6.37% | 9.75% | 5.89% |
| GAP35 | obj | Best | 1.25E+04 | **1.23E+04** | 1.24E+04 | 1.32E+04 | 1.33E+04 | 1.29E+04 | 1.34E+04 | 1.32E+04 |
| | | Mean | 1.25E+04 | **1.23E+04** | 1.24E+04 | 1.33E+04 | 1.34E+04 | 1.30E+04 | 1.35E+04 | 1.32E+04 |
| | gap | Best | 1.85% | **0.46%** | 1.15% | 7.15% | 8.03% | 5.48% | 8.83% | 7.28% |
| | | Mean | 1.85% | **0.65%** | 1.15% | 7.95% | 8.52% | 6.19% | 9.66% | 7.63% |
| GAP36 | obj | Best | 2.48E+04 | **2.46E+04** | 2.47E+04 | 2.66E+04 | 2.69E+04 | 2.60E+04 | 2.71E+04 | 2.65E+04 |
| | | Mean | 2.48E+04 | **2.46E+04** | 2.47E+04 | 2.69E+04 | 2.74E+04 | 2.62E+04 | 2.72E+04 | 2.66E+04 |
| | gap | Best | 1.06% | **0.23%** | 0.41% | 7.55% | 8.57% | 5.43% | 9.35% | 7.15% |
| | | Mean | 1.06% | **0.36%** | 0.41% | 8.59% | 10.41% | 6.11% | 9.79% | 7.53% |
| GAP37 | obj | Best | 5.55E+04 | **5.49E+04** | 5.50E+04 | 5.94E+04 | 6.14E+04 | 5.83E+04 | 6.03E+04 | 5.96E+04 |
| | | Mean | 5.55E+04 | **5.50E+04** | 5.50E+04 | 6.00E+04 | 6.22E+04 | 5.84E+04 | 6.09E+04 | 5.97E+04 |

| Pro. | Metric | Status | GUROBI | OR-TOOLS | SCIP | SA | VNS | LNS | TS | GA |
|---|---|---|---|---|---|---|---|---|---|---|
| | gap | Best | 1.18% | **0.18%** | 0.39% | 7.76% | 10.64% | 5.89% | 9.05% | 8.01% |
| | | Mean | 1.18% | **0.25%** | 0.39% | 8.55% | 11.89% | 6.16% | 9.99% | 8.14% |
| GAP38 | obj | Best | 2.50E+04 | **2.45E+04** | 2.46E+04 | 2.66E+04 | 2.67E+04 | 2.60E+04 | 2.70E+04 | 2.66E+04 |
| | | Mean | 2.50E+04 | **2.45E+04** | 2.46E+04 | 2.69E+04 | 2.70E+04 | 2.62E+04 | 2.72E+04 | 2.68E+04 |
| | gap | Best | 2.48% | **0.72%** | 1.22% | 8.41% | 8.81% | 6.38% | 9.87% | 8.49% |
| | | Mean | 2.48% | **0.82%** | 1.22% | 9.44% | 9.69% | 7.04% | 10.48% | 9.03% |
| GAP39 | obj | Best | NAN | **5.48E+04** | 5.50E+04 | 5.95E+04 | 6.02E+04 | 5.85E+04 | 6.05E+04 | 5.96E+04 |
| | | Mean | NAN | **5.48E+04** | 5.50E+04 | 6.01E+04 | 6.09E+04 | 5.86E+04 | 6.11E+04 | 5.98E+04 |
| | gap | Best | NAN | **0.46%** | 0.88% | 8.39% | 9.35% | 6.76% | 9.87% | 8.41% |
| | | Mean | NAN | **0.50%** | 0.88% | 9.20% | 10.40% | 6.97% | 10.72% | 8.72% |
| GAP40 | obj | Best | 9.84E+04 | **9.79E+04** | 9.79E+04 | 1.05E+05 | 1.03E+05 | 1.02E+05 | 1.07E+05 | 1.09E+05 |
| | | Mean | 9.84E+04 | **9.79E+04** | 9.79E+04 | 1.06E+05 | 1.10E+05 | 1.03E+05 | 1.07E+05 | 1.10E+05 |
| | gap | Best | 0.56% | **0.06%** | 0.11% | 7.18% | 4.77% | 4.45% | 8.39% | 10.66% |
| | | Mean | 0.56% | **0.07%** | 0.11% | 7.83% | 10.66% | 4.61% | 8.87% | 10.81% |
| GAP41 | obj | Best | NAN | **9.73E+04** | 9.75E+04 | 1.06E+05 | 1.03E+05 | 1.06E+05 | 1.07E+05 | 1.10E+05 |
| | | Mean | NAN | **9.73E+04** | 9.75E+04 | 1.07E+05 | 1.09E+05 | 1.06E+05 | 1.08E+05 | 1.10E+05 |
| | gap | Best | NAN | **0.17%** | 0.39% | 8.37% | 6.11% | 8.29% | 9.36% | 11.42% |
| | | Mean | NAN | **0.19%** | 0.39% | 9.17% | 10.66% | 8.53% | 9.69% | 11.56% |
| GAP42 | obj | Best | NAN | **9.73E+04** | 9.76E+04 | 1.07E+05 | 1.04E+05 | 1.05E+05 | 1.08E+05 | 1.09E+05 |
| | | Mean | NAN | **9.74E+04** | 9.76E+04 | 1.08E+05 | 1.09E+05 | 1.06E+05 | 1.09E+05 | 1.10E+05 |
| | gap | Best | NAN | **0.32%** | 0.59% | 9.63% | 7.13% | 7.73% | 10.43% | 11.34% |
| | | Mean | NAN | **0.35%** | 0.59% | 10.03% | 10.69% | 8.36% | 11.20% | 11.73% |
| GAP43 | obj | Best | **1.27E+04** | **1.27E+04** | **1.27E+04** | 1.45E+04 | 1.53E+04 | 1.32E+04 | 1.42E+04 | 1.43E+04 |
| | | Mean | **1.27E+04** | **1.27E+04** | **1.27E+04** | 1.60E+04 | 1.65E+04 | 1.37E+04 | 1.61E+04 | 1.47E+04 |
| | gap | Best | **0.00%** | **0.00%** | **0.00%** | 12.26% | 17.03% | 3.73% | 10.84% | 11.44% |
| | | Mean | **0.00%** | **0.00%** | **0.00%** | 20.46% | 22.86% | 7.18% | 20.14% | 13.76% |
| GAP44 | obj | Best | **2.49E+04** | **2.49E+04** | **2.49E+04** | 3.17E+04 | 3.29E+04 | 2.66E+04 | 3.19E+04 | 2.82E+04 |
| | | Mean | **2.49E+04** | **2.49E+04** | **2.49E+04** | 3.41E+04 | 3.62E+04 | 2.71E+04 | 3.40E+04 | 2.89E+04 |
| | gap | Best | **0.00%** | **0.00%** | **0.00%** | 21.34% | 24.14% | 6.24% | 21.74% | 11.66% |
| | | Mean | **0.00%** | **0.00%** | **0.00%** | 26.61% | 30.73% | 7.99% | 26.52% | 13.77% |
| GAP45 | obj | Best | **1.16E+04** | **1.16E+04** | **1.16E+04** | 1.38E+04 | 1.41E+04 | 1.25E+04 | 1.32E+04 | 1.28E+04 |
| | | Mean | **1.16E+04** | 1.16E+04 | **1.16E+04** | 1.55E+04 | 1.48E+04 | 1.28E+04 | 1.48E+04 | 1.32E+04 |
| | gap | Best | **0.00%** | **0.00%** | **0.00%** | 16.36% | 17.88% | 7.17% | 12.60% | 9.75% |
| | | Mean | **0.00%** | 0.01% | **0.00%** | 24.75% | 21.53% | 9.72% | 21.30% | 12.38% |
| GAP46 | obj | Best | **2.33E+04** | **2.33E+04** | **2.33E+04** | 2.90E+04 | 2.95E+04 | 2.55E+04 | 2.76E+04 | 2.68E+04 |
| | | Mean | **2.33E+04** | **2.33E+04** | **2.33E+04** | 3.06E+04 | 3.11E+04 | 2.58E+04 | 2.82E+04 | 2.77E+04 |
| | gap | Best | **0.01%** | **0.01%** | **0.01%** | 19.51% | 20.90% | 8.78% | 15.47% | 13.09% |
| | | Mean | **0.01%** | **0.01%** | **0.01%** | 23.72% | 24.83% | 9.54% | 17.27% | 15.76% |
| GAP47 | obj | Best | 4.57E+04 | **4.57E+04** | **4.57E+04** | 5.48E+04 | 5.32E+04 | 5.01E+04 | 5.49E+04 | 5.50E+04 |
| | | Mean | 4.57E+04 | **4.57E+04** | **4.57E+04** | 5.59E+04 | 5.72E+04 | 5.07E+04 | 5.65E+04 | 5.59E+04 |
| | gap | Best | 0.01% | **0.00%** | **0.00%** | 16.51% | 14.08% | 8.70% | 16.65% | 16.77% |
| | | Mean | 0.01% | **0.00%** | **0.00%** | 18.15% | 19.56% | 9.77% | 18.94% | 18.22% |
| GAP48 | obj | Best | **1.02E+05** | **1.02E+05** | **1.02E+05** | 1.23E+05 | 1.25E+05 | 1.15E+05 | 1.26E+05 | 1.30E+05 |
| | | Mean | **1.02E+05** | **1.02E+05** | **1.02E+05** | 1.29E+05 | 1.37E+05 | 1.17E+05 | 1.29E+05 | 1.37E+05 |
| | gap | Best | **0.00%** | **0.00%** | **0.00%** | 16.95% | 17.93% | 10.87% | 18.72% | 21.02% |
| | | Mean | **0.00%** | **0.00%** | **0.00%** | 20.19% | 24.37% | 12.08% | 20.78% | 24.85% |

| Pro. | Metric | Status | GUROBI | OR-TOOLS | SCIP | SA | VNS | LNS | TS | GA |
|---|---|---|---|---|---|---|---|---|---|---|
| GAP49 | obj | Best | **8.44E+03** | **8.44E+03** | **8.44E+03** | 9.71E+03 | 9.83E+03 | 9.00E+03 | 9.79E+03 | 9.59E+03 |
| | | Mean | **8.44E+03** | 8.47E+03 | **8.44E+03** | 1.00E+04 | 1.01E+04 | 9.19E+03 | 1.02E+04 | 9.97E+03 |
| | gap | Best | **0.00%** | **0.00%** | **0.00%** | 13.16% | 14.17% | 6.25% | 13.80% | 12.01% |
| | | Mean | **0.00%** | 0.41% | **0.00%** | 15.82% | 16.73% | 8.19% | 17.14% | 15.29% |
| GAP50 | obj | Best | **2.24E+04** | **2.24E+04** | **2.24E+04** | 2.59E+04 | 2.59E+04 | 2.42E+04 | 2.73E+04 | 2.61E+04 |
| | | Mean | **2.24E+04** | **2.24E+04** | **2.24E+04** | 2.73E+04 | 2.72E+04 | 2.48E+04 | 2.74E+04 | 2.67E+04 |
| | gap | Best | **0.00%** | **0.00%** | **0.00%** | 13.45% | 13.44% | 7.48% | 17.91% | 14.38% |
| | | Mean | **0.00%** | **0.00%** | **0.00%** | 17.86% | 17.51% | 9.64% | 18.21% | 16.03% |
| GAP51 | obj | Best | **4.49E+04** | **4.49E+04** | **4.49E+04** | 5.45E+04 | 5.34E+04 | 5.00E+04 | 5.44E+04 | 5.43E+04 |
| | | Mean | **4.49E+04** | **4.49E+04** | **4.49E+04** | 5.57E+04 | 5.49E+04 | 5.06E+04 | 5.56E+04 | 5.59E+04 |
| | gap | Best | **0.01%** | **0.00%** | **0.00%** | 17.63% | 15.90% | 10.27% | 17.55% | 17.32% |
| | | Mean | **0.01%** | **0.00%** | **0.00%** | 19.47% | 18.26% | 11.23% | 19.26% | 19.66% |
| GAP52 | obj | Best | 1.04E+05 | **1.00E+05** | **1.00E+05** | 1.23E+05 | 1.21E+05 | 1.14E+05 | 1.21E+05 | 1.25E+05 |
| | | Mean | 1.04E+05 | **1.00E+05** | **1.00E+05** | 1.26E+05 | 1.30E+05 | 1.15E+05 | 1.27E+05 | 1.30E+05 |
| | gap | Best | 3.86% | **0.00%** | **0.00%** | 18.03% | 17.19% | 12.28% | 16.95% | 19.47% |
| | | Mean | 3.86% | **0.00%** | **0.00%** | 20.43% | 22.05% | 12.93% | 20.56% | 22.76% |
| GAP53 | obj | Best | 4.64E+04 | **4.46E+04** | 4.46E+04 | 5.33E+04 | 5.22E+04 | 4.96E+04 | 5.44E+04 | 5.41E+04 |
| | | Mean | 4.64E+04 | **4.46E+04** | 4.46E+04 | 5.41E+04 | 5.51E+04 | 5.01E+04 | 5.60E+04 | 5.51E+04 |
| | gap | Best | 3.92% | **0.00%** | 0.17% | 16.42% | 14.65% | 10.19% | 18.12% | 17.56% |
| | | Mean | 3.92% | **0.00%** | 0.17% | 17.66% | 18.85% | 11.00% | 20.38% | 19.03% |
| GAP54 | obj | Best | 1.04E+05 | **1.00E+05** | 1.02E+05 | 1.21E+05 | 1.20E+05 | 1.15E+05 | 1.26E+05 | 1.27E+05 |
| | | Mean | 1.04E+05 | **1.00E+05** | 1.02E+05 | 1.24E+05 | 1.27E+05 | 1.18E+05 | 1.33E+05 | 1.31E+05 |
| | gap | Best | 3.83% | **0.00%** | 1.39% | 17.50% | 16.86% | 13.13% | 20.42% | 21.25% |
| | | Mean | 3.83% | **0.03%** | 1.39% | 19.06% | 20.76% | 14.89% | 24.41% | 23.31% |
| GAP55 | obj | Best | 1.85E+05 | **1.81E+05** | **1.81E+05** | 2.32E+05 | 2.82E+05 | 2.27E+05 | 2.17E+05 | 3.02E+05 |
| | | Mean | 1.85E+05 | **1.81E+05** | **1.81E+05** | 2.37E+05 | 2.88E+05 | 2.31E+05 | 2.45E+05 | 3.21E+05 |
| | gap | Best | 2.41% | **0.00%** | **0.00%** | 22.28% | 35.83% | 20.40% | 16.69% | 40.22% |
| | | Mean | 2.60% | **0.00%** | **0.00%** | 23.73% | 37.16% | 21.73% | 26.03% | 43.53% |
| GAP56 | obj | Best | 1.82E+05 | **1.78E+05** | 1.79E+05 | 2.28E+05 | 2.52E+05 | 2.22E+05 | 2.48E+05 | 3.04E+05 |
| | | Mean | 1.82E+05 | **1.78E+05** | 1.79E+05 | 2.40E+05 | 2.71E+05 | 2.27E+05 | 2.50E+05 | 3.13E+05 |
| | gap | Best | 1.92% | **0.00%** | 0.45% | 21.75% | 29.12% | 19.72% | 28.06% | 41.38% |
| | | Mean | 1.92% | **0.01%** | 0.45% | 25.45% | 33.98% | 21.33% | 28.79% | 43.05% |
| GAP57 | obj | Best | NAN | **1.77E+05** | 1.79E+05 | 2.33E+05 | 2.65E+05 | 2.24E+05 | 2.45E+05 | 3.20E+05 |
| | | Mean | NAN | **1.77E+05** | 1.79E+05 | 2.40E+05 | 2.71E+05 | 2.35E+05 | 2.51E+05 | 3.37E+05 |
| | gap | Best | NAN | **0.00%** | 1.28% | 24.10% | 33.29% | 20.90% | 27.74% | 44.83% |
| | | Mean | NAN | **0.04%** | 1.28% | 26.08% | 34.71% | 24.74% | 29.59% | 47.49% |

### 3.4 Capacitated facility location problem (CFLP)

The experimental results of CFLP are presented in Table S-14.

**Table S-14** Experimental results on CFLP test suit.

| Pro. | Metric | Status | GUROBI | OR-TOOLS | SCIP | SA | VNS | LNS | TS | GA |
|---|---|---|---|---|---|---|---|---|---|---|
| CFLP01 | obj | Best | **2.84E+03** | 2.89E+03 | 2.94E+03 | 3.29E+03 | 3.47E+03 | 3.13E+03 | 3.75E+03 | 3.37E+03 |
| | | Mean | **2.84E+03** | 2.97E+03 | 2.98E+03 | 3.45E+03 | 3.58E+03 | 3.17E+03 | 3.81E+03 | 3.46E+03 |
| | gap | Best | **0.00%** | 1.51% | 3.36% | 13.48% | 18.09% | 9.15% | 24.19% | 15.73% |
| | | Mean | **0.00%** | 4.12% | 4.54% | 17.56% | 20.58% | 10.18% | 25.45% | 17.79% |

| Pro. | Metric | Status | GUROBI | OR-TOOLS | SCIP | SA | VNS | LNS | TS | GA |
|---|---|---|---|---|---|---|---|---|---|---|
| CFLP02 | obj | Best | **2.98E+03** | 3.05E+03 | 3.15E+03 | 3.56E+03 | 3.61E+03 | 3.35E+03 | 3.80E+03 | 3.45E+03 |
| | | Mean | **2.98E+03** | 3.07E+03 | 3.20E+03 | 3.67E+03 | 3.74E+03 | 3.39E+03 | 4.02E+03 | 3.56E+03 |
| | gap | Best | **0.00%** | 2.34% | 5.49% | 16.46% | 17.67% | 11.13% | 21.62% | 13.66% |
| | | Mean | **0.00%** | 3.07% | 6.87% | 18.96% | 20.45% | 12.24% | 25.85% | 16.38% |
| CFLP03 | obj | Best | **3.04E+03** | 3.12E+03 | 3.25E+03 | 3.64E+03 | 3.59E+03 | 3.25E+03 | 3.73E+03 | 3.57E+03 |
| | | Mean | **3.04E+03** | 3.16E+03 | 3.25E+03 | 3.78E+03 | 3.73E+03 | 3.35E+03 | 3.93E+03 | 3.68E+03 |
| | gap | Best | **0.00%** | 2.46% | 6.47% | 16.54% | 15.39% | 6.41% | 18.46% | 14.89% |
| | | Mean | **0.00%** | 3.79% | 6.52% | 19.56% | 18.49% | 9.26% | 22.53% | 17.31% |
| CFLP04 | obj | Best | **2.98E+03** | 3.05E+03 | 3.17E+03 | 3.52E+03 | 3.61E+03 | 3.28E+03 | 3.76E+03 | 3.54E+03 |
| | | Mean | **2.98E+03** | 3.11E+03 | 3.17E+03 | 3.62E+03 | 3.70E+03 | 3.31E+03 | 3.93E+03 | 3.63E+03 |
| | gap | Best | **0.00%** | 2.19% | 5.89% | 15.25% | 17.43% | 8.99% | 20.55% | 15.61% |
| | | Mean | **0.00%** | 3.96% | 5.89% | 17.44% | 19.34% | 9.87% | 24.03% | 17.62% |
| CFLP05 | obj | Best | **3.04E+03** | 3.14E+03 | 3.25E+03 | 3.48E+03 | 3.59E+03 | 3.31E+03 | 3.68E+03 | 3.40E+03 |
| | | Mean | **3.04E+03** | 3.17E+03 | 3.26E+03 | 3.66E+03 | 3.67E+03 | 3.36E+03 | 3.77E+03 | 3.50E+03 |
| | gap | Best | **0.00%** | 3.14% | 6.57% | 12.58% | 15.38% | 8.04% | 17.27% | 10.49% |
| | | Mean | **0.00%** | 4.17% | 6.59% | 16.74% | 17.21% | 9.49% | 19.19% | 13.06% |
| CFLP06 | obj | Best | **2.95E+03** | 3.08E+03 | 3.13E+03 | 3.49E+03 | 3.61E+03 | 3.27E+03 | 3.75E+03 | 3.47E+03 |
| | | Mean | **2.95E+03** | 3.15E+03 | 3.13E+03 | 3.64E+03 | 3.70E+03 | 3.33E+03 | 3.83E+03 | 3.56E+03 |
| | gap | Best | **0.00%** | 4.17% | 5.57% | 15.23% | 18.16% | 9.52% | 21.21% | 14.88% |
| | | Mean | **0.00%** | 6.14% | 5.57% | 18.80% | 20.04% | 11.28% | 22.89% | 17.03% |
| CFLP07 | obj | Best | **2.89E+03** | 3.04E+03 | 3.03E+03 | 3.38E+03 | 3.59E+03 | 3.24E+03 | 3.34E+03 | 3.37E+03 |
| | | Mean | **2.89E+03** | 3.11E+03 | 3.03E+03 | 3.51E+03 | 3.72E+03 | 3.27E+03 | 3.77E+03 | 3.46E+03 |
| | gap | Best | **0.00%** | 5.21% | 4.60% | 14.65% | 19.63% | 11.02% | 13.47% | 14.26% |
| | | Mean | **0.00%** | 7.16% | 4.71% | 17.65% | 22.32% | 11.79% | 23.04% | 16.49% |
| CFLP08 | obj | Best | **2.94E+03** | 3.00E+03 | 3.14E+03 | 3.58E+03 | 3.56E+03 | 3.27E+03 | 3.67E+03 | 3.38E+03 |
| | | Mean | **2.94E+03** | 3.09E+03 | 3.15E+03 | 3.72E+03 | 3.72E+03 | 3.30E+03 | 3.94E+03 | 3.59E+03 |
| | gap | Best | **0.00%** | 2.08% | 6.39% | 17.88% | 17.36% | 10.03% | 19.99% | 13.13% |
| | | Mean | **0.00%** | 4.70% | 6.59% | 20.91% | 20.91% | 11.02% | 25.35% | 17.91% |
| CFLP09 | obj | Best | **2.23E+03** | 2.28E+03 | 2.27E+03 | 2.58E+03 | 2.66E+03 | 2.50E+03 | 2.69E+03 | 2.57E+03 |
| | | Mean | **2.23E+03** | 2.31E+03 | 2.28E+03 | 2.70E+03 | 2.75E+03 | 2.54E+03 | 2.78E+03 | 2.59E+03 |
| | gap | Best | **0.00%** | 1.98% | 1.53% | 13.53% | 16.15% | 10.69% | 16.88% | 13.15% |
| | | Mean | **0.00%** | 3.17% | 1.92% | 17.11% | 18.72% | 12.16% | 19.56% | 13.76% |
| CFLP10 | obj | Best | **2.30E+03** | 2.32E+03 | 2.33E+03 | 2.64E+03 | 2.63E+03 | 2.50E+03 | 2.71E+03 | 2.66E+03 |
| | | Mean | **2.30E+03** | 2.37E+03 | 2.34E+03 | 2.71E+03 | 2.68E+03 | 2.58E+03 | 2.76E+03 | 2.71E+03 |
| | gap | Best | **0.00%** | 0.63% | 1.28% | 12.74% | 12.35% | 7.81% | 15.08% | 13.40% |
| | | Mean | **0.00%** | 2.62% | 1.43% | 14.98% | 14.18% | 10.52% | 16.49% | 14.92% |
| CFLP11 | obj | Best | **2.25E+03** | 2.32E+03 | 2.30E+03 | 2.55E+03 | 2.57E+03 | 2.52E+03 | 2.59E+03 | 2.67E+03 |
| | | Mean | **2.25E+03** | 2.35E+03 | 2.30E+03 | 2.65E+03 | 2.69E+03 | 2.60E+03 | 2.74E+03 | 2.73E+03 |
| | gap | Best | **0.00%** | 3.20% | 2.16% | 11.90% | 12.43% | 10.92% | 13.22% | 15.80% |
| | | Mean | **0.00%** | 4.40% | 2.16% | 15.25% | 16.28% | 13.64% | 17.96% | 17.73% |
| CFLP12 | obj | Best | **2.24E+03** | 2.32E+03 | 2.25E+03 | 2.52E+03 | 2.65E+03 | 2.42E+03 | 2.58E+03 | 2.56E+03 |
| | | Mean | **2.24E+03** | 2.36E+03 | 2.26E+03 | 2.67E+03 | 2.68E+03 | 2.52E+03 | 2.70E+03 | 2.60E+03 |
| | gap | Best | **0.00%** | 3.43% | 0.56% | 11.19% | 15.41% | 7.29% | 13.09% | 12.39% |
| | | Mean | **0.00%** | 5.12% | 0.66% | 15.90% | 16.53% | 11.15% | 16.96% | 13.70% |
| CFLP13 | obj | Best | **2.25E+03** | 2.34E+03 | 2.29E+03 | 2.60E+03 | 2.58E+03 | 2.46E+03 | 2.60E+03 | 2.56E+03 |
| | | Mean | **2.25E+03** | 2.38E+03 | 2.29E+03 | 2.69E+03 | 2.71E+03 | 2.56E+03 | 2.76E+03 | 2.66E+03 |
| | gap | Best | **0.00%** | 3.85% | 1.74% | 13.26% | 12.75% | 8.23% | 13.22% | 12.11% |

| Pro. | Metric | Status | GUROBI | OR-TOOLS | SCIP | SA | VNS | LNS | TS | GA |
|---|---|---|---|---|---|---|---|---|---|---|
| | | Mean | **0.00%** | 5.43% | 1.74% | 16.28% | 16.66% | 11.83% | 18.35% | 15.34% |
| CFLP14 | obj | Best | **2.18E+03** | 2.22E+03 | 2.21E+03 | 2.51E+03 | 2.44E+03 | 2.39E+03 | 2.48E+03 | 2.53E+03 |
| | | Mean | **2.18E+03** | 2.25E+03 | 2.21E+03 | 2.60E+03 | 2.56E+03 | 2.49E+03 | 2.58E+03 | 2.57E+03 |
| | gap | Best | **0.00%** | 1.43% | 1.26% | 13.10% | 10.33% | 8.71% | 11.96% | 13.48% |
| | | Mean | **0.00%** | 2.68% | 1.28% | 15.98% | 14.69% | 12.06% | 15.08% | 14.81% |
| CFLP15 | obj | Best | **2.24E+03** | 2.27E+03 | 2.25E+03 | 2.51E+03 | 2.60E+03 | 2.39E+03 | 2.70E+03 | 2.50E+03 |
| | | Mean | **2.24E+03** | 2.30E+03 | 2.25E+03 | 2.62E+03 | 2.67E+03 | 2.49E+03 | 2.82E+03 | 2.63E+03 |
| | gap | Best | **0.00%** | 1.36% | 0.71% | 11.02% | 14.00% | 6.64% | 17.12% | 10.40% |
| | | Mean | **0.00%** | 2.62% | 0.82% | 14.61% | 16.32% | 10.02% | 20.45% | 15.01% |
| CFLP16 | obj | Best | **2.27E+03** | 2.31E+03 | 2.32E+03 | 2.52E+03 | 2.60E+03 | 2.50E+03 | 2.68E+03 | 2.62E+03 |
| | | Mean | **2.27E+03** | 2.32E+03 | 2.32E+03 | 2.60E+03 | 2.70E+03 | 2.57E+03 | 2.78E+03 | 2.71E+03 |
| | gap | Best | **0.00%** | 1.62% | 2.27% | 10.11% | 12.89% | 9.22% | 15.42% | 13.49% |
| | | Mean | **0.00%** | 2.37% | 2.27% | 12.71% | 15.94% | 11.60% | 18.28% | 16.35% |
| CFLP17 | obj | Best | **2.06E+03** | 2.08E+03 | 2.07E+03 | 2.29E+03 | 2.35E+03 | 2.13E+03 | 2.31E+03 | 2.33E+03 |
| | | Mean | **2.06E+03** | 2.09E+03 | 2.08E+03 | 2.39E+03 | 2.47E+03 | 2.28E+03 | 2.48E+03 | 2.39E+03 |
| | gap | Best | **0.00%** | 1.31% | 0.68% | 10.25% | 12.37% | 3.41% | 11.03% | 11.57% |
| | | Mean | **0.00%** | 1.77% | 1.11% | 13.99% | 16.60% | 9.65% | 16.96% | 14.00% |
| CFLP18 | obj | Best | **1.96E+03** | 1.98E+03 | **1.96E+03** | 2.22E+03 | 2.27E+03 | 2.11E+03 | 2.38E+03 | 2.14E+03 |
| | | Mean | **1.96E+03** | 1.99E+03 | **1.96E+03** | 2.28E+03 | 2.33E+03 | 2.24E+03 | 2.42E+03 | 2.26E+03 |
| | gap | Best | **0.00%** | 0.83% | **0.00%** | 11.75% | 13.50% | 6.99% | 17.68% | 8.54% |
| | | Mean | **0.00%** | 1.35% | **0.00%** | 13.84% | 15.95% | 12.45% | 18.86% | 12.98% |
| CFLP19 | obj | Best | **2.10E+03** | 2.13E+03 | **2.10E+03** | 2.33E+03 | 2.32E+03 | 2.28E+03 | 2.44E+03 | 2.50E+03 |
| | | Mean | **2.10E+03** | 2.15E+03 | **2.10E+03** | 2.55E+03 | 2.46E+03 | 2.38E+03 | 2.51E+03 | 2.56E+03 |
| | gap | Best | **0.00%** | 1.22% | **0.00%** | 9.83% | 9.30% | 7.65% | 13.67% | 15.89% |
| | | Mean | **0.00%** | 1.93% | **0.00%** | 17.36% | 14.37% | 11.37% | 16.07% | 17.78% |
| CFLP20 | obj | Best | **2.02E+03** | **2.02E+03** | **2.02E+03** | 2.25E+03 | 2.26E+03 | 2.15E+03 | 2.40E+03 | 2.13E+03 |
| | | Mean | **2.02E+03** | 2.05E+03 | **2.02E+03** | 2.37E+03 | 2.38E+03 | 2.26E+03 | 2.52E+03 | 2.31E+03 |
| | gap | Best | **0.00%** | **0.00%** | **0.00%** | 9.91% | 10.39% | 6.00% | 15.50% | 5.06% |
| | | Mean | **0.00%** | 1.26% | **0.00%** | 14.42% | 14.86% | 10.50% | 19.58% | 12.01% |
| CFLP21 | obj | Best | **1.98E+03** | **1.98E+03** | 1.98E+03 | 2.24E+03 | 2.28E+03 | 2.24E+03 | 2.30E+03 | 2.15E+03 |
| | | Mean | **1.98E+03** | 2.01E+03 | 1.99E+03 | 2.35E+03 | 2.32E+03 | 2.34E+03 | 2.39E+03 | 2.30E+03 |
| | gap | Best | **0.00%** | **0.00%** | 0.20% | 11.66% | 13.16% | 11.69% | 13.79% | 7.76% |
| | | Mean | **0.00%** | 1.40% | 0.43% | 15.49% | 14.78% | 15.18% | 17.18% | 13.67% |
| CFLP22 | obj | Best | **1.95E+03** | **1.95E+03** | **1.95E+03** | 2.17E+03 | 2.16E+03 | 2.08E+03 | 2.28E+03 | 2.15E+03 |
| | | Mean | **1.95E+03** | 1.97E+03 | **1.95E+03** | 2.25E+03 | 2.24E+03 | 2.17E+03 | 2.38E+03 | 2.28E+03 |
| | gap | Best | **0.00%** | **0.00%** | **0.00%** | 10.44% | 9.75% | 6.54% | 14.74% | 9.57% |
| | | Mean | **0.00%** | 1.36% | **0.00%** | 13.43% | 13.17% | 10.20% | 18.02% | 14.70% |
| CFLP23 | obj | Best | **2.06E+03** | **2.06E+03** | **2.06E+03** | 2.29E+03 | 2.32E+03 | 2.21E+03 | 2.39E+03 | 2.18E+03 |
| | | Mean | **2.06E+03** | 2.07E+03 | 2.07E+03 | 2.39E+03 | 2.45E+03 | 2.27E+03 | 2.48E+03 | 2.33E+03 |
| | gap | Best | **0.00%** | **0.00%** | **0.00%** | 9.91% | 11.04% | 6.53% | 13.66% | 5.46% |
| | | Mean | **0.00%** | 0.23% | 0.19% | 13.68% | 15.63% | 9.20% | 16.75% | 11.29% |
| CFLP24 | obj | Best | **2.03E+03** | **2.03E+03** | **2.03E+03** | 2.27E+03 | 2.21E+03 | 2.23E+03 | 2.37E+03 | 2.30E+03 |
| | | Mean | **2.03E+03** | 2.05E+03 | 2.03E+03 | 2.29E+03 | 2.41E+03 | 2.29E+03 | 2.45E+03 | 2.40E+03 |
| | gap | Best | **0.00%** | **0.00%** | **0.00%** | 10.92% | 8.13% | 9.08% | 14.52% | 11.77% |
| | | Mean | **0.00%** | 1.01% | 0.01% | 11.59% | 15.62% | 11.54% | 17.33% | 15.49% |
| CFLP25 | obj | Best | **1.88E+03** | **1.88E+03** | **1.88E+03** | 2.03E+03 | 2.18E+03 | 2.01E+03 | 2.24E+03 | 2.15E+03 |
| | | Mean | **1.88E+03** | **1.88E+03** | **1.88E+03** | 2.22E+03 | 2.24E+03 | 2.17E+03 | 2.33E+03 | 2.23E+03 |

| Pro. | Metric | Status | GUROBI | OR-TOOLS | SCIP | SA | VNS | LNS | TS | GA |
|---|---|---|---|---|---|---|---|---|---|---|
| | gap | Best | **0.00%** | **0.00%** | **0.00%** | 7.05% | 13.74% | 6.25% | 16.05% | 12.25% |
| | | Mean | **0.00%** | **0.00%** | **0.00%** | 14.69% | 15.73% | 12.89% | 19.00% | 15.57% |
| CFLP26 | obj | Best | **2.07E+03** | 2.08E+03 | 2.08E+03 | 2.32E+03 | 2.46E+03 | 2.27E+03 | 2.37E+03 | 2.29E+03 |
| | | Mean | **2.07E+03** | 2.09E+03 | 2.08E+03 | 2.44E+03 | 2.52E+03 | 2.33E+03 | 2.43E+03 | 2.41E+03 |
| | gap | Best | **0.00%** | 0.30% | 0.30% | 10.63% | 15.76% | 8.91% | 12.49% | 9.40% |
| | | Mean | **0.00%** | 0.87% | 0.30% | 14.97% | 17.80% | 11.05% | 14.57% | 13.84% |
| CFLP27 | obj | Best | **1.94E+03** | **1.94E+03** | 1.94E+03 | 2.23E+03 | 2.13E+03 | 2.08E+03 | 2.14E+03 | 2.15E+03 |
| | | Mean | **1.94E+03** | **1.94E+03** | 1.94E+03 | 2.27E+03 | 2.25E+03 | 2.12E+03 | 2.25E+03 | 2.22E+03 |
| | gap | Best | **0.00%** | **0.00%** | 0.10% | 13.00% | 8.88% | 6.98% | 9.56% | 9.91% |
| | | Mean | **0.00%** | **0.00%** | 0.11% | 14.63% | 13.67% | 8.77% | 13.76% | 12.85% |
| CFLP28 | obj | Best | **1.95E+03** | **1.95E+03** | **1.95E+03** | 2.16E+03 | 2.24E+03 | 2.16E+03 | 2.31E+03 | 2.16E+03 |
| | | Mean | **1.95E+03** | **1.95E+03** | **1.95E+03** | 2.24E+03 | 2.34E+03 | 2.24E+03 | 2.36E+03 | 2.31E+03 |
| | gap | Best | **0.00%** | **0.00%** | **0.00%** | 9.75% | 13.09% | 9.93% | 15.84% | 9.97% |
| | | Mean | **0.00%** | **0.00%** | **0.00%** | 13.01% | 16.67% | 12.90% | 17.42% | 15.51% |
| CFLP29 | obj | Best | **1.96E+03** | **1.96E+03** | **1.96E+03** | 2.26E+03 | 2.28E+03 | 2.18E+03 | 2.34E+03 | 2.10E+03 |
| | | Mean | **1.96E+03** | **1.96E+03** | **1.96E+03** | 2.38E+03 | 2.35E+03 | 2.23E+03 | 2.42E+03 | 2.24E+03 |
| | gap | Best | **0.00%** | **0.00%** | **0.00%** | 13.45% | 14.10% | 10.07% | 16.35% | 6.87% |
| | | Mean | **0.00%** | **0.00%** | **0.00%** | 17.59% | 16.59% | 12.45% | 19.12% | 12.37% |
| CFLP30 | obj | Best | **1.89E+03** | **1.89E+03** | **1.89E+03** | 2.02E+03 | 2.11E+03 | 2.02E+03 | 2.13E+03 | 2.14E+03 |
| | | Mean | **1.89E+03** | **1.89E+03** | **1.89E+03** | 2.14E+03 | 2.16E+03 | 2.06E+03 | 2.27E+03 | 2.19E+03 |
| | gap | Best | **0.00%** | **0.00%** | **0.00%** | 6.18% | 10.24% | 6.48% | 11.12% | 11.38% |
| | | Mean | **0.00%** | **0.00%** | **0.00%** | 11.29% | 12.19% | 8.06% | 16.58% | 13.42% |
| CFLP31 | obj | Best | **2.04E+03** | **2.04E+03** | **2.04E+03** | 2.29E+03 | 2.26E+03 | 2.15E+03 | 2.32E+03 | 2.28E+03 |
| | | Mean | **2.04E+03** | 2.04E+03 | 2.05E+03 | 2.33E+03 | 2.34E+03 | 2.27E+03 | 2.37E+03 | 2.35E+03 |
| | gap | Best | **0.00%** | **0.00%** | **0.00%** | 10.74% | 9.58% | 4.97% | 12.04% | 10.57% |
| | | Mean | **0.00%** | 0.11% | 0.22% | 12.46% | 12.62% | 9.86% | 13.87% | 12.96% |
| CFLP32 | obj | Best | **1.94E+03** | **1.94E+03** | **1.94E+03** | 2.17E+03 | 2.31E+03 | 2.21E+03 | 2.21E+03 | 2.10E+03 |
| | | Mean | **1.94E+03** | 2.31E+03 | **1.94E+03** | 2.28E+03 | 2.46E+03 | 2.28E+03 | 2.36E+03 | 2.31E+03 |
| | gap | Best | **0.00%** | **0.00%** | **0.00%** | 10.52% | 15.90% | 12.00% | 12.12% | 7.45% |
| | | Mean | **0.00%** | 9.68% | **0.00%** | 14.56% | 20.80% | 14.65% | 17.58% | 15.70% |
| CFLP33 | obj | Best | **1.94E+03** | **1.94E+03** | **1.94E+03** | 2.10E+03 | 2.11E+03 | 2.10E+03 | 2.22E+03 | 2.05E+03 |
| | | Mean | **1.94E+03** | **1.94E+03** | **1.94E+03** | 2.26E+03 | 2.24E+03 | 2.18E+03 | 2.36E+03 | 2.23E+03 |
| | gap | Best | **0.00%** | **0.00%** | **0.00%** | 7.59% | 8.13% | 7.70% | 12.56% | 5.56% |
| | | Mean | **0.00%** | **0.00%** | **0.00%** | 14.01% | 13.07% | 10.97% | 17.53% | 12.88% |
| CFLP34 | obj | Best | **2.00E+03** | **2.00E+03** | **2.00E+03** | 2.16E+03 | 2.25E+03 | 2.18E+03 | 2.29E+03 | 2.21E+03 |
| | | Mean | **2.00E+03** | **2.00E+03** | **2.00E+03** | 2.20E+03 | 2.35E+03 | 2.27E+03 | 2.40E+03 | 2.34E+03 |
| | gap | Best | **0.00%** | **0.00%** | **0.00%** | 7.17% | 11.17% | 8.25% | 12.66% | 9.33% |
| | | Mean | **0.00%** | **0.00%** | **0.00%** | 9.00% | 14.51% | 11.62% | 16.64% | 14.30% |
| CFLP35 | obj | Best | **2.07E+03** | 2.07E+03 | **2.07E+03** | 2.33E+03 | 2.27E+03 | 2.17E+03 | 2.40E+03 | 2.35E+03 |
| | | Mean | **2.07E+03** | 2.09E+03 | **2.07E+03** | 2.47E+03 | 2.35E+03 | 2.29E+03 | 2.46E+03 | 2.42E+03 |
| | gap | Best | **0.00%** | 0.13% | **0.00%** | 11.22% | 9.07% | 4.71% | 14.03% | 12.00% |
| | | Mean | **0.00%** | 1.39% | **0.00%** | 16.38% | 12.04% | 9.57% | 15.97% | 14.63% |
| CFLP36 | obj | Best | **1.94E+03** | **1.94E+03** | **1.94E+03** | 2.21E+03 | 2.34E+03 | 2.19E+03 | 2.26E+03 | 2.23E+03 |
| | | Mean | **1.94E+03** | **1.94E+03** | **1.94E+03** | 2.27E+03 | 2.42E+03 | 2.24E+03 | 2.38E+03 | 2.38E+03 |
| | gap | Best | **0.00%** | **0.00%** | **0.00%** | 12.37% | 17.12% | 11.66% | 14.19% | 13.20% |
| | | Mean | **0.00%** | **0.00%** | **0.00%** | 14.64% | 19.68% | 13.48% | 18.30% | 18.58% |
| CFLP37 | obj | Best | **1.95E+03** | **1.95E+03** | **1.95E+03** | 2.20E+03 | 2.21E+03 | 2.17E+03 | 2.28E+03 | 2.21E+03 |

| Pro. | Metric | Status | GUROBI | OR-TOOLS | SCIP | SA | VNS | LNS | TS | GA |
|---|---|---|---|---|---|---|---|---|---|---|
| | | Mean | **1.95E+03** | **1.95E+03** | **1.95E+03** | 2.31E+03 | 2.32E+03 | 2.25E+03 | 2.38E+03 | 2.28E+03 |
| | gap | Best | **0.00%** | **0.00%** | **0.00%** | 11.09% | 11.54% | 9.89% | 14.32% | 11.62% |
| | | Mean | **0.00%** | **0.00%** | **0.00%** | 15.22% | 15.72% | 13.29% | 17.86% | 14.07% |
| CFLP38 | obj | Best | **2.01E+03** | **2.01E+03** | **2.01E+03** | 2.20E+03 | 2.28E+03 | 2.20E+03 | 2.28E+03 | 2.20E+03 |
| | | Mean | **2.01E+03** | **2.01E+03** | **2.01E+03** | 2.32E+03 | 2.35E+03 | 2.27E+03 | 2.38E+03 | 2.32E+03 |
| | gap | Best | **0.00%** | **0.00%** | **0.00%** | 8.65% | 11.90% | 8.56% | 11.58% | 8.56% |
| | | Mean | **0.00%** | **0.00%** | **0.00%** | 13.04% | 14.17% | 11.46% | 15.23% | 13.03% |
| CFLP39 | obj | Best | **1.96E+03** | **1.96E+03** | **1.96E+03** | 2.14E+03 | 2.14E+03 | 2.09E+03 | 2.12E+03 | 2.17E+03 |
| | | Mean | **1.96E+03** | **1.96E+03** | **1.96E+03** | 2.25E+03 | 2.38E+03 | 2.16E+03 | 2.27E+03 | 2.29E+03 |
| | gap | Best | **0.00%** | **0.00%** | **0.00%** | 8.24% | 8.25% | 6.27% | 7.70% | 9.64% |
| | | Mean | **0.00%** | **0.00%** | **0.00%** | 12.53% | 17.18% | 9.12% | 13.47% | 14.41% |
| CFLP40 | obj | Best | **1.99E+03** | **1.99E+03** | **1.99E+03** | 2.17E+03 | 2.27E+03 | 2.14E+03 | 2.29E+03 | 2.17E+03 |
| | | Mean | **1.99E+03** | **1.99E+03** | **1.99E+03** | 2.34E+03 | 2.34E+03 | 2.23E+03 | 2.40E+03 | 2.29E+03 |
| | gap | Best | **0.00%** | **0.00%** | **0.00%** | 8.25% | 12.27% | 7.05% | 12.96% | 8.11% |
| | | Mean | **0.00%** | **0.00%** | **0.00%** | 14.57% | 14.74% | 10.61% | 16.74% | 12.76% |

## 3.5 Bin packing problem with conflicts (BPPC)

The relevant experimental results on BPPC are presented in Table S-15.

**Table S-15** Experimental results on BPPC test suit.

| Pro. | Metric | Status | GUROBI | OR-TOOLS | SCIP | SA | VNS | LNS | TS | GA |
|---|---|---|---|---|---|---|---|---|---|---|
| BPPC01 | obj | Best | NAN | **1.06E+02** | 1.09E+02 | **1.06E+02** | **1.06E+02** | **1.06E+02** | **1.06E+02** | 1.07E+02 |
| | | Mean | NAN | **1.06E+02** | 1.09E+02 | 1.07E+02 | 1.07E+02 | 1.07E+02 | 1.07E+02 | 1.07E+02 |
| | gap | Best | NAN | 31.13% | 33.03% | 31.13% | 31.13% | 31.13% | 31.13% | 31.78% |
| | | Mean | NAN | **31.26%** | 33.03% | 31.65% | 31.52% | 31.65% | 31.52% | 31.78% |
| BPPC02 | obj | Best | NAN | **1.05E+02** | 1.11E+02 | 1.06E+02 | 1.06E+02 | **1.05E+02** | **1.05E+02** | **1.05E+02** |
| | | Mean | NAN | **1.06E+02** | 1.11E+02 | 1.06E+02 | 1.06E+02 | **1.06E+02** | 1.06E+02 | 1.06E+02 |
| | gap | Best | NAN | **2.86%** | 8.11% | 3.77% | 3.77% | **2.86%** | **2.86%** | **2.86%** |
| | | Mean | NAN | **3.41%** | 8.11% | 4.13% | 3.77% | **3.41%** | 3.95% | 3.95% |
| BPPC03 | obj | Best | NAN | **1.04E+02** | 1.08E+02 | 1.05E+02 | **1.04E+02** | **1.04E+02** | 1.05E+02 | 1.05E+02 |
| | | Mean | NAN | **1.04E+02** | 1.08E+02 | 1.05E+02 | 1.05E+02 | 1.04E+02 | 1.05E+02 | 1.05E+02 |
| | gap | Best | NAN | **6.73%** | 10.19% | 7.62% | **6.73%** | **6.73%** | 7.62% | 7.62% |
| | | Mean | NAN | **6.73%** | 10.19% | 7.79% | 7.44% | 7.09% | 7.97% | 7.97% |
| BPPC04 | obj | Best | NAN | **1.05E+02** | 1.10E+02 | 1.06E+02 | **1.05E+02** | 1.06E+02 | 1.06E+02 | 1.07E+02 |
| | | Mean | NAN | **1.05E+02** | 1.10E+02 | 1.07E+02 | 1.06E+02 | 1.06E+02 | 1.07E+02 | 1.08E+02 |
| | gap | Best | NAN | **4.76%** | 9.09% | 5.66% | **4.76%** | 5.66% | 5.66% | 6.54% |
| | | Mean | NAN | **4.76%** | 9.09% | 6.54% | 5.66% | 5.84% | 6.19% | 7.06% |
| BPPC05 | obj | Best | NAN | **1.18E+02** | 1.23E+02 | 1.22E+02 | 1.22E+02 | 1.20E+02 | 1.22E+02 | 1.21E+02 |
| | | Mean | NAN | **1.18E+02** | 1.23E+02 | 1.23E+02 | 1.22E+02 | 1.21E+02 | 1.24E+02 | 1.24E+02 |
| | gap | Best | NAN | **44.92%** | 47.15% | 46.72% | 46.72% | 45.83% | 46.72% | 46.28% |
| | | Mean | NAN | **45.10%** | 47.15% | 47.15% | 46.89% | 46.28% | 47.65% | 47.49% |
| BPPC06 | obj | Best | NAN | **1.32E+02** | 1.38E+02 | 1.34E+02 | 1.34E+02 | 1.33E+02 | 1.34E+02 | 1.36E+02 |
| | | Mean | NAN | **1.33E+02** | 1.38E+02 | 1.36E+02 | 1.35E+02 | 1.34E+02 | 1.35E+02 | 1.36E+02 |
| | gap | Best | NAN | **93.94%** | 94.20% | 94.03% | 94.03% | 93.98% | 94.03% | 94.12% |
| | | Mean | NAN | **93.98%** | 94.20% | 94.10% | 94.08% | 94.04% | 94.09% | 94.13% |
| BPPC07 | obj | Best | NAN | **1.66E+02** | 1.70E+02 | 1.69E+02 | 1.69E+02 | 1.68E+02 | 1.70E+02 | 1.71E+02 |

| Pro. | Metric | Status | GUROBI | OR-TOOLS | SCIP | SA | VNS | LNS | TS | GA |
|---|---|---|---|---|---|---|---|---|---|---|
| | | Mean | NAN | **1.67E+02** | 1.70E+02 | 1.70E+02 | 1.70E+02 | 1.69E+02 | 1.71E+02 | 1.71E+02 |
| | gap | Best | NAN | **93.98%** | 94.12% | 94.08% | 94.08% | 94.05% | 94.12% | 94.15% |
| | | Mean | NAN | **94.00%** | 94.12% | 94.10% | 94.11% | 94.07% | 94.16% | 94.17% |
| BPPC08 | obj | Best | NAN | **1.78E+02** | 1.82E+02 | 1.80E+02 | 1.80E+02 | **1.78E+02** | 1.81E+02 | 1.81E+02 |
| | | Mean | NAN | **1.79E+02** | 1.82E+02 | 1.81E+02 | 1.81E+02 | **1.79E+02** | 1.82E+02 | 1.82E+02 |
| | gap | Best | NAN | **98.31%** | 98.35% | 98.33% | 98.33% | **98.31%** | 98.34% | 98.34% |
| | | Mean | NAN | **98.33%** | 98.35% | 98.34% | 98.34% | **98.33%** | 98.35% | 98.35% |
| BPPC09 | obj | Best | NAN | **2.05E+02** | 2.07E+02 | **2.05E+02** | **2.05E+02** | **2.05E+02** | **2.05E+02** | **2.05E+02** |
| | | Mean | NAN | 2.05E+02 | 2.07E+02 | **2.05E+02** | **2.05E+02** | **2.05E+02** | 2.05E+02 | 2.06E+02 |
| | gap | Best | NAN | **97.07%** | 97.10% | **97.07%** | **97.07%** | **97.07%** | **97.07%** | **97.07%** |
| | | Mean | NAN | 97.08% | 97.10% | **97.07%** | **97.07%** | **97.07%** | 97.08% | 97.08% |
| BPPC10 | obj | Best | NAN | **2.29E+02** | 2.32E+02 | **2.29E+02** | 2.30E+02 | **2.29E+02** | 2.30E+02 | 2.30E+02 |
| | | Mean | NAN | 2.30E+02 | 2.32E+02 | **2.29E+02** | 2.30E+02 | 2.30E+02 | 2.30E+02 | 2.31E+02 |
| | gap | Best | NAN | **92.58%** | 92.67% | **92.58%** | 92.61% | **92.58%** | 92.61% | 92.61% |
| | | Mean | NAN | 92.61% | 92.67% | **92.58%** | 92.62% | 92.60% | 92.62% | 92.63% |
| BPPC11 | obj | Best | NAN | **2.13E+02** | 2.19E+02 | 2.15E+02 | 2.14E+02 | 2.14E+02 | 2.16E+02 | 2.14E+02 |
| | | Mean | NAN | **2.15E+02** | NAN | 2.16E+02 | 2.15E+02 | **2.15E+02** | 2.17E+02 | 2.16E+02 |
| | gap | Best | NAN | **66.20%** | 67.12% | 66.51% | 66.36% | 66.36% | 66.67% | 66.36% |
| | | Mean | NAN | **66.48%** | NAN | 66.64% | 66.54% | **66.48%** | 66.79% | 66.67% |
| BPPC12 | obj | Best | NAN | 2.15E+02 | 2.33E+02 | 2.14E+02 | 2.14E+02 | **2.12E+02** | 2.13E+02 | 2.14E+02 |
| | | Mean | NAN | 2.15E+02 | 2.39E+02 | 2.14E+02 | 2.14E+02 | **2.13E+02** | 2.14E+02 | 2.15E+02 |
| | gap | Best | NAN | 52.56% | 56.22% | 52.34% | 52.34% | **51.89%** | 52.11% | 52.34% |
| | | Mean | NAN | 52.56% | 57.39% | 52.38% | 52.34% | **52.02%** | 52.38% | 52.47% |
| BPPC13 | obj | Best | NAN | **2.14E+02** | 2.63E+02 | **2.16E+02** | **2.15E+02** | **2.14E+02** | **2.16E+02** | 2.17E+02 |
| | | Mean | NAN | **2.15E+02** | 2.63E+02 | 2.17E+02 | **2.16E+02** | **2.15E+02** | 2.17E+02 | 2.18E+02 |
| | gap | Best | NAN | **99.07%** | 99.24% | **99.07%** | **99.07%** | **99.07%** | **99.07%** | 99.08% |
| | | Mean | NAN | **99.07%** | 99.24% | 99.08% | **99.07%** | **99.07%** | 99.08% | 99.08% |
| BPPC14 | obj | Best | NAN | 2.19E+02 | 2.22E+02 | 2.19E+02 | 2.19E+02 | **2.17E+02** | 2.19E+02 | 2.20E+02 |
| | | Mean | NAN | 2.20E+02 | 2.22E+02 | 2.20E+02 | 2.20E+02 | **2.18E+02** | 2.21E+02 | 2.21E+02 |
| | gap | Best | NAN | 95.89% | 95.95% | 95.89% | 95.89% | **95.85%** | 95.89% | 95.91% |
| | | Mean | NAN | 95.90% | 95.95% | 95.91% | 95.91% | **95.87%** | 95.92% | 95.93% |
| BPPC15 | obj | Best | NAN | 2.28E+02 | 2.33E+02 | 2.29E+02 | 2.28E+02 | **2.25E+02** | 2.27E+02 | 2.30E+02 |
| | | Mean | NAN | 2.29E+02 | 2.33E+02 | 2.30E+02 | 2.29E+02 | **2.26E+02** | 2.28E+02 | 2.33E+02 |
| | gap | Best | NAN | 78.95% | 79.40% | 79.04% | 78.95% | **78.67%** | 78.85% | 79.13% |
| | | Mean | NAN | 79.02% | 79.40% | 79.09% | 79.04% | **78.78%** | 78.97% | 79.43% |
| BPPC16 | obj | Best | NAN | 2.52E+02 | 2.57E+02 | 2.55E+02 | 2.53E+02 | **2.50E+02** | 2.50E+02 | 2.58E+02 |
| | | Mean | NAN | 2.53E+02 | 2.57E+02 | 2.56E+02 | 2.54E+02 | **2.51E+02** | 2.53E+02 | 2.60E+02 |
| | gap | Best | NAN | 94.44% | 94.55% | 94.51% | 94.47% | **94.40%** | 94.40% | 94.57% |
| | | Mean | NAN | 94.46% | 94.55% | 94.53% | 94.49% | **94.42%** | 94.47% | 94.61% |
| BPPC17 | obj | Best | NAN | 3.02E+02 | 3.07E+02 | 3.01E+02 | 3.02E+02 | **2.99E+02** | 3.03E+02 | 3.04E+02 |
| | | Mean | NAN | 3.03E+02 | NAN | 3.03E+02 | 3.02E+02 | **3.00E+02** | 3.03E+02 | 3.06E+02 |
| | gap | Best | NAN | 97.35% | 97.39% | 97.34% | 97.35% | **97.32%** | 97.36% | 97.37% |
| | | Mean | NAN | 97.36% | NAN | 97.36% | 97.35% | **97.34%** | 97.36% | 97.38% |
| BPPC18 | obj | Best | NAN | **3.43E+02** | 3.55E+02 | 3.47E+02 | 3.46E+02 | 3.46E+02 | 3.49E+02 | 3.51E+02 |
| | | Mean | NAN | **3.47E+02** | 3.55E+02 | 3.49E+02 | 3.49E+02 | **3.47E+02** | 3.50E+02 | 3.53E+02 |
| | gap | Best | NAN | **95.34%** | 95.49% | 95.39% | 95.38% | 95.38% | 95.42% | 95.44% |

| Pro. | Metric | Status | GUROBI | OR-TOOLS | SCIP | SA | VNS | LNS | TS | GA |
|---|---|---|---|---|---|---|---|---|---|---|
| | | Mean | NAN | **95.39%** | 95.49% | 95.41% | 95.42% | **95.39%** | 95.43% | 95.47% |
| BPPC19 | obj | Best | NAN | **4.04E+02** | 4.10E+02 | **4.05E+02** | **4.05E+02** | **4.04E+02** | **4.05E+02** | **4.06E+02** |
| | | Mean | NAN | **4.04E+02** | 4.10E+02 | **4.06E+02** | **4.06E+02** | **4.05E+02** | **4.07E+02** | 4.09E+02 |
| | gap | Best | NAN | **99.26%** | 99.27% | **99.26%** | **99.26%** | **99.26%** | **99.26%** | **99.26%** |
| | | Mean | NAN | **99.26%** | 99.27% | **99.26%** | **99.26%** | **99.26%** | **99.26%** | 99.27% |
| BPPC20 | obj | Best | NAN | **4.59E+02** | NAN | **4.59E+02** | **4.59E+02** | **4.59E+02** | 4.60E+02 | 4.60E+02 |
| | | Mean | NAN | **4.60E+02** | NAN | **4.60E+02** | **4.60E+02** | **4.60E+02** | 4.60E+02 | 4.61E+02 |
| | gap | Best | NAN | **91.94%** | NAN | **91.94%** | **91.94%** | **91.94%** | 91.96% | 91.96% |
| | | Mean | NAN | **91.96%** | NAN | **91.96%** | **91.96%** | **91.96%** | 91.96% | 91.98% |
| BPPC21 | obj | Best | 2.10E+01 | **2.00E+01** | **2.00E+01** | 2.10E+01 | 2.10E+01 | 2.10E+01 | 2.20E+01 | 2.20E+01 |
| | | Mean | 2.10E+01 | **2.00E+01** | **2.00E+01** | 2.16E+01 | 2.18E+01 | 2.12E+01 | 2.20E+01 | 2.20E+01 |
| | gap | Best | 4.76% | **0.00%** | **0.00%** | 4.76% | 4.76% | 4.76% | 9.09% | 9.09% |
| | | Mean | 4.76% | **0.00%** | **0.00%** | 7.36% | 8.23% | 5.63% | 9.09% | 9.09% |
| BPPC22 | obj | Best | **2.10E+01** | **2.10E+01** | **2.10E+01** | **2.10E+01** | **2.10E+01** | **2.10E+01** | **2.10E+01** | **2.10E+01** |
| | | Mean | **2.10E+01** | **2.10E+01** | **2.10E+01** | 2.18E+01 | 2.18E+01 | 2.12E+01 | 2.16E+01 | 2.18E+01 |
| | gap | Best | **4.76%** | **4.76%** | **4.76%** | **4.76%** | **4.76%** | **4.76%** | **4.76%** | **4.76%** |
| | | Mean | **4.76%** | **4.76%** | **4.76%** | 8.23% | 8.23% | 5.63% | 7.36% | 8.23% |
| BPPC23 | obj | Best | **2.10E+01** | **2.10E+01** | 2.20E+01 | **2.10E+01** | 2.20E+01 | **2.10E+01** | 2.20E+01 | **2.10E+01** |
| | | Mean | **2.10E+01** | **2.10E+01** | 2.22E+01 | 2.18E+01 | 2.20E+01 | 2.12E+01 | 2.20E+01 | 2.18E+01 |
| | gap | Best | **4.76%** | **4.76%** | 9.09% | **4.76%** | 9.09% | **4.76%** | 9.09% | **4.76%** |
| | | Mean | **4.76%** | **4.76%** | 9.88% | 8.23% | 9.09% | 5.63% | 9.09% | 8.23% |
| BPPC24 | obj | Best | **2.10E+01** | **2.10E+01** | 2.20E+01 | 2.20E+01 | **2.10E+01** | **2.10E+01** | 2.20E+01 | **2.10E+01** |
| | | Mean | **2.10E+01** | **2.10E+01** | 2.20E+01 | 2.20E+01 | 2.18E+01 | 2.12E+01 | 2.20E+01 | 2.18E+01 |
| | gap | Best | **4.76%** | **4.76%** | 9.09% | 9.09% | **4.76%** | **4.76%** | 9.09% | **4.76%** |
| | | Mean | **4.76%** | **4.76%** | 9.09% | 9.09% | 8.23% | 5.63% | 9.09% | 8.23% |
| BPPC25 | obj | Best | **2.20E+01** | **2.20E+01** | 2.30E+01 | **2.20E+01** | **2.20E+01** | **2.20E+01** | **2.20E+01** | **2.20E+01** |
| | | Mean | **2.20E+01** | **2.20E+01** | 2.30E+01 | 2.26E+01 | 2.24E+01 | **2.20E+01** | 2.26E+01 | 2.26E+01 |
| | gap | Best | **0.00%** | **0.00%** | 4.35% | **0.00%** | **0.00%** | **0.00%** | **0.00%** | **0.00%** |
| | | Mean | **0.00%** | **0.00%** | 4.35% | 2.61% | 1.74% | **0.00%** | 2.61% | 2.61% |
| BPPC26 | obj | Best | NAN | **2.70E+01** | 2.80E+01 | **2.70E+01** | **2.70E+01** | **2.70E+01** | **2.70E+01** | **2.70E+01** |
| | | Mean | NAN | **2.70E+01** | 2.80E+01 | 2.72E+01 | 2.74E+01 | 2.74E+01 | 2.72E+01 | 2.78E+01 |
| | gap | Best | NAN | **3.70%** | 7.14% | **3.70%** | **3.70%** | **3.70%** | **3.70%** | **3.70%** |
| | | Mean | NAN | **3.70%** | 7.14% | 4.39% | 5.08% | 5.08% | 4.39% | 6.46% |
| BPPC27 | obj | Best | NAN | **4.30E+01** | 4.40E+01 | **4.30E+01** | **4.30E+01** | **4.30E+01** | **4.30E+01** | **4.30E+01** |
| | | Mean | NAN | **4.30E+01** | 4.40E+01 | **4.30E+01** | **4.30E+01** | **4.30E+01** | **4.30E+01** | **4.30E+01** |
| | gap | Best | NAN | **2.33%** | 4.55% | **2.33%** | **2.33%** | **2.33%** | **2.33%** | **2.33%** |
| | | Mean | NAN | **2.33%** | 4.55% | **2.33%** | **2.33%** | **2.33%** | **2.33%** | **2.33%** |
| BPPC28 | obj | Best | NAN | **4.10E+01** | 4.20E+01 | **4.10E+01** | **4.10E+01** | **4.10E+01** | **4.10E+01** | **4.10E+01** |
| | | Mean | NAN | **4.10E+01** | 4.20E+01 | **4.10E+01** | **4.10E+01** | **4.10E+01** | **4.10E+01** | **4.10E+01** |
| | gap | Best | NAN | **0.00%** | 2.38% | **0.00%** | **0.00%** | **0.00%** | **0.00%** | **0.00%** |
| | | Mean | NAN | **0.00%** | 2.38% | **0.00%** | **0.00%** | **0.00%** | **0.00%** | **0.00%** |
| BPPC29 | obj | Best | NAN | **4.60E+01** | 4.70E+01 | **4.60E+01** | **4.60E+01** | **4.60E+01** | **4.60E+01** | **4.60E+01** |
| | | Mean | NAN | **4.60E+01** | 4.70E+01 | **4.60E+01** | **4.60E+01** | **4.60E+01** | 4.62E+01 | 4.62E+01 |
| | gap | Best | NAN | **0.00%** | 2.13% | **0.00%** | **0.00%** | **0.00%** | **0.00%** | **0.00%** |
| | | Mean | NAN | **0.00%** | 2.13% | **0.00%** | **0.00%** | **0.00%** | 0.43% | 0.43% |
| BPPC30 | obj | Best | NAN | **5.60E+01** | **5.60E+01** | **5.60E+01** | **5.60E+01** | **5.60E+01** | **5.60E+01** | **5.60E+01** |

| Pro. | Metric | Status | GUROBI | OR-TOOLS | SCIP | SA | VNS | LNS | TS | GA |
|---|---|---|---|---|---|---|---|---|---|---|
| | | Mean | NAN | **5.60E+01** | **5.60E+01** | **5.60E+01** | **5.60E+01** | **5.60E+01** | **5.60E+01** | **5.60E+01** |
| | gap | Best | NAN | **7.14%** | **7.14%** | **7.14%** | **7.14%** | **7.14%** | **7.14%** | **7.14%** |
| | | Mean | NAN | **7.14%** | **7.14%** | **7.14%** | **7.14%** | **7.14%** | **7.14%** | **7.14%** |
| BPPC31 | obj | Best | 4.10E+01 | **4.00E+01** | **4.00E+01** | 4.30E+01 | 4.30E+01 | 4.20E+01 | 4.20E+01 | 4.30E+01 |
| | | Mean | NAN | **4.00E+01** | **4.00E+01** | 4.32E+01 | 4.30E+01 | 4.24E+01 | 4.34E+01 | 4.30E+01 |
| | gap | Best | 2.44% | **0.00%** | **0.00%** | 6.98% | 6.98% | 4.76% | 4.76% | 6.98% |
| | | Mean | NAN | **0.00%** | **0.00%** | 7.40% | 6.98% | 5.65% | 7.80% | 6.98% |
| BPPC32 | obj | Best | 4.10E+01 | **4.10E+01** | 4.50E+01 | 4.30E+01 | 4.30E+01 | 4.20E+01 | 4.30E+01 | 4.30E+01 |
| | | Mean | 4.16E+01 | **4.10E+01** | 4.50E+01 | 4.34E+01 | 4.30E+01 | 4.26E+01 | 4.30E+01 | 4.36E+01 |
| | gap | Best | 2.44% | **2.44%** | 11.11% | 6.98% | 6.98% | 4.76% | 6.98% | 6.98% |
| | | Mean | 3.83% | **2.44%** | 11.11% | 7.82% | 6.98% | 6.09% | 6.98% | 8.25% |
| BPPC33 | obj | Best | NAN | **4.10E+01** | 4.40E+01 | 4.30E+01 | 4.30E+01 | 4.20E+01 | 4.30E+01 | 4.30E+01 |
| | | Mean | NAN | **4.16E+01** | 4.40E+01 | 4.32E+01 | 4.30E+01 | 4.24E+01 | 4.34E+01 | 4.32E+01 |
| | gap | Best | NAN | **2.44%** | 9.09% | 6.98% | 6.98% | 4.76% | 6.98% | 6.98% |
| | | Mean | NAN | **3.83%** | 9.09% | 7.40% | 6.98% | 5.65% | 7.82% | 7.40% |
| BPPC34 | obj | Best | NAN | **4.20E+01** | 4.50E+01 | 4.40E+01 | 4.30E+01 | 4.30E+01 | 4.30E+01 | 4.30E+01 |
| | | Mean | NAN | **4.20E+01** | 4.50E+01 | 4.40E+01 | 4.34E+01 | 4.30E+01 | 4.36E+01 | 4.40E+01 |
| | gap | Best | NAN | **4.76%** | 11.11% | 9.09% | 6.98% | 6.98% | 6.98% | 6.98% |
| | | Mean | NAN | **4.76%** | 11.11% | 9.09% | 7.82% | 6.98% | 8.25% | 9.07% |
| BPPC35 | obj | Best | NAN | **5.10E+01** | 5.30E+01 | **5.10E+01** | **5.10E+01** | **5.10E+01** | **5.10E+01** | **5.10E+01** |
| | | Mean | NAN | **5.10E+01** | 5.30E+01 | **5.10E+01** | 5.14E+01 | **5.10E+01** | 5.16E+01 | 5.16E+01 |
| | gap | Best | NAN | **21.57%** | 24.53% | **21.57%** | **21.57%** | **21.57%** | **21.57%** | **21.57%** |
| | | Mean | NAN | **21.57%** | 24.53% | **21.57%** | 22.17% | **21.57%** | 22.46% | 22.47% |
| BPPC36 | obj | Best | 6.30E+01 | **5.80E+01** | 6.30E+01 | **5.80E+01** | **5.80E+01** | **5.80E+01** | 5.90E+01 | **5.80E+01** |
| | | Mean | 6.30E+01 | **5.80E+01** | 6.30E+01 | 5.88E+01 | 5.94E+01 | 5.84E+01 | 5.94E+01 | 5.92E+01 |
| | gap | Best | 36.51% | **31.03%** | 36.51% | **31.03%** | **31.03%** | **31.03%** | 32.20% | **31.03%** |
| | | Mean | 36.51% | **31.03%** | 36.51% | 31.97% | 32.65% | 31.50% | 32.66% | 32.42% |
| BPPC37 | obj | Best | NAN | **7.70E+01** | 7.90E+01 | **7.70E+01** | **7.70E+01** | **7.70E+01** | **7.70E+01** | **7.70E+01** |
| | | Mean | NAN | **7.70E+01** | 7.90E+01 | **7.70E+01** | **7.70E+01** | **7.70E+01** | 7.78E+01 | 7.72E+01 |
| | gap | Best | NAN | **48.05%** | 49.37% | **48.05%** | **48.05%** | **48.05%** | **48.05%** | **48.05%** |
| | | Mean | NAN | **48.05%** | 49.37% | **48.05%** | **48.05%** | **48.05%** | 48.58% | 48.19% |
| BPPC38 | obj | Best | NAN | **8.20E+01** | 8.50E+01 | 8.30E+01 | 8.30E+01 | 8.30E+01 | 8.30E+01 | 8.40E+01 |
| | | Mean | NAN | **8.26E+01** | 8.50E+01 | 8.30E+01 | 8.30E+01 | 8.32E+01 | 8.32E+01 | 8.40E+01 |
| | gap | Best | NAN | **52.44%** | 54.12% | 53.01% | 53.01% | 53.01% | 53.01% | 53.57% |
| | | Mean | NAN | **52.78%** | 54.12% | 53.01% | 53.01% | 53.12% | 53.12% | 53.57% |
| BPPC39 | obj | Best | NAN | 1.02E+02 | 1.04E+02 | 1.02E+02 | 1.02E+02 | 1.02E+02 | 1.02E+02 | 1.03E+02 |
| | | Mean | NAN | 1.02E+02 | 1.04E+02 | 1.02E+02 | 1.02E+02 | 1.02E+02 | 1.02E+02 | 1.03E+02 |
| | gap | Best | NAN | 59.80% | 60.58% | 59.80% | 59.80% | 59.80% | 59.80% | 60.19% |
| | | Mean | NAN | 59.80% | 60.58% | 59.88% | 59.80% | 59.80% | 59.88% | 60.19% |
| BPPC40 | obj | Best | NAN | **1.11E+02** | 1.12E+02 | **1.11E+02** | **1.11E+02** | **1.11E+02** | **1.11E+02** | 1.12E+02 |
| | | Mean | NAN | **1.11E+02** | 1.12E+02 | **1.11E+02** | 1.11E+02 | **1.11E+02** | 1.11E+02 | 1.12E+02 |
| | gap | Best | NAN | **59.46%** | 59.82% | **59.46%** | **59.46%** | **59.46%** | **59.46%** | 59.82% |
| | | Mean | NAN | **59.46%** | 59.82% | **59.46%** | 59.53% | **59.46%** | 59.60% | 59.82% |
| BPPC41 | obj | Best | NAN | **8.30E+01** | 8.30E+01 | 9.00E+01 | 8.80E+01 | 8.70E+01 | 8.90E+01 | 9.00E+01 |
| | | Mean | NAN | **8.30E+01** | 8.30E+01 | 9.02E+01 | 8.90E+01 | 8.76E+01 | 8.98E+01 | 9.00E+01 |
| | gap | Best | NAN | **0.00%** | NAN | 7.78% | 5.68% | 4.60% | 6.74% | 7.78% |

| Pro. | Metric | Status | GUROBI | OR-TOOLS | SCIP | SA | VNS | LNS | TS | GA |
|---|---|---|---|---|---|---|---|---|---|---|
| | | Mean | NAN | **0.00%** | NAN | 7.98% | 6.74% | 5.25% | 7.57% | 7.78% |
| BPPC42 | obj | Best | NAN | **8.50E+01** | **8.50E+01** | 8.90E+01 | 8.90E+01 | 8.80E+01 | 8.90E+01 | 8.90E+01 |
| | | Mean | NAN | **8.50E+01** | **8.50E+01** | 9.02E+01 | 8.92E+01 | 8.82E+01 | 9.04E+01 | 9.00E+01 |
| | gap | Best | NAN | **3.53%** | **3.53%** | 7.87% | 7.87% | 6.82% | 7.87% | 7.87% |
| | | Mean | NAN | **3.53%** | **3.53%** | 9.08% | 8.07% | 7.03% | 9.28% | 8.88% |
| BPPC43 | obj | Best | NAN | **8.60E+01** | 9.40E+01 | 8.90E+01 | 8.90E+01 | 8.70E+01 | 9.00E+01 | 9.00E+01 |
| | | Mean | NAN | **8.68E+01** | 9.96E+01 | 9.00E+01 | 8.94E+01 | 8.78E+01 | 9.06E+01 | 9.02E+01 |
| | gap | Best | NAN | **3.49%** | 11.70% | 6.74% | 6.74% | 4.60% | 7.78% | 7.78% |
| | | Mean | NAN | **4.38%** | 16.60% | 7.77% | 7.16% | 5.46% | 8.39% | 7.98% |
| BPPC44 | obj | Best | NAN | **8.80E+01** | 9.10E+01 | 9.00E+01 | 9.00E+01 | **8.80E+01** | 9.10E+01 | 9.10E+01 |
| | | Mean | NAN | **8.82E+01** | 9.10E+01 | 9.00E+01 | 9.04E+01 | 8.88E+01 | 9.14E+01 | 9.14E+01 |
| | gap | Best | NAN | **6.82%** | 9.89% | 8.89% | 8.89% | **6.82%** | 9.89% | 9.89% |
| | | Mean | NAN | **7.03%** | 9.89% | 8.89% | 9.29% | 7.66% | 10.28% | 10.28% |
| BPPC45 | obj | Best | NAN | **9.90E+01** | 1.03E+02 | 1.02E+02 | 1.01E+02 | 1.01E+02 | 1.01E+02 | 1.02E+02 |
| | | Mean | NAN | **1.00E+02** | 1.03E+02 | 1.03E+02 | 1.02E+02 | 1.02E+02 | 1.03E+02 | 1.03E+02 |
| | gap | Best | NAN | **87.88%** | 88.35% | 88.24% | 88.12% | 88.12% | 88.12% | 88.24% |
| | | Mean | NAN | **88.00%** | 88.35% | 88.30% | 88.26% | 88.19% | 88.30% | 88.33% |
| BPPC46 | obj | Best | NAN | **1.34E+02** | 1.39E+02 | 1.34E+02 | **1.34E+02** | **1.34E+02** | **1.34E+02** | 1.35E+02 |
| | | Mean | NAN | **1.34E+02** | 1.39E+02 | 1.35E+02 | **1.34E+02** | **1.34E+02** | **1.34E+02** | 1.36E+02 |
| | gap | Best | NAN | **71.64%** | 72.66% | 71.64% | **71.64%** | **71.64%** | **71.64%** | 71.85% |
| | | Mean | NAN | **71.68%** | 72.66% | 71.81% | **71.68%** | **71.68%** | **71.68%** | 72.02% |
| BPPC47 | obj | Best | NAN | **1.58E+02** | 1.59E+02 | 1.59E+02 | 1.59E+02 | **1.58E+02** | 1.59E+02 | 1.60E+02 |
| | | Mean | NAN | **1.58E+02** | 1.59E+02 | 1.60E+02 | 1.60E+02 | 1.59E+02 | 1.60E+02 | 1.61E+02 |
| | gap | Best | NAN | **89.87%** | 89.94% | 89.94% | 89.94% | **89.87%** | 89.94% | 90.00% |
| | | Mean | NAN | **89.87%** | 89.94% | 89.97% | 89.97% | 89.92% | 90.02% | 90.06% |
| BPPC48 | obj | Best | NAN | **1.73E+02** | 1.77E+02 | 1.75E+02 | 1.75E+02 | 1.74E+02 | 1.75E+02 | 1.75E+02 |
| | | Mean | NAN | **1.74E+02** | 1.77E+02 | 1.76E+02 | 1.76E+02 | 1.75E+02 | 1.76E+02 | 1.78E+02 |
| | gap | Best | NAN | **90.17%** | 90.40% | 90.29% | 90.29% | 90.23% | 90.29% | 90.29% |
| | | Mean | NAN | **90.23%** | 90.40% | 90.32% | 90.33% | 90.31% | 90.33% | 90.43% |
| BPPC49 | obj | Best | NAN | **1.97E+02** | 2.00E+02 | 1.98E+02 | 1.98E+02 | 1.98E+02 | 1.99E+02 | 1.99E+02 |
| | | Mean | NAN | **1.98E+02** | 2.00E+02 | 1.98E+02 | 1.99E+02 | 1.98E+02 | 1.99E+02 | 2.00E+02 |
| | gap | Best | NAN | **87.82%** | 88.00% | 87.88% | 87.88% | 87.88% | 87.94% | 87.94% |
| | | Mean | NAN | **87.87%** | 88.00% | 87.90% | 87.92% | 87.89% | 87.96% | 87.99% |
| BPPC50 | obj | Best | NAN | **2.28E+02** | **2.28E+02** | **2.28E+02** | **2.28E+02** | **2.28E+02** | **2.28E+02** | **2.28E+02** |
| | | Mean | NAN | **2.28E+02** | **2.28E+02** | **2.28E+02** | **2.28E+02** | **2.28E+02** | **2.28E+02** | **2.28E+02** |
| | gap | Best | NAN | **90.35%** | **90.35%** | **90.35%** | **90.35%** | **90.35%** | **90.35%** | **90.35%** |
| | | Mean | NAN | **90.35%** | **90.35%** | **90.35%** | **90.35%** | **90.35%** | **90.35%** | **90.35%** |
| BPPC51 | obj | Best | NAN | **1.67E+02** | **1.67E+02** | 1.79E+02 | 1.79E+02 | 1.76E+02 | 1.81E+02 | 1.81E+02 |
| | | Mean | NAN | **1.67E+02** | NAN | 1.81E+02 | 1.80E+02 | 1.76E+02 | 1.82E+02 | 1.81E+02 |
| | gap | Best | NAN | **0.60%** | **0.60%** | 7.26% | 7.26% | 5.68% | 8.29% | 8.29% |
| | | Mean | NAN | **0.60%** | NAN | 8.08% | 7.78% | 5.89% | 8.59% | 8.49% |
| BPPC52 | obj | Best | NAN | **1.71E+02** | 2.02E+02 | 1.81E+02 | 1.79E+02 | 1.76E+02 | 1.82E+02 | 1.81E+02 |
| | | Mean | NAN | **1.71E+02** | 2.02E+02 | 1.82E+02 | 1.80E+02 | 1.77E+02 | 1.83E+02 | 1.82E+02 |
| | gap | Best | NAN | **21.64%** | 33.66% | 25.97% | 25.14% | 23.86% | 26.37% | 25.97% |
| | | Mean | NAN | **21.82%** | 33.66% | 26.45% | 25.47% | 24.21% | 26.62% | 26.37% |
| BPPC53 | obj | Best | NAN | **1.75E+02** | 2.21E+02 | 1.80E+02 | 1.79E+02 | **1.75E+02** | 1.82E+02 | 1.81E+02 |

| Pro. | Metric | Status | GUROBI | OR-TOOLS | SCIP | SA | VNS | LNS | TS | GA |
|---|---|---|---|---|---|---|---|---|---|---|
| | | Mean | NAN | **1.75E+02** | 2.21E+02 | 1.82E+02 | 1.80E+02 | 1.76E+02 | 1.83E+02 | 1.82E+02 |
| | gap | Best | NAN | **46.86%** | 57.92% | 48.33% | 48.04% | **46.86%** | 48.90% | 48.62% |
| | | Mean | NAN | **46.92%** | 57.92% | 48.79% | 48.27% | 47.28% | 49.18% | 48.96% |
| BPPC54 | obj | Best | NAN | **1.77E+02** | 1.84E+02 | 1.82E+02 | 1.82E+02 | **1.77E+02** | 1.84E+02 | 1.83E+02 |
| | | Mean | NAN | 1.79E+02 | 1.84E+02 | 1.83E+02 | 1.83E+02 | **1.78E+02** | 1.85E+02 | 1.84E+02 |
| | gap | Best | NAN | **47.46%** | 49.46% | 48.90% | 48.90% | **47.46%** | 49.46% | 49.18% |
| | | Mean | NAN | 47.93% | 49.46% | 49.29% | 49.07% | **47.81%** | 49.62% | 49.46% |
| BPPC55 | obj | Best | NAN | 2.29E+02 | 2.31E+02 | **2.28E+02** | 2.29E+02 | **2.28E+02** | **2.28E+02** | 2.30E+02 |
| | | Mean | NAN | 2.29E+02 | 2.31E+02 | 2.30E+02 | 2.29E+02 | **2.28E+02** | 2.30E+02 | 2.31E+02 |
| | gap | Best | NAN | 91.70% | 91.77% | **91.67%** | 91.70% | **91.67%** | **91.67%** | 91.74% |
| | | Mean | NAN | 91.70% | 91.77% | 91.74% | 91.71% | **91.68%** | 91.72% | 91.77% |
| BPPC56 | obj | Best | NAN | **2.36E+02** | 2.42E+02 | 2.39E+02 | 2.40E+02 | 2.37E+02 | 2.39E+02 | 2.40E+02 |
| | | Mean | NAN | **2.37E+02** | NAN | 2.40E+02 | 2.40E+02 | 2.38E+02 | 2.40E+02 | 2.42E+02 |
| | gap | Best | NAN | **99.15%** | 99.17% | 99.16% | 99.17% | 99.16% | 99.16% | 99.17% |
| | | Mean | NAN | **99.15%** | NAN | 99.17% | 99.17% | 99.16% | 99.17% | 99.17% |
| BPPC57 | obj | Best | NAN | **3.04E+02** | NAN | **3.05E+02** | **3.04E+02** | **3.04E+02** | **3.05E+02** | **3.05E+02** |
| | | Mean | NAN | **3.05E+02** | NAN | 3.07E+02 | 3.06E+02 | **3.05E+02** | 3.06E+02 | 3.07E+02 |
| | gap | Best | NAN | **99.34%** | NAN | **99.34%** | **99.34%** | **99.34%** | **99.34%** | **99.34%** |
| | | Mean | NAN | **99.34%** | NAN | 99.35% | 99.35% | **99.34%** | 99.35% | 99.35% |
| BPPC58 | obj | Best | NAN | 3.69E+02 | NAN | **3.68E+02** | 3.69E+02 | **3.68E+02** | 3.70E+02 | 3.70E+02 |
| | | Mean | NAN | **3.70E+02** | NAN | **3.70E+02** | **3.70E+02** | **3.68E+02** | **3.70E+02** | **3.72E+02** |
| | gap | Best | NAN | 99.19% | NAN | **99.18%** | 99.19% | **99.18%** | 99.19% | 99.19% |
| | | Mean | NAN | **99.19%** | NAN | **99.19%** | **99.19%** | **99.19%** | **99.19%** | **99.19%** |
| BPPC59 | obj | Best | NAN | **4.14E+02** | NAN | **4.13E+02** | **4.14E+02** | **4.13E+02** | **4.13E+02** | **4.14E+02** |
| | | Mean | NAN | 4.15E+02 | NAN | **4.14E+02** | **4.14E+02** | **4.14E+02** | 4.15E+02 | 4.15E+02 |
| | gap | Best | NAN | **99.03%** | NAN | **99.03%** | **99.03%** | **99.03%** | **99.03%** | **99.03%** |
| | | Mean | NAN | 99.04% | NAN | **99.03%** | **99.03%** | **99.03%** | 99.04% | 99.04% |
| BPPC60 | obj | Best | NAN | 4.52E+02 | NAN | 4.51E+02 | 4.52E+02 | **4.51E+02** | **4.51E+02** | 4.52E+02 |
| | | Mean | NAN | 4.53E+02 | NAN | **4.52E+02** | **4.52E+02** | **4.52E+02** | **4.53E+02** | **4.53E+02** |
| | gap | Best | NAN | 98.01% | NAN | 98.00% | 98.01% | **98.00%** | **98.00%** | 98.01% |
| | | Mean | NAN | **98.01%** | NAN | **98.01%** | **98.01%** | **98.01%** | **98.01%** | **98.01%** |

3.6 Generalized bin packing problem (GBPPI)

Table S-16 provides the experimental results on 50 GBPPI problems.

**Table S-16** Experimental results on GBPPI test suit.

| Pro. | Metric | Status | GUROBI | OR-TOOLS | SCIP | SA | VNS | LNS | TS | GA |
|---|---|---|---|---|---|---|---|---|---|---|
| GBP PI01 | obj | Best | 2.84E+02 | **2.83E+02** | 3.14E+02 | 3.25E+02 | 3.45E+02 | 4.02E+02 | 3.91E+02 | 3.14E+02 |
| | | Mean | 2.89E+02 | **2.88E+02** | 3.14E+02 | 3.70E+02 | 3.74E+02 | 4.31E+02 | 4.20E+02 | 3.37E+02 |
| | gap | Best | 0.35% | **0.00%** | 9.87% | 12.92% | 17.97% | 29.60% | 27.62% | 9.87% |
| | | Mean | 2.00% | **1.80%** | 9.87% | 23.10% | 24.18% | 34.27% | 32.44% | 15.86% |
| GBP PI02 | obj | Best | **6.78E+02** | **6.78E+02** | **6.78E+02** | 8.25E+02 | 8.69E+02 | 9.31E+02 | 8.82E+02 | 7.51E+02 |
| | | Mean | **6.78E+02** | 6.80E+02 | **6.78E+02** | 9.04E+02 | 9.25E+02 | 1.01E+03 | 9.40E+02 | 8.03E+02 |
| | gap | Best | **0.00%** | **0.00%** | **0.00%** | 17.82% | 21.98% | 27.18% | 23.13% | 9.72% |
| | | Mean | **0.00%** | 0.26% | **0.00%** | 24.80% | 26.57% | 32.87% | 27.54% | 15.13% |
| | obj | Best | **4.77E+02** | **4.77E+02** | 5.39E+02 | 5.37E+02 | 5.45E+02 | 6.55E+02 | 5.77E+02 | 5.22E+02 |

| Pro. | Metric | Status | GUROBI | OR-TOOLS | SCIP | SA | VNS | LNS | TS | GA |
|---|---|---|---|---|---|---|---|---|---|---|
| GBP PI03 | | Mean | **4.77E+02** | 4.79E+02 | 5.39E+02 | 5.47E+02 | 5.67E+02 | 6.62E+02 | 6.17E+02 | 5.44E+02 |
| | gap | Best | **0.00%** | **0.00%** | 11.50% | 11.17% | 12.48% | 27.18% | 17.33% | 8.62% |
| | | Mean | **0.00%** | 0.49% | 11.50% | 12.84% | 15.81% | 27.93% | 22.54% | 12.28% |
| GBP PI04 | obj | Best | 8.21E+02 | **8.00E+02** | 9.03E+02 | 9.04E+02 | 9.11E+02 | 1.00E+03 | 9.58E+02 | 8.35E+02 |
| | | Mean | 8.28E+02 | **8.14E+02** | 9.03E+02 | 9.42E+02 | 9.58E+02 | 1.02E+03 | 1.02E+03 | 8.63E+02 |
| | gap | Best | 5.48% | **3.00%** | 14.06% | 14.16% | 14.82% | 22.63% | 19.00% | 7.07% |
| | | Mean | 6.30% | **4.70%** | 14.06% | 17.50% | 18.89% | 23.77% | 23.66% | 10.07% |
| GBP PI05 | obj | Best | **1.13E+03** | 1.16E+03 | 1.28E+03 | 1.39E+03 | 1.35E+03 | 1.45E+03 | 1.46E+03 | 1.24E+03 |
| | | Mean | 1.21E+03 | **1.17E+03** | 1.28E+03 | 1.43E+03 | 1.47E+03 | 1.47E+03 | 1.51E+03 | 1.29E+03 |
| | gap | Best | **0.00%** | 2.68% | 11.83% | 18.89% | 16.79% | 22.57% | 22.84% | 9.05% |
| | | Mean | 7.18% | **3.97%** | 11.83% | 21.16% | 23.52% | 23.61% | 25.20% | 12.69% |
| GBP PI06 | obj | Best | **1.65E+03** | 1.66E+03 | 1.76E+03 | 2.00E+03 | 2.06E+03 | 2.21E+03 | 2.01E+03 | 1.82E+03 |
| | | Mean | **1.65E+03** | 1.68E+03 | 1.76E+03 | 2.10E+03 | 2.12E+03 | 2.29E+03 | 2.11E+03 | 1.85E+03 |
| | gap | Best | **0.00%** | 0.18% | 5.87% | 17.48% | 19.84% | 25.25% | 17.97% | 9.03% |
| | | Mean | **0.00%** | 1.54% | 5.87% | 21.15% | 22.18% | 27.82% | 21.65% | 10.66% |
| GBP PI07 | obj | Best | 1.77E+03 | **1.57E+03** | 1.82E+03 | 1.90E+03 | 1.86E+03 | 1.97E+03 | 2.06E+03 | 1.75E+03 |
| | | Mean | 1.77E+03 | **1.59E+03** | 1.82E+03 | 1.92E+03 | 1.91E+03 | 1.99E+03 | 2.09E+03 | 1.78E+03 |
| | gap | Best | 11.76% | **0.45%** | 14.14% | 17.98% | 16.31% | 20.85% | 24.12% | 10.91% |
| | | Mean | 11.76% | **1.68%** | 14.14% | 18.59% | 18.29% | 21.78% | 25.34% | 12.51% |
| GBP PI08 | obj | Best | 2.11E+03 | **2.10E+03** | 2.38E+03 | 2.45E+03 | 2.46E+03 | 2.82E+03 | 2.61E+03 | 2.32E+03 |
| | | Mean | 2.16E+03 | **2.12E+03** | 2.38E+03 | 2.51E+03 | 2.51E+03 | 2.84E+03 | 2.69E+03 | 2.38E+03 |
| | gap | Best | 3.51% | **3.28%** | 14.65% | 16.95% | 17.36% | 27.83% | 22.02% | 12.41% |
| | | Mean | 5.86% | **3.88%** | 14.65% | 18.96% | 18.94% | 28.47% | 24.47% | 14.67% |
| GBP PI09 | obj | Best | **2.84E+03** | 2.86E+03 | 3.19E+03 | 3.57E+03 | 3.46E+03 | 4.44E+03 | 3.85E+03 | 3.34E+03 |
| | | Mean | **2.84E+03** | 2.87E+03 | 3.19E+03 | 3.83E+03 | 3.68E+03 | 4.48E+03 | 3.97E+03 | 3.36E+03 |
| | gap | Best | **0.00%** | 0.87% | 11.01% | 20.57% | 18.00% | 36.08% | 26.19% | 14.93% |
| | | Mean | **0.00%** | 1.19% | 11.01% | 25.86% | 22.67% | 36.58% | 28.46% | 15.47% |
| GBP PI10 | obj | Best | NAN | **2.67E+03** | 3.09E+03 | 3.28E+03 | 3.13E+03 | 3.71E+03 | 3.61E+03 | 2.93E+03 |
| | | Mean | NAN | **2.68E+03** | 3.09E+03 | 3.32E+03 | 3.20E+03 | 3.80E+03 | 3.70E+03 | 3.04E+03 |
| | gap | Best | NAN | **2.13%** | 15.41% | 20.21% | 16.54% | 29.63% | 27.64% | 10.76% |
| | | Mean | NAN | **2.55%** | 15.41% | 21.18% | 18.31% | 31.16% | 29.28% | 13.97% |
| GBP PI11 | obj | Best | NAN | **4.57E+03** | 5.28E+03 | 5.39E+03 | 5.29E+03 | 5.87E+03 | 5.66E+03 | 5.27E+03 |
| | | Mean | NAN | **4.60E+03** | 5.28E+03 | 5.48E+03 | 5.38E+03 | 5.92E+03 | 5.81E+03 | 5.34E+03 |
| | gap | Best | NAN | **1.49%** | 14.83% | 16.57% | 14.91% | 23.40% | 20.51% | 14.59% |
| | | Mean | NAN | **2.30%** | 14.83% | 17.98% | 16.35% | 24.01% | 22.58% | 15.84% |
| GBP PI12 | obj | Best | NAN | **6.04E+03** | 6.70E+03 | 7.79E+03 | 7.71E+03 | 8.92E+03 | 8.24E+03 | 7.47E+03 |
| | | Mean | NAN | **6.06E+03** | 6.70E+03 | 8.07E+03 | 7.86E+03 | 9.09E+03 | 8.39E+03 | 7.97E+03 |
| | gap | Best | NAN | **1.49%** | 11.16% | 23.63% | 22.89% | 33.33% | 27.78% | 20.39% |
| | | Mean | NAN | **1.82%** | 11.16% | 26.22% | 24.35% | 34.54% | 29.09% | 25.28% |
| GBP PI13 | obj | Best | NAN | **6.85E+03** | 8.35E+03 | 8.19E+03 | 7.68E+03 | 9.26E+03 | 9.40E+03 | 8.44E+03 |
| | | Mean | NAN | **6.88E+03** | 8.35E+03 | 8.42E+03 | 7.83E+03 | 9.40E+03 | 9.46E+03 | 8.52E+03 |
| | gap | Best | NAN | **0.60%** | 18.49% | 16.94% | 11.38% | 26.53% | 27.65% | 19.38% |
| | | Mean | NAN | **1.15%** | 18.49% | 19.16% | 13.11% | 27.58% | 28.09% | 20.13% |
| GBP PI14 | obj | Best | NAN | **1.07E+04** | 1.29E+04 | 1.31E+04 | 1.24E+04 | 1.37E+04 | 1.38E+04 | 1.41E+04 |
| | | Mean | NAN | **1.18E+04** | 1.29E+04 | 1.32E+04 | 1.27E+04 | 1.39E+04 | 1.39E+04 | 1.41E+04 |
| | gap | Best | NAN | **3.80%** | 11.43% | 12.78% | 8.24% | 16.62% | 17.40% | 18.95% |

| Pro. | Metric | Status | GUROBI | OR-TOOLS | SCIP | SA | VNS | LNS | TS | GA |
|---|---|---|---|---|---|---|---|---|---|---|
| | | Mean | NAN | **9.41%** | 11.43% | 13.41% | 9.86% | 17.76% | 17.80% | 19.30% |
| GBP PI15 | obj | Best | NAN | **1.53E+04** | 1.72E+04 | 2.17E+04 | 2.11E+04 | 2.21E+04 | 2.15E+04 | 2.13E+04 |
| | | Mean | NAN | **1.54E+04** | 1.72E+04 | 2.21E+04 | 2.13E+04 | 2.24E+04 | 2.17E+04 | 2.17E+04 |
| | gap | Best | NAN | **2.75%** | 13.58% | 31.67% | 29.67% | 33.00% | 31.04% | 30.28% |
| | | Mean | NAN | **3.47%** | 13.58% | 32.81% | 30.51% | 33.86% | 31.60% | 31.59% |
| GBP PI16 | obj | Best | **3.40E+02** | **3.40E+02** | 3.90E+02 | 4.11E+02 | 4.23E+02 | 3.98E+02 | 4.32E+02 | 3.86E+02 |
| | | Mean | **3.40E+02** | 3.47E+02 | 3.90E+02 | 4.30E+02 | 4.36E+02 | 4.20E+02 | 4.44E+02 | 4.17E+02 |
| | gap | Best | **0.00%** | **0.00%** | 12.82% | 17.27% | 19.62% | 14.57% | 21.30% | 11.92% |
| | | Mean | **0.00%** | 2.12% | 12.82% | 20.91% | 21.99% | 18.97% | 23.46% | 18.35% |
| GBP PI17 | obj | Best | **4.79E+02** | 4.89E+02 | 4.89E+02 | 5.95E+02 | 6.03E+02 | 6.46E+02 | 6.08E+02 | 5.17E+02 |
| | | Mean | **4.79E+02** | 4.97E+02 | 4.89E+02 | 6.18E+02 | 6.33E+02 | 6.85E+02 | 6.31E+02 | 5.34E+02 |
| | gap | Best | **0.00%** | 2.04% | 2.04% | 19.50% | 20.56% | 25.85% | 21.22% | 7.35% |
| | | Mean | **0.00%** | 3.54% | 2.04% | 22.31% | 24.26% | 29.79% | 24.07% | 10.19% |
| GBP PI18 | obj | Best | **7.86E+02** | 7.94E+02 | 8.64E+02 | 9.09E+02 | 8.92E+02 | 9.55E+02 | 9.57E+02 | 8.76E+02 |
| | | Mean | **7.96E+02** | 7.96E+02 | 8.64E+02 | 9.39E+02 | 9.21E+02 | 9.61E+02 | 9.84E+02 | 9.04E+02 |
| | gap | Best | **0.25%** | 1.26% | 9.26% | 13.75% | 12.11% | 17.91% | 18.08% | 10.50% |
| | | Mean | **1.45%** | 1.55% | 9.26% | 16.44% | 14.79% | 18.38% | 20.25% | 13.24% |
| GBP PI19 | obj | Best | **1.28E+03** | 1.28E+03 | 1.41E+03 | 1.50E+03 | 1.50E+03 | 1.55E+03 | 1.58E+03 | 1.49E+03 |
| | | Mean | **1.28E+03** | 1.29E+03 | 1.41E+03 | 1.55E+03 | 1.52E+03 | 1.57E+03 | 1.61E+03 | 1.52E+03 |
| | gap | Best | **0.00%** | 0.16% | 9.50% | 15.16% | 14.99% | 17.62% | 19.39% | 14.25% |
| | | Mean | **0.00%** | 0.84% | 9.50% | 17.39% | 16.07% | 18.62% | 20.74% | 16.19% |
| GBP PI20 | obj | Best | 2.01E+03 | **1.97E+03** | 2.18E+03 | 2.34E+03 | 2.25E+03 | 2.41E+03 | 2.45E+03 | 2.20E+03 |
| | | Mean | 2.02E+03 | **1.98E+03** | 2.18E+03 | 2.36E+03 | 2.31E+03 | 2.43E+03 | 2.48E+03 | 2.24E+03 |
| | gap | Best | 3.83% | **2.03%** | 11.42% | 17.54% | 13.94% | 19.93% | 21.01% | 12.22% |
| | | Mean | 4.55% | **2.36%** | 11.42% | 18.15% | 16.17% | 20.64% | 22.00% | 13.83% |
| GBP PI21 | obj | Best | 2.26E+03 | **2.19E+03** | 2.44E+03 | 2.56E+03 | 2.50E+03 | 2.64E+03 | 2.69E+03 | 2.39E+03 |
| | | Mean | 2.29E+03 | **2.20E+03** | 2.44E+03 | 2.64E+03 | 2.53E+03 | 2.69E+03 | 2.71E+03 | 2.50E+03 |
| | gap | Best | 3.94% | **1.00%** | 10.97% | 15.25% | 13.21% | 18.00% | 19.41% | 9.10% |
| | | Mean | 5.15% | **1.33%** | 10.97% | 17.87% | 14.35% | 19.46% | 20.03% | 13.13% |
| GBP PI22 | obj | Best | NAN | **4.84E+03** | 5.53E+03 | 5.62E+03 | 5.45E+03 | 6.07E+03 | 5.93E+03 | 5.69E+03 |
| | | Mean | NAN | **4.85E+03** | 5.53E+03 | 5.74E+03 | 5.53E+03 | 6.09E+03 | 5.99E+03 | 5.72E+03 |
| | gap | Best | NAN | **2.37%** | 14.44% | 15.93% | 13.18% | 22.12% | 20.20% | 16.94% |
| | | Mean | NAN | **2.44%** | 14.44% | 17.64% | 14.46% | 22.36% | 21.06% | 17.40% |
| GBP PI23 | obj | Best | 4.08E+03 | **3.47E+03** | 4.22E+03 | 4.07E+03 | 3.93E+03 | 4.50E+03 | 4.43E+03 | 3.92E+03 |
| | | Mean | 8.00E+19 | **3.50E+03** | 4.22E+03 | 4.16E+03 | 3.98E+03 | 4.55E+03 | 4.54E+03 | 4.04E+03 |
| | gap | Best | 17.61% | **3.14%** | 20.27% | 17.33% | 14.36% | 25.26% | 24.03% | 14.27% |
| | | Mean | 83.52% | **3.89%** | 20.27% | 19.10% | 15.45% | 26.01% | 25.88% | 16.69% |
| GBP PI24 | obj | Best | NAN | **8.55E+03** | 1.21E+04 | 1.05E+04 | 1.04E+04 | 1.06E+04 | 1.08E+04 | 1.13E+04 |
| | | Mean | NAN | **8.63E+03** | 1.21E+04 | 1.08E+04 | 1.05E+04 | 1.07E+04 | 1.11E+04 | 1.15E+04 |
| | gap | Best | NAN | **0.02%** | 28.17% | 16.71% | 16.00% | 17.43% | 19.25% | 23.14% |
| | | Mean | NAN | **0.96%** | 28.17% | 19.04% | 17.19% | 18.51% | 21.54% | 23.96% |
| GBP PI25 | obj | Best | NAN | **1.39E+04** | 1.52E+04 | 1.57E+04 | 1.50E+04 | 1.53E+04 | 1.54E+04 | 1.56E+04 |
| | | Mean | NAN | **1.39E+04** | 1.52E+04 | 1.59E+04 | 1.52E+04 | 1.54E+04 | 1.57E+04 | 1.57E+04 |
| | gap | Best | NAN | **7.12%** | 15.03% | 17.91% | 14.21% | 15.46% | 16.12% | 17.42% |
| | | Mean | NAN | **7.46%** | 15.03% | 18.66% | 15.27% | 16.20% | 17.71% | 18.03% |
| GBP PI26 | obj | Best | **3.42E+02** | 3.50E+02 | 3.66E+02 | 4.09E+02 | 4.06E+02 | 6.91E+02 | 4.17E+02 | 4.26E+02 |
| | | Mean | **3.42E+02** | 3.52E+02 | 3.66E+02 | 4.39E+02 | 4.35E+02 | 7.25E+02 | 4.54E+02 | 4.36E+02 |

| Pro. | Metric | Status | GUROBI | OR-TOOLS | SCIP | SA | VNS | LNS | TS | GA |
|---|---|---|---|---|---|---|---|---|---|---|
| | gap | Best | **0.00%** | 2.29% | 6.56% | 16.38% | 15.76% | 50.51% | 17.99% | 19.72% |
| | | Mean | **0.00%** | 2.78% | 6.56% | 21.88% | 21.33% | 52.80% | 24.37% | 21.61% |
| GBP PI27 | obj | Best | **7.45E+02** | 7.45E+02 | 7.45E+02 | 8.20E+02 | 9.08E+02 | 9.93E+02 | 9.33E+02 | 7.96E+02 |
| | | Mean | **7.45E+02** | **7.45E+02** | **7.45E+02** | 8.70E+02 | 9.47E+02 | 1.10E+03 | 1.01E+03 | 8.72E+02 |
| | gap | Best | **0.00%** | **0.00%** | **0.00%** | 9.15% | 17.95% | 24.97% | 20.15% | 6.41% |
| | | Mean | **0.00%** | **0.00%** | **0.00%** | 14.30% | 21.32% | 31.99% | 26.23% | 14.31% |
| GBP PI28 | obj | Best | **5.39E+02** | **5.39E+02** | 6.74E+02 | 6.18E+02 | 6.29E+02 | 8.50E+02 | 6.65E+02 | 6.29E+02 |
| | | Mean | **5.39E+02** | 5.53E+02 | 6.74E+02 | 6.41E+02 | 6.61E+02 | 8.75E+02 | 6.88E+02 | 6.51E+02 |
| | gap | Best | **0.00%** | **0.00%** | 20.03% | 12.78% | 14.31% | 36.59% | 18.95% | 14.31% |
| | | Mean | **0.00%** | 2.58% | 20.03% | 15.91% | 18.36% | 38.36% | 21.60% | 17.05% |
| GBP PI29 | obj | Best | **7.42E+02** | 7.51E+02 | 8.86E+02 | 8.69E+02 | 9.25E+02 | 1.21E+03 | 9.77E+02 | 8.33E+02 |
| | | Mean | 7.84E+02 | **7.58E+02** | 8.86E+02 | 8.99E+02 | 9.57E+02 | 1.28E+03 | 9.97E+02 | 8.58E+02 |
| | gap | Best | **2.83%** | 3.99% | 18.62% | 17.03% | 22.05% | 40.22% | 26.20% | 13.45% |
| | | Mean | 8.01% | **4.87%** | 18.62% | 19.73% | 24.59% | 43.41% | 27.63% | 15.87% |
| GBP PI30 | obj | Best | **9.57E+02** | 9.74E+02 | 1.14E+03 | 1.10E+03 | 1.06E+03 | 1.50E+03 | 1.16E+03 | 1.03E+03 |
| | | Mean | 1.02E+03 | **9.85E+02** | 1.14E+03 | 1.14E+03 | 1.10E+03 | 1.54E+03 | 1.19E+03 | 1.04E+03 |
| | gap | Best | **1.36%** | 3.08% | 16.83% | 14.42% | 11.03% | 37.02% | 18.76% | 8.35% |
| | | Mean | 7.16% | **4.17%** | 16.83% | 17.35% | 14.08% | 38.75% | 20.52% | 9.62% |
| GBP PI31 | obj | Best | **1.66E+03** | 1.66E+03 | 1.76E+03 | 1.96E+03 | 1.90E+03 | 2.16E+03 | 1.92E+03 | 1.79E+03 |
| | | Mean | **1.66E+03** | 1.67E+03 | 1.76E+03 | 2.00E+03 | 2.03E+03 | 2.23E+03 | 2.02E+03 | 1.82E+03 |
| | gap | Best | **0.00%** | 0.12% | 5.46% | 15.21% | 12.39% | 23.10% | 13.53% | 7.05% |
| | | Mean | **0.00%** | 0.45% | 5.46% | 17.02% | 17.86% | 25.52% | 17.83% | 8.60% |
| GBP PI32 | obj | Best | 1.31E+03 | **1.19E+03** | 1.41E+03 | 1.53E+03 | 1.41E+03 | 2.37E+03 | 1.58E+03 | 1.37E+03 |
| | | Mean | 1.31E+03 | **1.19E+03** | 1.41E+03 | 1.55E+03 | 1.49E+03 | 2.43E+03 | 1.67E+03 | 1.44E+03 |
| | gap | Best | 10.81% | **1.43%** | 17.13% | 23.21% | 16.95% | 50.55% | 25.79% | 14.53% |
| | | Mean | 10.81% | **1.76%** | 17.13% | 24.48% | 21.16% | 51.85% | 29.74% | 18.68% |
| GBP PI33 | obj | Best | 2.78E+03 | **2.55E+03** | 2.97E+03 | 2.99E+03 | 2.81E+03 | 3.77E+03 | 3.10E+03 | 2.84E+03 |
| | | Mean | 2.93E+03 | **2.58E+03** | 2.97E+03 | 3.04E+03 | 2.99E+03 | 3.82E+03 | 3.20E+03 | 2.89E+03 |
| | gap | Best | 9.59% | **1.76%** | 15.38% | 15.97% | 10.78% | 33.40% | 19.09% | 11.59% |
| | | Mean | 14.09% | **2.78%** | 15.38% | 17.54% | 16.06% | 34.38% | 21.60% | 13.07% |
| GBP PI34 | obj | Best | **2.80E+03** | 2.80E+03 | 3.18E+03 | 3.48E+03 | 3.58E+03 | 4.44E+03 | 3.66E+03 | 3.25E+03 |
| | | Mean | **2.80E+03** | 2.82E+03 | 3.18E+03 | 3.64E+03 | 3.70E+03 | 4.51E+03 | 3.82E+03 | 3.28E+03 |
| | gap | Best | **0.00%** | 0.14% | 12.09% | 19.64% | 21.88% | 36.96% | 23.59% | 13.77% |
| | | Mean | **0.00%** | 0.71% | 12.09% | 22.92% | 24.20% | 37.95% | 26.70% | 14.72% |
| GBP PI35 | obj | Best | NAN | **3.50E+03** | 4.01E+03 | 4.18E+03 | 4.02E+03 | 5.70E+03 | 4.34E+03 | 4.06E+03 |
| | | Mean | NAN | **3.52E+03** | 4.01E+03 | 4.23E+03 | 4.15E+03 | 5.77E+03 | 4.44E+03 | 4.14E+03 |
| | gap | Best | NAN | **1.63%** | 14.18% | 17.55% | 14.31% | 39.54% | 20.74% | 15.28% |
| | | Mean | NAN | **2.15%** | 14.18% | 18.52% | 17.00% | 40.36% | 22.46% | 16.81% |
| GBP PI36 | obj | Best | NAN | **4.14E+03** | 5.00E+03 | 4.92E+03 | 4.97E+03 | 6.19E+03 | 5.35E+03 | 4.52E+03 |
| | | Mean | NAN | **4.16E+03** | 5.00E+03 | 5.02E+03 | 5.07E+03 | 6.37E+03 | 5.43E+03 | 4.73E+03 |
| | gap | Best | NAN | **2.42%** | 19.20% | 17.98% | 18.78% | 34.83% | 24.62% | 10.61% |
| | | Mean | NAN | **2.90%** | 19.20% | 19.58% | 20.34% | 36.62% | 25.65% | 14.46% |
| GBP PI37 | obj | Best | NAN | **6.20E+03** | 6.84E+03 | 7.80E+03 | 7.80E+03 | 8.68E+03 | 7.92E+03 | 7.53E+03 |
| | | Mean | NAN | **6.22E+03** | 6.84E+03 | 8.01E+03 | 8.03E+03 | 9.01E+03 | 8.17E+03 | 7.93E+03 |
| | gap | Best | NAN | **2.45%** | 11.54% | 22.46% | 22.52% | 30.32% | 23.62% | 19.72% |
| | | Mean | NAN | **2.81%** | 11.54% | 24.51% | 24.72% | 32.80% | 25.97% | 23.71% |
| | obj | Best | NAN | **7.80E+03** | 9.98E+03 | 9.55E+03 | 9.11E+03 | 1.40E+04 | 1.04E+04 | 9.66E+03 |

| Pro. | Metric | Status | GUROBI | OR-TOOLS | SCIP | SA | VNS | LNS | TS | GA |
|---|---|---|---|---|---|---|---|---|---|---|
| GBP PI38 | | Mean | NAN | **7.86E+03** | 9.98E+03 | 9.80E+03 | 9.47E+03 | 1.41E+04 | 1.06E+04 | 9.82E+03 |
| | gap | Best | NAN | **10.14%** | 12.95% | 8.97% | 4.63% | 37.83% | 16.09% | 10.05% |
| | | Mean | NAN | **10.61%** | 12.95% | 11.30% | 8.16% | 38.36% | 17.73% | 11.50% |
| GBP PI39 | obj | Best | NAN | **1.10E+04** | 1.32E+04 | 1.30E+04 | 1.30E+04 | 1.65E+04 | 1.40E+04 | 1.38E+04 |
| | | Mean | NAN | **1.11E+04** | 1.32E+04 | 1.34E+04 | 1.33E+04 | 1.65E+04 | 1.42E+04 | 1.41E+04 |
| | gap | Best | NAN | **9.03%** | 7.73% | 6.94% | 6.94% | 26.27% | 12.95% | 12.29% |
| | | Mean | NAN | **9.60%** | 7.73% | 9.05% | 8.53% | 26.50% | 14.66% | 13.86% |
| GBP PI40 | obj | Best | NAN | **1.58E+04** | 1.69E+04 | 2.07E+04 | 2.01E+04 | 2.23E+04 | 2.09E+04 | 2.07E+04 |
| | | Mean | NAN | **1.61E+04** | 1.69E+04 | 2.08E+04 | 2.05E+04 | 2.25E+04 | 2.12E+04 | 2.09E+04 |
| | gap | Best | NAN | **3.18%** | 9.42% | 26.01% | 24.03% | 31.36% | 26.80% | 26.05% |
| | | Mean | NAN | **4.71%** | 9.42% | 26.52% | 25.30% | 31.95% | 27.78% | 26.86% |
| GBP PI41 | obj | Best | **3.82E+02** | **3.82E+02** | 3.88E+02 | 4.12E+02 | 4.12E+02 | 6.26E+02 | 4.12E+02 | 4.02E+02 |
| | | Mean | **3.82E+02** | 3.83E+02 | 3.88E+02 | 4.26E+02 | 4.16E+02 | 6.76E+02 | 4.29E+02 | 4.23E+02 |
| | gap | Best | **0.00%** | **0.00%** | 1.55% | 7.28% | 7.28% | 38.98% | 7.28% | 4.98% |
| | | Mean | **0.00%** | 0.21% | 1.55% | 10.36% | 8.21% | 43.41% | 10.98% | 9.53% |
| GBP PI42 | obj | Best | **5.18E+02** | **5.18E+02** | 5.34E+02 | 5.83E+02 | 5.78E+02 | 7.74E+02 | 6.22E+02 | 5.87E+02 |
| | | Mean | **5.18E+02** | 5.23E+02 | 5.34E+02 | 6.09E+02 | 5.89E+02 | 7.98E+02 | 6.47E+02 | 6.10E+02 |
| | gap | Best | **0.00%** | **0.00%** | 3.00% | 11.15% | 10.38% | 33.07% | 16.72% | 11.75% |
| | | Mean | **0.00%** | 1.02% | 3.00% | 14.87% | 12.09% | 35.06% | 19.92% | 14.96% |
| GBP PI43 | obj | Best | **9.87E+02** | 9.89E+02 | 1.07E+03 | 1.16E+03 | 1.11E+03 | 1.32E+03 | 1.22E+03 | 1.10E+03 |
| | | Mean | 1.10E+03 | **1.01E+03** | 1.07E+03 | 1.19E+03 | 1.14E+03 | 1.34E+03 | 1.24E+03 | 1.13E+03 |
| | gap | Best | **2.53%** | 2.73% | 10.18% | 16.71% | 13.02% | 27.18% | 21.08% | 12.62% |
| | | Mean | 12.58% | **4.32%** | 10.18% | 19.38% | 15.38% | 28.43% | 22.13% | 14.83% |
| GBP PI44 | obj | Best | **1.12E+03** | 1.16E+03 | 1.21E+03 | 1.26E+03 | 1.32E+03 | 1.47E+03 | 1.35E+03 | 1.27E+03 |
| | | Mean | **1.15E+03** | 1.18E+03 | 1.21E+03 | 1.32E+03 | 1.37E+03 | 1.52E+03 | 1.38E+03 | 1.33E+03 |
| | gap | Best | **0.27%** | 3.95% | 7.37% | 10.92% | 15.43% | 23.95% | 17.12% | 12.18% |
| | | Mean | **3.02%** | 5.01% | 7.37% | 15.41% | 18.28% | 26.61% | 19.02% | 15.78% |
| GBP PI45 | obj | Best | 1.60E+03 | **1.52E+03** | 1.72E+03 | 1.77E+03 | 1.73E+03 | 2.55E+03 | 1.80E+03 | 1.72E+03 |
| | | Mean | 1.71E+03 | **1.54E+03** | 1.72E+03 | 1.80E+03 | 1.79E+03 | 2.59E+03 | 1.93E+03 | 1.78E+03 |
| | gap | Best | 8.82% | **3.76%** | 15.33% | 17.63% | 15.48% | 42.91% | 19.04% | 15.13% |
| | | Mean | 14.68% | **5.33%** | 15.33% | 18.86% | 18.47% | 43.65% | 24.19% | 17.99% |
| GBP PI46 | obj | Best | 2.71E+03 | **2.57E+03** | 2.86E+03 | 2.91E+03 | 2.90E+03 | 3.34E+03 | 3.03E+03 | 2.87E+03 |
| | | Mean | 2.97E+03 | **2.59E+03** | 2.86E+03 | 2.99E+03 | 2.98E+03 | 3.40E+03 | 3.07E+03 | 3.00E+03 |
| | gap | Best | 6.60% | **1.40%** | 11.31% | 12.92% | 12.59% | 24.04% | 16.23% | 11.71% |
| | | Mean | 14.25% | **1.99%** | 11.31% | 15.31% | 14.96% | 25.55% | 17.34% | 15.39% |
| GBP PI47 | obj | Best | NAN | **4.55E+03** | 5.28E+03 | 5.35E+03 | 5.19E+03 | 6.11E+03 | 5.48E+03 | 5.27E+03 |
| | | Mean | NAN | **4.58E+03** | 5.28E+03 | 5.43E+03 | 5.30E+03 | 6.20E+03 | 5.57E+03 | 5.35E+03 |
| | gap | Best | NAN | **1.43%** | 14.97% | 16.13% | 13.49% | 26.56% | 18.04% | 14.76% |
| | | Mean | NAN | **1.99%** | 14.97% | 17.31% | 15.29% | 27.57% | 19.46% | 16.07% |
| GBP PI48 | obj | Best | NAN | **3.24E+03** | 3.78E+03 | 3.83E+03 | 3.63E+03 | 5.41E+03 | 4.12E+03 | 3.73E+03 |
| | | Mean | NAN | **3.26E+03** | 3.78E+03 | 3.90E+03 | 3.74E+03 | 5.45E+03 | 4.26E+03 | 3.77E+03 |
| | gap | Best | NAN | **2.34%** | 16.22% | 17.34% | 12.76% | 41.51% | 23.10% | 15.05% |
| | | Mean | NAN | **2.78%** | 16.22% | 18.84% | 15.41% | 41.91% | 25.72% | 15.92% |
| GBP PI49 | obj | Best | NAN | **1.31E+04** | 1.41E+04 | 1.44E+04 | 1.41E+04 | 1.65E+04 | 1.47E+04 | 1.50E+04 |
| | | Mean | NAN | **1.33E+04** | 1.41E+04 | 1.46E+04 | 1.43E+04 | 1.66E+04 | 1.49E+04 | 1.53E+04 |
| | gap | Best | NAN | **4.12%** | 10.90% | 12.96% | 11.11% | 23.97% | 14.60% | 16.24% |
| | | Mean | NAN | **5.64%** | 10.90% | 13.68% | 11.96% | 24.26% | 15.63% | 18.06% |

| Pro. | Metric | Status | GUROBI | OR-TOOLS | SCIP | SA | VNS | LNS | TS | GA |
|---|---|---|---|---|---|---|---|---|---|---|
| GBP PI50 | obj | Best | NAN | **1.25E+04** | 1.45E+04 | 1.34E+04 | 1.36E+04 | 1.58E+04 | 1.41E+04 | 1.42E+04 |
| | | Mean | NAN | **1.28E+04** | 1.45E+04 | 1.37E+04 | 1.36E+04 | 1.59E+04 | 1.42E+04 | 1.44E+04 |
| | gap | Best | NAN | **3.38%** | 16.65% | 10.19% | 10.98% | 23.59% | 14.33% | 15.12% |
| | | Mean | NAN | **5.44%** | 16.65% | 11.83% | 11.54% | 24.14% | 14.73% | 16.22% |

3.7 Quadratic multiple knapsack problem (QMKP)

The experimental results of QMKP are shown in Table S-17.

**Table S-17** Experimental results on QMKP test suit.

| Pro. | Metric | Status | GUROBI | OR-TOOLS | SCIP | SA | VNS | LNS | TS | GA |
|---|---|---|---|---|---|---|---|---|---|---|
| QMKP01 | obj | Best | **9.98E+03** | **9.98E+03** | 9.32E+03 | 9.98E+03 | 9.98E+03 | **9.98E+03** | **9.98E+03** | **9.98E+03** |
| | | Mean | **9.98E+03** | 9.97E+03 | 9.32E+03 | 9.94E+03 | 9.94E+03 | 9.97E+03 | 9.92E+03 | 9.93E+03 |
| | gap | Best | **0.00%** | **0.00%** | 7.07% | 0.35% | 0.36% | **0.00%** | **0.00%** | **0.00%** |
| | | Mean | **0.00%** | 0.11% | 7.07% | 0.82% | 0.37% | 0.13% | 0.63% | 0.50% |
| QMKP02 | obj | Best | **1.05E+04** | **1.05E+04** | **1.05E+04** | **1.05E+04** | **1.05E+04** | **1.05E+04** | **1.05E+04** | **1.05E+04** |
| | | Mean | **1.05E+04** | **1.05E+04** | **1.05E+04** | **1.05E+04** | **1.05E+04** | **1.05E+04** | **1.05E+04** | **1.05E+04** |
| | gap | Best | **0.00%** | **0.00%** | **0.00%** | **0.00%** | **0.00%** | **0.00%** | **0.00%** | **0.00%** |
| | | Mean | **0.00%** | **0.00%** | **0.00%** | **0.00%** | **0.00%** | **0.00%** | **0.00%** | **0.00%** |
| QMKP03 | obj | Best | **8.74E+03** | **8.74E+03** | 8.46E+03 | 8.64E+03 | 8.74E+03 | **8.74E+03** | 8.44E+03 | 8.67E+03 |
| | | Mean | **8.74E+03** | 8.72E+03 | 8.46E+03 | 8.50E+03 | 8.64E+03 | 8.64E+03 | 8.31E+03 | 8.49E+03 |
| | gap | Best | **0.00%** | **0.00%** | 3.37% | 2.85% | 1.14% | **0.00%** | 3.53% | 0.83% |
| | | Mean | **0.00%** | 0.24% | 3.37% | 4.69% | 1.15% | 1.25% | 5.23% | 2.99% |
| QMKP04 | obj | Best | 4.81E+03 | 8.07E+03 | 3.86E+03 | 5.80E+03 | 6.09E+03 | 7.43E+03 | **9.02E+03** | 7.33E+03 |
| | | Mean | 4.86E+03 | **7.44E+03** | 3.86E+03 | 5.59E+03 | 5.74E+03 | 7.04E+03 | 6.98E+03 | 6.65E+03 |
| | gap | Best | 120.08% | 33.67% | 179.36% | 93.31% | 87.76% | 45.09% | **19.55%** | 47.07% |
| | | Mean | 121.82% | **46.09%** | 179.36% | 106.67% | 88.02% | 53.63% | 62.58% | 62.73% |
| QMKP05 | obj | Best | 4.97E+03 | 5.48E+03 | 3.68E+03 | 5.66E+03 | 5.36E+03 | 5.68E+03 | 5.30E+03 | **5.69E+03** |
| | | Mean | 4.97E+03 | 5.35E+03 | 3.68E+03 | 5.39E+03 | 5.16E+03 | **5.59E+03** | 5.20E+03 | 5.48E+03 |
| | gap | Best | 66.85% | 51.34% | 125.00% | 53.93% | 60.77% | 46.06% | 56.54% | **45.57%** |
| | | Mean | 66.85% | 54.99% | 125.00% | 58.76% | 60.90% | **48.22%** | 59.35% | 51.45% |
| QMKP06 | obj | Best | **1.99E+04** | **1.99E+04** | **1.99E+04** | **1.99E+04** | **1.99E+04** | **1.99E+04** | **1.99E+04** | **1.99E+04** |
| | | Mean | **1.99E+04** | **1.99E+04** | **1.99E+04** | **1.99E+04** | **1.99E+04** | **1.99E+04** | 1.98E+04 | **1.99E+04** |
| | gap | Best | **0.00%** | **0.00%** | **0.00%** | **0.00%** | **0.00%** | **0.00%** | **0.00%** | **0.00%** |
| | | Mean | **0.00%** | **0.00%** | **0.00%** | **0.00%** | **0.00%** | **0.00%** | 0.10% | **0.00%** |
| QMKP07 | obj | Best | 1.50E+04 | 1.71E+04 | 1.23E+04 | 1.71E+04 | 1.63E+04 | 1.72E+04 | 1.69E+04 | **1.73E+04** |
| | | Mean | 1.50E+04 | 1.69E+04 | 1.23E+04 | 1.66E+04 | 1.60E+04 | **1.71E+04** | 1.65E+04 | 1.71E+04 |
| | gap | Best | 33.73% | 17.13% | 62.76% | 20.71% | 25.37% | 16.25% | 18.84% | **15.82%** |
| | | Mean | 33.73% | 18.23% | 62.76% | 27.11% | 25.42% | **17.41%** | 21.79% | 17.47% |
| QMKP08 | obj | Best | **2.68E+04** | **2.68E+04** | **2.68E+04** | **2.68E+04** | **2.68E+04** | **2.68E+04** | **2.68E+04** | **2.68E+04** |
| | | Mean | **2.68E+04** | **2.68E+04** | **2.68E+04** | **2.68E+04** | **2.68E+04** | **2.68E+04** | **2.68E+04** | **2.68E+04** |
| | gap | Best | **0.00%** | **0.00%** | **0.00%** | **0.00%** | **0.00%** | **0.00%** | **0.00%** | **0.00%** |
| | | Mean | **0.00%** | **0.00%** | **0.00%** | **0.00%** | **0.00%** | **0.00%** | **0.00%** | **0.00%** |
| QMKP09 | obj | Best | 3.91E+03 | **7.38E+03** | 3.59E+03 | 7.07E+03 | 6.09E+03 | 7.05E+03 | 6.87E+03 | 6.92E+03 |
| | | Mean | 3.91E+03 | **6.99E+03** | 3.59E+03 | 6.15E+03 | 5.69E+03 | 6.60E+03 | 6.53E+03 | 6.41E+03 |
| | gap | Best | 259.33% | **90.18%** | 290.95% | 129.84% | 146.75% | 99.05% | 104.29% | 102.85% |
| | | Mean | 259.33% | **100.96%** | 290.95% | 149.94% | 147.05% | 113.14% | 115.18% | 119.78% |
| QMKP10 | obj | Best | 4.86E+03 | 5.28E+03 | 4.39E+03 | 5.17E+03 | 5.15E+03 | 5.47E+03 | 5.10E+03 | **5.53E+03** |

| Pro. | Metric | Status | GUROBI | OR-TOOLS | SCIP | SA | VNS | LNS | TS | GA |
|---|---|---|---|---|---|---|---|---|---|---|
| | | Mean | 4.86E+03 | 5.15E+03 | 4.31E+03 | 5.01E+03 | 5.05E+03 | **5.33E+03** | 4.94E+03 | 5.14E+03 |
| | gap | Best | 28.51% | 18.38% | 42.43% | 24.93% | 23.78% | 14.12% | 22.51% | **12.95%** |
| | | Mean | 28.51% | 21.46% | 45.17% | 32.04% | 23.81% | **17.25%** | 26.57% | 21.76% |
| QMKP11 | obj | Best | **1.22E+04** | **1.22E+04** | 1.10E+04 | 1.20E+04 | 1.22E+04 | **1.22E+04** | 1.21E+04 | 1.22E+04 |
| | | Mean | **1.22E+04** | 1.22E+04 | 1.10E+04 | 1.20E+04 | 1.21E+04 | 1.21E+04 | 1.20E+04 | 1.21E+04 |
| | gap | Best | **0.00%** | **0.00%** | 10.53% | 1.69% | 0.45% | **0.00%** | 0.54% | 0.14% |
| | | Mean | **0.00%** | 0.03% | 10.63% | 2.14% | 0.46% | 0.47% | 1.37% | 0.84% |
| QMKP12 | obj | Best | **1.33E+04** | **1.33E+04** | **1.33E+04** | **1.33E+04** | **1.33E+04** | **1.33E+04** | **1.33E+04** | **1.33E+04** |
| | | Mean | **1.33E+04** | **1.33E+04** | **1.33E+04** | **1.33E+04** | **1.33E+04** | **1.33E+04** | **1.33E+04** | **1.33E+04** |
| | gap | Best | **0.00%** | **0.00%** | **0.00%** | **0.00%** | **0.00%** | **0.00%** | **0.00%** | **0.00%** |
| | | Mean | **0.00%** | **0.00%** | **0.00%** | **0.00%** | **0.00%** | **0.00%** | **0.00%** | **0.00%** |
| QMKP13 | obj | Best | 5.84E+03 | 9.95E+03 | 4.85E+03 | 9.82E+03 | 9.49E+03 | **1.07E+04** | 9.07E+03 | 1.04E+04 |
| | | Mean | 6.48E+03 | 9.48E+03 | 4.85E+03 | 9.04E+03 | 8.76E+03 | **9.80E+03** | 8.54E+03 | 9.52E+03 |
| | gap | Best | 102.82% | 40.84% | 189.27% | 55.91% | 59.90% | **31.39%** | 54.54% | 34.73% |
| | | Mean | 117.77% | 47.94% | 189.27% | 72.13% | 60.64% | **43.39%** | 64.62% | 47.83% |
| QMKP14 | obj | Best | 1.93E+04 | 1.95E+04 | 1.93E+04 | 1.94E+04 | 1.95E+04 | **1.95E+04** | 1.94E+04 | 1.95E+04 |
| | | Mean | 1.93E+04 | 1.95E+04 | 1.93E+04 | 1.92E+04 | 1.94E+04 | **1.95E+04** | 1.89E+04 | 1.91E+04 |
| | gap | Best | 1.23% | 0.00% | 1.26% | 1.75% | 0.89% | **0.00%** | 0.64% | 0.36% |
| | | Mean | 1.23% | 0.32% | 1.26% | 2.93% | 0.89% | **0.31%** | 3.64% | 2.13% |
| QMKP15 | obj | Best | 8.97E+03 | 1.33E+04 | 8.48E+03 | 1.29E+04 | 1.20E+04 | 1.33E+04 | 1.26E+04 | **1.34E+04** |
| | | Mean | 8.97E+03 | 1.26E+04 | 8.33E+03 | 1.20E+04 | 1.13E+04 | **1.28E+04** | 1.14E+04 | 1.26E+04 |
| | gap | Best | 88.08% | 26.93% | 98.95% | 40.98% | 48.93% | 26.75% | 33.75% | **26.04%** |
| | | Mean | 88.08% | 34.21% | 102.72% | 54.96% | 49.37% | **31.66%** | 49.27% | 34.02% |
| QMKP16 | obj | Best | 9.84E+03 | 1.46E+04 | 1.01E+04 | 1.50E+04 | 1.32E+04 | 1.48E+04 | 1.31E+04 | **1.52E+04** |
| | | Mean | 9.84E+03 | 1.44E+04 | 1.01E+04 | 1.32E+04 | 1.20E+04 | **1.43E+04** | 1.25E+04 | 1.42E+04 |
| | gap | Best | 134.14% | 58.04% | 128.68% | 76.23% | 91.33% | 55.55% | 75.41% | **51.24%** |
| | | Mean | 134.14% | 60.51% | 128.68% | 103.42% | 92.64% | **60.99%** | 84.18% | 62.88% |
| QMKP17 | obj | Best | **3.35E+04** | **3.35E+04** | 3.32E+04 | **3.35E+04** | **3.35E+04** | **3.35E+04** | **3.35E+04** | **3.35E+04** |
| | | Mean | **3.35E+04** | **3.35E+04** | 3.32E+04 | **3.35E+04** | **3.35E+04** | **3.35E+04** | **3.35E+04** | **3.35E+04** |
| | gap | Best | **0.00%** | **0.00%** | 0.82% | **0.00%** | **0.00%** | **0.00%** | **0.00%** | **0.00%** |
| | | Mean | **0.00%** | **0.00%** | 0.82% | **0.00%** | **0.00%** | **0.00%** | **0.00%** | **0.00%** |
| QMKP18 | obj | Best | **3.16E+04** | **3.16E+04** | 3.11E+04 | 3.16E+04 | 3.13E+04 | **3.16E+04** | **3.16E+04** | **3.16E+04** |
| | | Mean | **3.16E+04** | 3.15E+04 | 3.11E+04 | 3.13E+04 | 3.11E+04 | 3.15E+04 | 3.10E+04 | 3.12E+04 |
| | gap | Best | **0.00%** | **0.00%** | 1.36% | 0.89% | 1.41% | **0.00%** | **0.00%** | **0.00%** |
| | | Mean | **0.00%** | 0.20% | 1.36% | 1.72% | 1.41% | 0.12% | 1.80% | 1.22% |
| QMKP19 | obj | Best | **1.55E+04** | **1.55E+04** | **1.55E+04** | **1.55E+04** | **1.55E+04** | **1.55E+04** | **1.55E+04** | **1.55E+04** |
| | | Mean | **1.55E+04** | **1.55E+04** | **1.55E+04** | **1.55E+04** | **1.55E+04** | **1.55E+04** | 1.55E+04 | 1.55E+04 |
| | gap | Best | **0.00%** | **0.00%** | **0.00%** | **0.00%** | **0.00%** | **0.00%** | **0.00%** | **0.00%** |
| | | Mean | **0.00%** | **0.00%** | **0.00%** | **0.00%** | **0.00%** | **0.00%** | 0.02% | 0.04% |
| QMKP20 | obj | Best | 1.05E+04 | **1.15E+04** | 8.42E+03 | 1.13E+04 | 1.14E+04 | 1.13E+04 | 1.09E+04 | 1.15E+04 |
| | | Mean | 1.05E+04 | 1.11E+04 | 8.42E+03 | 1.11E+04 | 1.09E+04 | **1.12E+04** | 1.05E+04 | 1.11E+04 |
| | gap | Best | 27.50% | **16.31%** | 58.78% | 20.32% | 22.26% | 18.38% | 22.35% | 16.66% |
| | | Mean | 27.50% | 20.10% | 58.86% | 23.42% | 22.36% | **19.38%** | 27.03% | 20.57% |
| QMKP21 | obj | Best | 1.00E+04 | 1.07E+04 | 8.25E+03 | 1.06E+04 | 1.05E+04 | 1.01E+04 | 1.02E+04 | **1.08E+04** |
| | | Mean | 1.00E+04 | 1.02E+04 | 8.16E+03 | 1.03E+04 | 1.00E+04 | 9.99E+03 | 9.98E+03 | **1.04E+04** |
| | gap | Best | 17.87% | 10.21% | 43.07% | 14.39% | 17.74% | 16.82% | 15.37% | **9.38%** |
| | | Mean | 17.87% | 15.97% | 44.64% | 22.59% | 17.82% | 18.13% | 18.30% | **13.27%** |

| Pro. | Metric | Status | GUROBI | OR-TOOLS | SCIP | SA | VNS | LNS | TS | GA |
|---|---|---|---|---|---|---|---|---|---|---|
| QMKP22 | obj | Best | 1.03E+04 | 1.45E+04 | 9.69E+03 | 1.53E+04 | 1.38E+04 | **1.51E+04** | 1.42E+04 | 1.50E+04 |
| | | Mean | 1.03E+04 | 1.40E+04 | 9.57E+03 | 1.39E+04 | 1.30E+04 | 1.44E+04 | 1.32E+04 | **1.45E+04** |
| | gap | Best | 121.29% | 57.12% | 135.37% | 65.60% | 74.91% | **51.33%** | 61.15% | 52.37% |
| | | Mean | 121.29% | 62.73% | 138.52% | 84.66% | 75.38% | 58.22% | 73.55% | **57.71%** |
| QMKP23 | obj | Best | 3.73E+03 | 6.90E+03 | 3.87E+03 | 6.69E+03 | 6.37E+03 | **7.66E+03** | 6.82E+03 | 6.81E+03 |
| | | Mean | 3.73E+03 | 6.35E+03 | 3.87E+03 | 6.23E+03 | 6.11E+03 | **7.13E+03** | 6.44E+03 | 6.49E+03 |
| | gap | Best | 308.57% | 121.02% | 294.21% | 145.37% | 149.53% | **99.09%** | 123.45% | 123.77% |
| | | Mean | 308.57% | 140.64% | 294.21% | 160.87% | 149.68% | **114.85%** | 137.53% | 135.66% |
| QMKP24 | obj | Best | 1.68E+04 | 1.80E+04 | 1.45E+04 | 1.79E+04 | 1.79E+04 | 1.82E+04 | 1.71E+04 | **1.83E+04** |
| | | Mean | 1.68E+04 | **1.78E+04** | 1.45E+04 | 1.73E+04 | 1.76E+04 | 1.78E+04 | 1.64E+04 | 1.78E+04 |
| | gap | Best | 49.56% | 39.39% | 73.17% | 45.43% | 42.78% | 38.20% | 47.06% | **37.26%** |
| | | Mean | 49.56% | **40.77%** | 73.17% | 52.36% | 42.79% | 41.12% | 52.82% | 41.18% |
| QMKP25 | obj | Best | **4.77E+04** | **4.77E+04** | **4.77E+04** | **4.77E+04** | **4.77E+04** | **4.77E+04** | **4.77E+04** | **4.77E+04** |
| | | Mean | **4.77E+04** | **4.77E+04** | **4.77E+04** | **4.77E+04** | **4.77E+04** | **4.77E+04** | **4.77E+04** | **4.77E+04** |
| | gap | Best | **0.00%** | **0.00%** | **0.00%** | **0.00%** | **0.00%** | **0.00%** | **0.00%** | **0.00%** |
| | | Mean | **0.00%** | **0.00%** | **0.00%** | **0.00%** | **0.00%** | **0.00%** | **0.00%** | **0.00%** |
| QMKP26 | obj | Best | 2.88E+04 | 2.98E+04 | 2.16E+04 | 2.96E+04 | 2.96E+04 | 2.98E+04 | 2.85E+04 | **2.98E+04** |
| | | Mean | 2.88E+04 | 2.97E+04 | 2.16E+04 | 2.91E+04 | 2.89E+04 | 2.97E+04 | 2.78E+04 | **2.97E+04** |
| | gap | Best | 18.41% | 14.30% | 57.71% | 17.35% | 18.05% | 14.30% | 19.51% | **14.30%** |
| | | Mean | 18.41% | 15.04% | 57.71% | 19.75% | 18.10% | 14.97% | 22.91% | **14.94%** |
| QMKP27 | obj | Best | 2.94E+04 | 2.99E+04 | 2.89E+04 | 2.97E+04 | 2.96E+04 | **3.00E+04** | 2.92E+04 | 3.00E+04 |
| | | Mean | 2.94E+04 | 2.97E+04 | 2.88E+04 | 2.93E+04 | 2.89E+04 | **3.00E+04** | 2.88E+04 | 2.98E+04 |
| | gap | Best | 22.37% | 20.40% | 24.42% | 22.80% | 24.35% | **19.81%** | 23.15% | 19.92% |
| | | Mean | 22.37% | 21.06% | 24.99% | 25.85% | 24.39% | **20.13%** | 24.92% | 20.71% |
| QMKP28 | obj | Best | 1.15E+04 | 1.22E+04 | 8.59E+03 | 1.19E+04 | 1.15E+04 | 1.20E+04 | 1.17E+04 | **1.23E+04** |
| | | Mean | 1.15E+04 | 1.15E+04 | 8.59E+03 | 1.11E+04 | 1.10E+04 | 1.16E+04 | 1.06E+04 | **1.19E+04** |
| | gap | Best | 25.83% | 19.09% | 68.94% | 31.11% | 31.27% | 20.63% | 24.01% | **18.00%** |
| | | Mean | 25.83% | 25.87% | 68.94% | 37.64% | 31.50% | 25.46% | 37.79% | **21.63%** |
| QMKP29 | obj | Best | **1.97E+04** | **1.97E+04** | 1.95E+04 | 1.97E+04 | **1.97E+04** | **1.97E+04** | **1.97E+04** | **1.97E+04** |
| | | Mean | **1.97E+04** | **1.97E+04** | 1.94E+04 | 1.97E+04 | **1.97E+04** | **1.97E+04** | 1.97E+04 | 1.97E+04 |
| | gap | Best | **0.00%** | **0.00%** | 1.24% | 0.01% | **0.00%** | **0.00%** | **0.00%** | **0.00%** |
| | | Mean | **0.00%** | **0.00%** | 1.34% | 0.05% | **0.00%** | **0.00%** | 0.29% | 0.07% |
| QMKP30 | obj | Best | 1.44E+04 | 1.47E+04 | 1.30E+04 | 1.45E+04 | 1.48E+04 | **1.47E+04** | 1.43E+04 | 1.47E+04 |
| | | Mean | 1.44E+04 | 1.44E+04 | 1.30E+04 | 1.41E+04 | **1.46E+04** | 1.45E+04 | 1.38E+04 | 1.45E+04 |
| | gap | Best | 6.96% | 5.31% | 19.01% | 9.27% | 5.58% | **4.92%** | 7.64% | 5.11% |
| | | Mean | 6.96% | 7.01% | 19.01% | 11.75% | **5.59%** | 6.52% | 12.34% | 6.37% |
| QMKP31 | obj | Best | 2.14E+04 | 2.26E+04 | 2.05E+04 | 2.31E+04 | 2.32E+04 | 2.33E+04 | 2.27E+04 | **2.33E+04** |
| | | Mean | 2.14E+04 | 2.22E+04 | 1.99E+04 | 2.28E+04 | 2.29E+04 | 2.29E+04 | 2.21E+04 | **2.31E+04** |
| | gap | Best | 35.48% | 28.58% | 41.83% | 27.43% | 26.89% | 24.83% | 27.86% | **24.69%** |
| | | Mean | 35.48% | 30.96% | 46.52% | 30.90% | 26.91% | 27.14% | 31.69% | **25.91%** |
| QMKP32 | obj | Best | 2.61E+04 | 2.68E+04 | 2.52E+04 | 2.72E+04 | 2.71E+04 | 2.72E+04 | 2.65E+04 | **2.72E+04** |
| | | Mean | 2.61E+04 | 2.65E+04 | 2.52E+04 | 2.64E+04 | 2.68E+04 | 2.68E+04 | 2.62E+04 | **2.70E+04** |
| | gap | Best | 13.17% | 10.08% | 17.45% | 11.80% | 10.41% | 8.80% | 11.44% | **8.63%** |
| | | Mean | 13.17% | 11.58% | 17.45% | 13.22% | 10.42% | 10.05% | 12.95% | **9.55%** |
| QMKP33 | obj | Best | 2.50E+04 | 2.58E+04 | 2.20E+04 | 2.56E+04 | 2.57E+04 | **2.60E+04** | 2.56E+04 | 2.57E+04 |
| | | Mean | 2.50E+04 | 2.56E+04 | 2.20E+04 | 2.53E+04 | 2.55E+04 | **2.57E+04** | 2.45E+04 | 2.56E+04 |
| | gap | Best | 22.20% | 18.19% | 38.50% | 20.78% | 19.76% | **17.36%** | 19.02% | 18.52% |

| Pro. | Metric | Status | GUROBI | OR-TOOLS | SCIP | SA | VNS | LNS | TS | GA |
|---|---|---|---|---|---|---|---|---|---|---|
| | | Mean | 22.20% | 18.95% | 38.50% | 22.37% | 19.77% | **18.84%** | 24.47% | 19.17% |
| QMKP34 | obj | Best | **5.13E+04** | **5.13E+04** | 5.11E+04 | **5.13E+04** | **5.13E+04** | **5.13E+04** | **5.13E+04** | **5.13E+04** |
| | | Mean | **5.13E+04** | **5.13E+04** | 5.01E+04 | **5.13E+04** | **5.13E+04** | **5.13E+04** | 5.11E+04 | **5.13E+04** |
| | gap | Best | **0.00%** | **0.00%** | 0.33% | **0.00%** | **0.00%** | **0.00%** | **0.00%** | **0.00%** |
| | | Mean | **0.00%** | **0.00%** | 2.37% | **0.00%** | **0.00%** | **0.00%** | 0.23% | **0.00%** |
| QMKP35 | obj | Best | 7.24E+03 | 1.61E+04 | 7.38E+03 | 1.55E+04 | 1.16E+04 | **1.82E+04** | 1.69E+04 | 1.62E+04 |
| | | Mean | 7.24E+03 | 1.45E+04 | 7.38E+03 | 1.36E+04 | 1.09E+04 | **1.61E+04** | 1.45E+04 | 1.51E+04 |
| | gap | Best | 458.11% | 151.10% | 447.45% | 198.21% | 269.36% | **121.70%** | 139.07% | 149.83% |
| | | Mean | 458.11% | 180.15% | 447.45% | 237.23% | 270.76% | **152.57%** | 186.70% | 167.49% |
| QMKP36 | obj | Best | **5.07E+04** | **5.07E+04** | 5.06E+04 | 5.07E+04 | 5.07E+04 | **5.07E+04** | **5.07E+04** | **5.07E+04** |
| | | Mean | **5.07E+04** | **5.07E+04** | 5.06E+04 | 5.07E+04 | 5.07E+04 | **5.07E+04** | 5.07E+04 | **5.07E+04** |
| | gap | Best | **0.00%** | **0.00%** | 0.16% | 0.02% | 0.05% | **0.00%** | **0.00%** | **0.00%** |
| | | Mean | **0.00%** | **0.00%** | 0.16% | 0.12% | 0.05% | **0.00%** | 0.07% | **0.00%** |
| QMKP37 | obj | Best | **2.10E+04** | **2.10E+04** | 2.08E+04 | **2.10E+04** | **2.10E+04** | **2.10E+04** | **2.10E+04** | **2.10E+04** |
| | | Mean | **2.10E+04** | **2.10E+04** | 2.08E+04 | **2.10E+04** | **2.10E+04** | **2.10E+04** | 2.08E+04 | **2.10E+04** |
| | gap | Best | **0.00%** | **0.00%** | 0.92% | **0.00%** | **0.00%** | **0.00%** | **0.00%** | **0.00%** |
| | | Mean | **0.00%** | **0.00%** | 0.92% | **0.00%** | **0.00%** | **0.00%** | 0.89% | **0.00%** |
| QMKP38 | obj | Best | 1.95E+04 | **1.97E+04** | 1.83E+04 | 1.96E+04 | 1.97E+04 | **1.97E+04** | 1.91E+04 | **1.97E+04** |
| | | Mean | 1.95E+04 | 1.96E+04 | 1.82E+04 | 1.95E+04 | **1.96E+04** | 1.96E+04 | 1.85E+04 | 1.96E+04 |
| | gap | Best | 0.64% | **0.00%** | 7.14% | 0.66% | 0.22% | **0.00%** | 2.66% | **0.00%** |
| | | Mean | 0.64% | 0.24% | 7.93% | 1.21% | **0.22%** | 0.33% | 6.36% | 0.45% |
| QMKP39 | obj | Best | 8.37E+03 | **8.89E+03** | 5.30E+03 | 8.85E+03 | 8.05E+03 | 8.62E+03 | 8.51E+03 | 8.77E+03 |
| | | Mean | 8.37E+03 | 7.87E+03 | 5.30E+03 | 7.63E+03 | 7.03E+03 | 8.31E+03 | 7.04E+03 | **8.52E+03** |
| | gap | Best | 72.01% | **61.81%** | 171.77% | 90.79% | 104.73% | 66.86% | 69.19% | 64.03% |
| | | Mean | 72.01% | 84.32% | 171.77% | 112.43% | 105.77% | 73.30% | 108.30% | **69.09%** |
| QMKP40 | obj | Best | NaN | 9.84E+03 | 5.60E+03 | 1.06E+04 | 9.02E+03 | 1.13E+04 | 1.08E+04 | **1.13E+04** |
| | | Mean | NaN | 8.86E+03 | 5.60E+03 | 1.01E+04 | 8.41E+03 | 1.02E+04 | 9.42E+03 | **1.03E+04** |
| | gap | Best | NaN | 198.10% | 423.75% | 190.51% | 248.77% | 158.94% | 170.47% | **159.17%** |
| | | Mean | NaN | 232.63% | 423.75% | 207.09% | 250.13% | 189.63% | 215.82% | **186.15%** |
| QMKP41 | obj | Best | **3.92E+04** | **3.92E+04** | 3.92E+04 | **3.92E+04** | **3.92E+04** | **3.92E+04** | 3.92E+04 | **3.92E+04** |
| | | Mean | **3.92E+04** | **3.92E+04** | 3.90E+04 | 3.92E+04 | **3.92E+04** | **3.92E+04** | 3.91E+04 | **3.92E+04** |
| | gap | Best | **0.00%** | **0.00%** | 0.06% | **0.00%** | **0.00%** | **0.00%** | 0.01% | **0.00%** |
| | | Mean | **0.00%** | **0.00%** | 0.44% | 0.01% | **0.00%** | **0.00%** | 0.32% | **0.00%** |
| QMKP42 | obj | Best | 2.30E+04 | 2.55E+04 | 1.69E+04 | 2.50E+04 | 2.46E+04 | 2.56E+04 | 2.43E+04 | **2.56E+04** |
| | | Mean | 2.30E+04 | 2.51E+04 | 1.69E+04 | 2.46E+04 | 2.43E+04 | 2.53E+04 | 2.32E+04 | **2.54E+04** |
| | gap | Best | 53.94% | 38.73% | 109.05% | 43.52% | 45.53% | 38.04% | 45.30% | **37.87%** |
| | | Mean | 53.94% | 40.93% | 109.54% | 49.25% | 45.55% | 39.84% | 52.81% | **38.90%** |
| QMKP43 | obj | Best | **6.76E+04** | **6.76E+04** | **6.76E+04** | **6.76E+04** | **6.76E+04** | **6.76E+04** | **6.76E+04** | **6.76E+04** |
| | | Mean | **6.76E+04** | **6.76E+04** | **6.76E+04** | **6.76E+04** | **6.76E+04** | **6.76E+04** | **6.76E+04** | **6.76E+04** |
| | gap | Best | **0.00%** | **0.00%** | **0.00%** | **0.00%** | **0.00%** | **0.00%** | **0.00%** | **0.00%** |
| | | Mean | **0.00%** | **0.00%** | **0.00%** | **0.00%** | **0.00%** | **0.00%** | **0.00%** | **0.00%** |
| QMKP44 | obj | Best | **6.28E+04** | **6.28E+04** | **6.28E+04** | **6.28E+04** | **6.28E+04** | **6.28E+04** | **6.28E+04** | **6.28E+04** |
| | | Mean | **6.28E+04** | **6.28E+04** | 6.28E+04 | **6.28E+04** | **6.28E+04** | **6.28E+04** | **6.28E+04** | **6.28E+04** |
| | gap | Best | **0.00%** | **0.00%** | **0.00%** | **0.00%** | **0.00%** | **0.00%** | **0.00%** | **0.00%** |
| | | Mean | **0.00%** | **0.00%** | 0.05% | **0.00%** | **0.00%** | **0.00%** | **0.00%** | **0.00%** |
| QMKP45 | obj | Best | 4.19E+04 | 4.38E+04 | 4.28E+04 | 4.41E+04 | 4.41E+04 | **4.42E+04** | 4.30E+04 | 4.41E+04 |
| | | Mean | 4.19E+04 | 4.37E+04 | 4.17E+04 | 4.35E+04 | 4.38E+04 | **4.41E+04** | 4.18E+04 | 4.40E+04 |

| Pro. | Metric | Status | GUROBI | OR-TOOLS | SCIP | SA | VNS | LNS | TS | GA |
|---|---|---|---|---|---|---|---|---|---|---|
| | gap | Best | 34.12% | 28.34% | 31.30% | 29.17% | 28.33% | **27.29%** | 30.86% | 27.39% |
| | | Mean | 34.12% | 28.75% | 35.17% | 31.75% | 28.34% | **27.52%** | 34.62% | 27.89% |

## 3.8 High school timetabling problem (HTS)

Table S-18 shows the experimental results of the HTS test suit.

**Table S-18** Experimental results on HTS test suit.

| Pro. | Metric | Status | GUROBI | OR-TOOLS | SCIP | SA | VNS | LNS | TS | GA |
|---|---|---|---|---|---|---|---|---|---|---|
| HTS01 | obj | Best | 7.11E+02 | 7.73E+02 | NAN | 7.20E+02 | 7.16E+02 | 7.07E+02 | 7.26E+02 | **7.04E+02** |
| | | Mean | 7.44E+02 | 7.84E+02 | NAN | 7.28E+02 | 7.32E+02 | **7.15E+02** | 7.40E+02 | 7.19E+02 |
| | gap | Best | 8.16% | 15.52% | NAN | 9.31% | 8.80% | 7.64% | 10.06% | **7.24%** |
| | | Mean | 12.06% | 16.68% | NAN | 10.34% | 10.80% | **8.69%** | 11.72% | 9.16% |
| HTS02 | obj | Best | 7.34E+02 | 7.84E+02 | NAN | 7.27E+02 | 7.29E+02 | **7.14E+02** | 7.33E+02 | 7.15E+02 |
| | | Mean | 7.34E+02 | 8.09E+02 | NAN | 7.34E+02 | 7.34E+02 | 7.21E+02 | 7.38E+02 | **7.16E+02** |
| | gap | Best | 7.77% | 13.65% | NAN | 6.88% | 7.13% | **5.18%** | 7.64% | 5.31% |
| | | Mean | 7.77% | 16.27% | NAN | 7.79% | 7.79% | 6.15% | 8.24% | 5.42% |
| HTS03 | obj | Best | 8.37E+02 | 8.79E+02 | NAN | 7.33E+02 | 7.33E+02 | 7.27E+02 | 7.34E+02 | **7.22E+02** |
| | | Mean | 8.37E+02 | 9.17E+02 | NAN | 7.36E+02 | 7.38E+02 | 7.30E+02 | 7.36E+02 | **7.25E+02** |
| | gap | Best | 14.70% | 18.77% | NAN | 2.59% | 2.59% | 1.79% | 2.72% | **1.11%** |
| | | Mean | 14.70% | 22.10% | NAN | 2.99% | 3.20% | 2.16% | 2.99% | **1.46%** |
| HTS04 | obj | Best | 8.68E+02 | 8.73E+02 | NAN | 7.38E+02 | 7.45E+02 | **7.34E+02** | 7.51E+02 | 7.40E+02 |
| | | Mean | NAN | 9.26E+02 | NAN | 7.47E+02 | 7.50E+02 | 7.42E+02 | 7.53E+02 | **7.40E+02** |
| | gap | Best | 16.59% | 17.07% | NAN | 1.90% | 2.82% | **1.36%** | 3.60% | 2.16% |
| | | Mean | NAN | 21.73% | NAN | 3.02% | 3.46% | 2.37% | 3.85% | **2.21%** |
| HTS05 | obj | Best | 6.82E+02 | 6.86E+02 | NAN | 6.23E+02 | 6.29E+02 | **6.18E+02** | 6.31E+02 | 6.20E+02 |
| | | Mean | 6.82E+02 | 6.94E+02 | NAN | 6.29E+02 | 6.31E+02 | 6.29E+02 | 6.33E+02 | **6.26E+02** |
| | gap | Best | 10.12% | 10.64% | NAN | 1.61% | 2.54% | **0.81%** | 2.85% | 1.13% |
| | | Mean | 10.12% | 11.69% | NAN | 2.51% | 2.88% | 2.53% | 3.22% | **2.01%** |
| HTS06 | obj | Best | 8.70E+02 | 9.22E+02 | NAN | 8.17E+02 | 8.18E+02 | **8.02E+02** | 8.26E+02 | 8.08E+02 |
| | | Mean | 8.70E+02 | 9.43E+02 | NAN | 8.27E+02 | 8.22E+02 | **8.10E+02** | 8.29E+02 | 8.11E+02 |
| | gap | Best | 13.68% | 18.55% | NAN | 8.08% | 8.19% | **6.36%** | 9.08% | 7.05% |
| | | Mean | 13.68% | 20.38% | NAN | 9.23% | 8.59% | **7.25%** | 9.45% | 7.44% |
| HTS07 | obj | Best | 1.30E+03 | 1.35E+03 | NAN | 1.22E+03 | 1.23E+03 | **1.21E+03** | 1.23E+03 | 1.23E+03 |
| | | Mean | 1.30E+03 | 1.38E+03 | NAN | 1.23E+03 | 1.23E+03 | **1.21E+03** | 1.23E+03 | 1.23E+03 |
| | gap | Best | 7.99% | 11.19% | NAN | 1.96% | 2.36% | **0.99%** | 2.60% | 2.52% |
| | | Mean | 7.99% | 13.07% | NAN | 2.53% | 2.73% | **1.36%** | 2.89% | 2.63% |
| HTS08 | obj | Best | 6.79E+02 | 6.93E+02 | 7.26E+02 | 6.60E+02 | 6.62E+02 | **6.38E+02** | 6.77E+02 | 6.53E+02 |
| | | Mean | 6.79E+02 | 7.07E+02 | 7.31E+02 | 6.69E+02 | 6.73E+02 | **6.42E+02** | 6.82E+02 | 6.65E+02 |
| | gap | Best | 8.84% | 10.68% | 14.74% | 6.21% | 6.50% | **2.98%** | 8.57% | 5.21% |
| | | Mean | 8.84% | 12.38% | 15.34% | 7.43% | 8.01% | **3.58%** | 9.29% | 6.85% |
| HTS09 | obj | Best | 8.65E+02 | 9.05E+02 | NAN | 8.19E+02 | 8.17E+02 | 8.15E+02 | 8.24E+02 | **8.13E+02** |
| | | Mean | 8.65E+02 | 9.27E+02 | NAN | 8.22E+02 | 8.19E+02 | 8.23E+02 | 8.26E+02 | **8.15E+02** |
| | gap | Best | 9.25% | 13.26% | NAN | 4.15% | 3.92% | 3.68% | 4.73% | **3.44%** |
| | | Mean | 9.25% | 15.27% | NAN | 4.48% | 4.15% | 4.59% | 4.96% | **3.70%** |
| HTS10 | obj | Best | 3.06E+02 | 3.15E+02 | NAN | 3.11E+02 | 3.13E+02 | **3.00E+02** | 3.12E+02 | 3.04E+02 |
| | | Mean | 3.06E+02 | 3.32E+02 | NAN | 3.13E+02 | 3.13E+02 | **3.06E+02** | 3.16E+02 | 3.11E+02 |

| Pro. | Metric | Status | GUROBI | OR-TOOLS | SCIP | SA | VNS | LNS | TS | GA |
|---|---|---|---|---|---|---|---|---|---|---|
| | gap | Best | 2.61% | 5.40% | NAN | 4.18% | 4.79% | **0.67%** | 4.49% | 1.97% |
| | | Mean | 2.61% | 10.13% | NAN | 4.91% | 4.91% | **2.58%** | 5.81% | 4.10% |
| HTS11 | obj | Best | NAN | 1.13E+03 | NAN | 9.87E+02 | 1.00E+03 | **9.76E+02** | 1.01E+03 | 9.89E+02 |
| | | Mean | NAN | 1.21E+03 | NAN | 1.01E+03 | 1.01E+03 | **9.88E+02** | 1.02E+03 | 9.96E+02 |
| | gap | Best | NAN | 15.78% | NAN | 3.24% | 4.50% | **2.15%** | 5.54% | 3.44% |
| | | Mean | NAN | 20.91% | NAN | 5.06% | 5.37% | **3.29%** | 6.29% | 4.11% |
| HTS12 | obj | Best | 1.05E+03 | 1.08E+03 | NAN | 1.02E+03 | 1.02E+03 | **1.01E+03** | 1.03E+03 | **1.01E+03** |
| | | Mean | 1.06E+03 | 1.09E+03 | NAN | 1.03E+03 | 1.03E+03 | 1.02E+03 | 1.04E+03 | **1.02E+03** |
| | gap | Best | 10.55% | 12.55% | NAN | 7.29% | 7.56% | **6.83%** | 8.99% | **6.83%** |
| | | Mean | 11.49% | 13.62% | NAN | 8.21% | 8.30% | 7.72% | 9.40% | **7.38%** |
| HTS13 | obj | Best | 2.76E+02 | 2.76E+02 | 2.76E+02 | 2.44E+02 | 2.51E+02 | **2.42E+02** | 2.53E+02 | 2.46E+02 |
| | | Mean | 2.76E+02 | 2.76E+02 | 2.76E+02 | 2.53E+02 | 2.53E+02 | **2.49E+02** | 2.60E+02 | 2.57E+02 |
| | gap | Best | 14.49% | 14.49% | 14.49% | 3.28% | 5.98% | **2.48%** | 6.72% | 4.07% |
| | | Mean | 14.49% | 14.49% | 14.49% | 6.81% | 6.64% | **5.28%** | 9.28% | 8.11% |
| HTS14 | obj | Best | 1.00E+03 | 1.01E+03 | NAN | 9.22E+02 | 9.21E+02 | **9.17E+02** | 9.35E+02 | 9.22E+02 |
| | | Mean | 1.00E+03 | 1.01E+03 | NAN | 9.32E+02 | 9.26E+02 | 9.24E+02 | 9.39E+02 | **9.24E+02** |
| | gap | Best | 9.00% | 9.81% | NAN | 1.30% | 1.19% | **0.76%** | 2.67% | 1.30% |
| | | Mean | 9.00% | 10.29% | NAN | 2.40% | 1.75% | 1.53% | 3.07% | **1.49%** |
| HTS15 | obj | Best | 2.57E+02 | 2.57E+02 | 2.57E+02 | 2.35E+02 | **2.34E+02** | **2.34E+02** | 2.35E+02 | 2.35E+02 |
| | | Mean | 2.57E+02 | 2.57E+02 | 2.57E+02 | 2.36E+02 | **2.34E+02** | 2.35E+02 | 2.36E+02 | 2.35E+02 |
| | gap | Best | 15.56% | 15.56% | 15.56% | 7.66% | **7.26%** | **7.26%** | 7.66% | 7.66% |
| | | Mean | 15.56% | 15.56% | 15.56% | 7.97% | **7.42%** | 7.74% | 8.05% | 7.66% |
| HTS16 | obj | Best | 5.00E+02 | 5.29E+02 | NAN | 4.77E+02 | 4.81E+02 | **4.75E+02** | 4.83E+02 | 4.77E+02 |
| | | Mean | 5.01E+02 | 5.37E+02 | NAN | 4.80E+02 | 4.85E+02 | **4.78E+02** | 4.92E+02 | 4.78E+02 |
| | gap | Best | 6.00% | 11.15% | NAN | 1.47% | 2.29% | **1.05%** | 2.69% | 1.47% |
| | | Mean | 6.15% | 12.38% | NAN | 2.16% | 3.05% | **1.59%** | 4.53% | 1.76% |
| HTS17 | obj | Best | 4.88E+02 | 5.08E+02 | NAN | 4.58E+02 | 4.58E+02 | **4.56E+02** | 4.60E+02 | 4.57E+02 |
| | | Mean | 5.10E+02 | 5.13E+02 | NAN | 4.62E+02 | 4.61E+02 | 4.60E+02 | 4.65E+02 | **4.58E+02** |
| | gap | Best | 6.56% | 10.24% | NAN | 0.44% | 0.44% | **0.00%** | 0.87% | 0.22% |
| | | Mean | 10.48% | 11.16% | NAN | 1.33% | 1.08% | 0.86% | 1.84% | **0.52%** |
| HTS18 | obj | Best | 3.35E+02 | 3.30E+02 | 4.14E+02 | 3.13E+02 | 3.12E+02 | **3.11E+02** | 3.14E+02 | **3.11E+02** |
| | | Mean | 3.38E+02 | 3.44E+02 | 4.57E+02 | 3.15E+02 | 3.13E+02 | 3.14E+02 | 3.16E+02 | **3.12E+02** |
| | gap | Best | 8.66% | 7.27% | 26.09% | 2.24% | 1.92% | **1.61%** | 2.55% | **1.61%** |
| | | Mean | 9.52% | 10.98% | 32.50% | 2.92% | 2.30% | 2.48% | 3.10% | **1.98%** |
| HTS19 | obj | Best | 2.55E+02 | 2.55E+02 | 2.70E+02 | 2.47E+02 | **2.46E+02** | 2.48E+02 | 2.48E+02 | **2.46E+02** |
| | | Mean | 2.58E+02 | 2.61E+02 | 3.14E+02 | 2.49E+02 | 2.49E+02 | 2.55E+02 | 2.49E+02 | **2.47E+02** |
| | gap | Best | 9.02% | 9.02% | 14.07% | 6.07% | **5.69%** | 6.45% | 6.45% | **5.69%** |
| | | Mean | 10.14% | 11.01% | 24.92% | 6.67% | 6.95% | 8.89% | 6.90% | **5.92%** |
| HTS20 | obj | Best | 3.25E+02 | 3.38E+02 | NAN | 3.30E+02 | 3.26E+02 | **3.21E+02** | 3.40E+02 | **3.21E+02** |
| | | Mean | 3.32E+02 | 3.48E+02 | NAN | 3.34E+02 | 3.30E+02 | 3.27E+02 | 3.42E+02 | **3.26E+02** |
| | gap | Best | 3.69% | 7.40% | NAN | 5.15% | 3.99% | **2.49%** | 7.94% | **2.49%** |
| | | Mean | 5.77% | 10.01% | NAN | 6.28% | 5.19% | 4.14% | 8.58% | **4.08%** |
| HTS21 | obj | Best | 1.11E+03 | 1.13E+03 | NAN | 1.06E+03 | 1.06E+03 | 1.06E+03 | 1.07E+03 | **1.05E+03** |
| | | Mean | 1.13E+03 | 1.14E+03 | NAN | 1.07E+03 | 1.06E+03 | 1.07E+03 | 1.08E+03 | **1.06E+03** |
| | gap | Best | 5.95% | 7.70% | NAN | 1.51% | 1.14% | 1.60% | 2.89% | **0.57%** |
| | | Mean | 7.93% | 8.85% | NAN | 2.37% | 1.64% | 2.10% | 3.39% | **1.19%** |
| HTS22 | obj | Best | 7.42E+02 | 7.50E+02 | 7.87E+02 | 7.07E+02 | 7.06E+02 | 6.95E+02 | 7.05E+02 | **6.94E+02** |

| Pro. | Metric | Status | GUROBI | OR-TOOLS | SCIP | SA | VNS | LNS | TS | GA |
|---|---|---|---|---|---|---|---|---|---|---|
| | | Mean | 7.47E+02 | 7.57E+02 | 7.91E+02 | 7.09E+02 | 7.10E+02 | 7.04E+02 | 7.10E+02 | **6.98E+02** |
| | gap | Best | 7.82% | 8.80% | 13.09% | 3.25% | 3.12% | 1.58% | 2.98% | **1.44%** |
| | | Mean | 8.41% | 9.64% | 13.56% | 3.52% | 3.63% | 2.86% | 3.66% | **2.03%** |
| HTS23 | obj | Best | 2.07E+03 | 2.09E+03 | NAN | 1.89E+03 | 1.90E+03 | **1.86E+03** | 1.91E+03 | 1.92E+03 |
| | | Mean | NAN | 2.11E+03 | NAN | 1.90E+03 | 1.91E+03 | **1.89E+03** | 1.91E+03 | 1.93E+03 |
| | gap | Best | 12.31% | 13.15% | NAN | 4.07% | 4.32% | **2.47%** | 4.72% | 5.37% |
| | | Mean | NAN | 13.84% | NAN | 4.44% | 4.71% | **3.77%** | 5.02% | 5.71% |
| HTS24 | obj | Best | 2.16E+03 | 2.21E+03 | NAN | 2.05E+03 | 2.06E+03 | **2.04E+03** | 2.06E+03 | 2.13E+03 |
| | | Mean | 2.17E+03 | 2.25E+03 | NAN | 2.07E+03 | 2.07E+03 | **2.05E+03** | 2.08E+03 | 2.20E+03 |
| | gap | Best | 7.54% | 9.67% | NAN | 2.34% | 2.91% | **1.91%** | 3.10% | 5.88% |
| | | Mean | 7.84% | 11.19% | NAN | 3.26% | 3.23% | **2.59%** | 3.76% | 9.15% |
| HTS25 | obj | Best | 9.70E+02 | 1.07E+03 | NAN | 9.61E+02 | 9.51E+02 | **9.43E+02** | 9.69E+02 | **9.43E+02** |
| | | Mean | 1.00E+03 | 1.11E+03 | NAN | 9.64E+02 | 9.57E+02 | **9.50E+02** | 9.77E+02 | 9.55E+02 |
| | gap | Best | 4.85% | 13.74% | NAN | 3.95% | 2.94% | **2.12%** | 4.75% | **2.12%** |
| | | Mean | 7.72% | 17.00% | NAN | 4.27% | 3.57% | **2.86%** | 5.48% | 3.33% |
| HTS26 | obj | Best | 5.90E+02 | 6.31E+02 | 7.21E+02 | 5.83E+02 | 5.89E+02 | **5.86E+02** | 6.04E+02 | 5.92E+02 |
| | | Mean | 6.27E+02 | 6.47E+02 | 7.51E+02 | 5.95E+02 | 5.96E+02 | **5.93E+02** | 6.08E+02 | **5.93E+02** |
| | gap | Best | 3.22% | 9.51% | 20.80% | 2.06% | 3.06% | **2.56%** | 5.46% | 3.55% |
| | | Mean | 8.85% | 11.70% | 23.67% | 4.09% | 4.25% | **3.77%** | 6.02% | **3.77%** |
| HTS27 | obj | Best | 5.56E+02 | 5.77E+02 | 6.13E+02 | 5.54E+02 | 5.51E+02 | 5.53E+02 | 5.53E+02 | **5.50E+02** |
| | | Mean | 5.61E+02 | 5.88E+02 | 6.13E+02 | 5.57E+02 | 5.55E+02 | 5.55E+02 | 5.57E+02 | **5.52E+02** |
| | gap | Best | 1.80% | 5.37% | 10.93% | 1.44% | 0.91% | 1.27% | 1.27% | **0.73%** |
| | | Mean | 2.64% | 7.20% | 10.99% | 1.94% | 1.69% | 1.55% | 2.01% | **1.05%** |
| HTS28 | obj | Best | NAN | 1.39E+03 | NAN | 1.10E+03 | 1.11E+03 | **1.10E+03** | 1.11E+03 | 1.10E+03 |
| | | Mean | NAN | 1.43E+03 | NAN | 1.11E+03 | 1.11E+03 | 1.11E+03 | 1.11E+03 | **1.10E+03** |
| | gap | Best | NAN | 22.75% | NAN | 2.54% | 3.07% | **2.37%** | 3.42% | 2.54% |
| | | Mean | NAN | 24.94% | NAN | 3.43% | 3.42% | 2.93% | 3.61% | **2.65%** |
| HTS29 | obj | Best | NAN | 1.38E+03 | NAN | 1.09E+03 | 1.09E+03 | **1.09E+03** | 1.10E+03 | 1.09E+03 |
| | | Mean | NAN | 1.51E+03 | NAN | 1.10E+03 | 1.10E+03 | 1.10E+03 | 1.10E+03 | **1.09E+03** |
| | gap | Best | NAN | 21.45% | NAN | 0.55% | 0.82% | **0.28%** | 1.00% | 0.46% |
| | | Mean | NAN | 28.14% | NAN | 1.61% | 1.48% | 1.23% | 1.67% | **0.70%** |
| HTS30 | obj | Best | 1.29E+03 | 1.41E+03 | NAN | 1.13E+03 | 1.12E+03 | **1.11E+03** | 1.13E+03 | 1.12E+03 |
| | | Mean | 1.30E+03 | 1.46E+03 | NAN | 1.14E+03 | 1.13E+03 | 1.12E+03 | 1.14E+03 | **1.12E+03** |
| | gap | Best | 14.54% | 21.69% | NAN | 2.30% | 1.16% | **0.63%** | 2.39% | 0.90% |
| | | Mean | 14.75% | 24.17% | NAN | 3.06% | 2.33% | 1.32% | 2.78% | **1.23%** |
| HTS31 | obj | Best | 1.32E+03 | 1.39E+03 | NAN | 1.14E+03 | 1.15E+03 | **1.13E+03** | 1.16E+03 | 1.14E+03 |
| | | Mean | 1.32E+03 | 1.43E+03 | NAN | 1.16E+03 | 1.16E+03 | **1.15E+03** | 1.16E+03 | 1.16E+03 |
| | gap | Best | 15.43% | 19.64% | NAN | 2.20% | 2.88% | **1.59%** | 3.89% | 2.20% |
| | | Mean | 15.57% | 21.95% | NAN | 3.66% | 4.26% | **3.16%** | 4.45% | 4.09% |
| HTS32 | obj | Best | 1.23E+03 | 1.25E+03 | NAN | 9.99E+02 | 9.95E+02 | 9.97E+02 | 9.98E+02 | **9.91E+02** |
| | | Mean | 1.23E+03 | 1.30E+03 | NAN | 1.01E+03 | 1.00E+03 | 1.00E+03 | 1.00E+03 | **1.00E+03** |
| | gap | Best | 20.08% | 21.42% | NAN | 1.60% | 1.21% | 1.40% | 1.50% | **0.81%** |
| | | Mean | 20.36% | 24.38% | NAN | 2.21% | 1.85% | 1.82% | 1.86% | **1.75%** |
| HTS33 | obj | Best | 1.15E+03 | 1.21E+03 | NAN | 1.02E+03 | 1.01E+03 | 1.00E+03 | 1.00E+03 | **1.00E+03** |
| | | Mean | 1.15E+03 | 1.25E+03 | NAN | 1.03E+03 | 1.02E+03 | **1.01E+03** | 1.03E+03 | 1.03E+03 |
| | gap | Best | 13.28% | 18.07% | NAN | 2.74% | 1.97% | 1.10% | 1.10% | **1.00%** |
| | | Mean | 13.65% | 20.52% | NAN | 3.96% | 2.92% | **1.64%** | 3.44% | 3.10% |

| Pro. | Metric | Status | GUROBI | OR-TOOLS | SCIP | SA | VNS | LNS | TS | GA |
|---|---|---|---|---|---|---|---|---|---|---|
| HTS34 | obj | Best | 1.17E+03 | 1.24E+03 | NAN | 1.01E+03 | 1.01E+03 | **9.98E+02** | 1.03E+03 | **9.98E+02** |
| | | Mean | 1.21E+03 | 1.26E+03 | NAN | 1.02E+03 | 1.02E+03 | **1.01E+03** | 1.03E+03 | 1.02E+03 |
| | gap | Best | 14.80% | 19.68% | NAN | 1.39% | 1.48% | **0.20%** | 2.83% | **0.20%** |
| | | Mean | 17.23% | 21.21% | NAN | 2.41% | 2.37% | **0.97%** | 3.24% | 2.26% |

3.9 Job shop scheduling problem (JSSP)

Table S-19 exhibits the exprimental results for JSSP problems.

**Table S-19** Experimental results on JSSP test suit.

| Pro. | Metric | Status | GUROBI | OR-TOOLS | SCIP | SA | VNS | LNS | TS | GA |
|---|---|---|---|---|---|---|---|---|---|---|
| JSSP01 | obj | Best | 1.42E+03 | **1.23E+03** | 1.33E+03 | 1.44E+03 | 1.41E+03 | 1.29E+03 | 1.49E+03 | 1.67E+03 |
| | | Mean | 1.42E+03 | **1.23E+03** | 1.33E+03 | 1.51E+03 | 1.48E+03 | 1.36E+03 | 1.57E+03 | 1.83E+03 |
| | gap | Best | 32.30% | **21.69%** | 27.35% | 32.92% | 31.39% | 25.21% | 35.17% | 42.10% |
| | | Mean | 32.30% | **21.69%** | 27.35% | 36.27% | 34.70% | 28.72% | 38.41% | 47.14% |
| JSSP02 | obj | Best | 1.51E+03 | **1.22E+03** | 1.29E+03 | 1.44E+03 | 1.36E+03 | 1.27E+03 | 1.40E+03 | 1.71E+03 |
| | | Mean | 1.51E+03 | **1.22E+03** | 1.30E+03 | 1.51E+03 | 1.43E+03 | 1.33E+03 | 1.58E+03 | 1.96E+03 |
| | gap | Best | 38.97% | **24.38%** | 28.60% | 35.82% | 32.18% | 27.42% | 33.98% | 45.98% |
| | | Mean | 38.97% | **24.38%** | 29.02% | 38.71% | 35.67% | 30.36% | 41.56% | 52.59% |
| JSSP03 | obj | Best | 1.49E+03 | **1.22E+03** | 1.29E+03 | 1.48E+03 | 1.46E+03 | 1.32E+03 | 1.43E+03 | 1.65E+03 |
| | | Mean | 1.49E+03 | **1.22E+03** | 1.29E+03 | 1.50E+03 | 1.52E+03 | 1.38E+03 | 1.52E+03 | 1.76E+03 |
| | gap | Best | 36.70% | **23.20%** | 27.30% | 36.27% | 35.75% | 28.84% | 34.40% | 42.89% |
| | | Mean | 36.70% | **23.20%** | 27.30% | 37.39% | 38.13% | 31.63% | 38.02% | 46.25% |
| JSSP04 | obj | Best | 1.44E+03 | **1.23E+03** | 1.34E+03 | 1.41E+03 | 1.33E+03 | 1.29E+03 | 1.49E+03 | 1.63E+03 |
| | | Mean | 1.44E+03 | **1.23E+03** | 1.34E+03 | 1.51E+03 | 1.43E+03 | 1.33E+03 | 1.58E+03 | 1.89E+03 |
| | gap | Best | 35.02% | **23.80%** | 30.28% | 33.50% | 29.49% | 27.41% | 37.16% | 42.53% |
| | | Mean | 35.05% | **23.80%** | 30.28% | 37.87% | 34.23% | 29.65% | 40.52% | 49.49% |
| JSSP05 | obj | Best | 1.46E+03 | **1.24E+03** | 1.30E+03 | 1.41E+03 | 1.45E+03 | 1.31E+03 | 1.55E+03 | 1.75E+03 |
| | | Mean | 1.46E+03 | **1.24E+03** | 1.30E+03 | 1.50E+03 | 1.48E+03 | 1.35E+03 | 1.66E+03 | 1.85E+03 |
| | gap | Best | 38.00% | **26.91%** | 30.18% | 35.49% | 37.41% | 30.76% | 41.45% | 48.29% |
| | | Mean | 38.00% | **26.91%** | 30.18% | 39.49% | 38.84% | 32.64% | 45.28% | 50.77% |
| JSSP06 | obj | Best | 1.80E+03 | **1.37E+03** | 3.47E+03 | 1.65E+03 | 1.52E+03 | 1.46E+03 | 1.84E+03 | 2.12E+03 |
| | | Mean | 1.80E+03 | **1.37E+03** | 3.47E+03 | 1.79E+03 | 1.67E+03 | 1.49E+03 | 1.93E+03 | 2.44E+03 |
| | gap | Best | 43.65% | **25.97%** | 70.82% | 38.52% | 33.42% | 30.73% | 44.91% | 52.15% |
| | | Mean | 43.65% | **26.02%** | 70.82% | 43.43% | 39.28% | 31.99% | 47.58% | 57.99% |
| JSSP07 | obj | Best | 1.58E+03 | **1.35E+03** | 2.42E+03 | 1.64E+03 | 1.45E+03 | 1.41E+03 | 1.66E+03 | 2.15E+03 |
| | | Mean | 1.64E+03 | **1.35E+03** | 2.42E+03 | 1.75E+03 | 1.55E+03 | 1.46E+03 | 1.77E+03 | 2.59E+03 |
| | gap | Best | 37.30% | **26.39%** | 59.16% | 39.74% | 31.91% | 29.99% | 40.47% | 53.97% |
| | | Mean | 39.78% | **26.39%** | 59.16% | 43.38% | 36.16% | 32.16% | 44.05% | 61.05% |
| JSSP08 | obj | Best | 1.81E+03 | **1.46E+03** | 1.76E+03 | 1.73E+03 | 1.68E+03 | 1.54E+03 | 1.90E+03 | 2.22E+03 |
| | | Mean | 1.81E+03 | **1.46E+03** | 1.76E+03 | 1.81E+03 | 1.73E+03 | 1.60E+03 | 2.00E+03 | 2.53E+03 |
| | gap | Best | 42.83% | **29.34%** | 41.17% | 40.29% | 38.51% | 32.92% | 45.60% | 53.41% |
| | | Mean | 42.83% | **29.34%** | 41.17% | 42.72% | 40.35% | 35.30% | 48.24% | 58.63% |
| JSSP09 | obj | Best | 1.71E+03 | **1.34E+03** | 1.80E+03 | 1.60E+03 | 1.52E+03 | 1.47E+03 | 1.67E+03 | 2.19E+03 |
| | | Mean | 1.71E+03 | **1.34E+03** | 1.80E+03 | 1.73E+03 | 1.66E+03 | 1.49E+03 | 1.86E+03 | 2.57E+03 |
| | gap | Best | 44.42% | **28.76%** | 47.17% | 40.45% | 37.60% | 35.31% | 43.16% | 56.60% |
| | | Mean | 44.42% | **29.18%** | 47.17% | 44.87% | 42.28% | 36.08% | 48.57% | 62.70% |

| Pro. | Metric | Status | GUROBI | OR-TOOLS | SCIP | SA | VNS | LNS | TS | GA |
|---|---|---|---|---|---|---|---|---|---|---|
| JSSP10 | obj | Best | 1.78E+03 | **1.35E+03** | 1.62E+03 | 1.69E+03 | 1.59E+03 | 1.44E+03 | 1.80E+03 | 2.05E+03 |
| | | Mean | 1.78E+03 | **1.36E+03** | 1.62E+03 | 1.75E+03 | 1.74E+03 | 1.46E+03 | 1.91E+03 | 2.35E+03 |
| | gap | Best | 47.98% | **31.16%** | 42.65% | 44.99% | 41.60% | 35.42% | 48.47% | 54.69% |
| | | Mean | 47.98% | **31.54%** | 42.65% | 46.83% | 46.16% | 36.51% | 51.44% | 60.02% |
| JSSP11 | obj | Best | 2.10E+03 | **1.64E+03** | 2.76E+03 | 2.03E+03 | 2.02E+03 | 1.81E+03 | 2.10E+03 | 2.77E+03 |
| | | Mean | 2.10E+03 | **1.65E+03** | 2.80E+03 | 2.19E+03 | 2.10E+03 | 1.84E+03 | 2.28E+03 | 3.71E+03 |
| | gap | Best | 41.94% | **25.88%** | 55.95% | 39.93% | 39.81% | 32.76% | 42.02% | 56.06% |
| | | Mean | 41.94% | **26.13%** | 56.48% | 44.33% | 41.99% | 33.96% | 46.53% | 66.03% |
| JSSP12 | obj | Best | 2.06E+03 | **1.60E+03** | 2.04E+03 | 2.06E+03 | 1.85E+03 | 1.77E+03 | 2.13E+03 | 2.92E+03 |
| | | Mean | 2.06E+03 | **1.61E+03** | 2.04E+03 | 2.19E+03 | 2.03E+03 | 1.86E+03 | 2.34E+03 | 3.84E+03 |
| | gap | Best | 40.72% | **23.56%** | 39.99% | 40.60% | 34.00% | 30.98% | 42.58% | 58.09% |
| | | Mean | 40.72% | **24.20%** | 39.99% | 44.03% | 39.27% | 34.22% | 47.60% | 67.56% |
| JSSP13 | obj | Best | 2.07E+03 | **1.60E+03** | 2.01E+03 | 1.88E+03 | 1.91E+03 | 1.73E+03 | 2.23E+03 | 3.02E+03 |
| | | Mean | 2.07E+03 | **1.61E+03** | 2.01E+03 | 2.16E+03 | 2.07E+03 | 1.79E+03 | 2.34E+03 | 3.60E+03 |
| | gap | Best | 43.04% | **26.08%** | 41.40% | 37.12% | 38.11% | 31.65% | 47.20% | 60.93% |
| | | Mean | 43.04% | **26.57%** | 41.40% | 45.10% | 42.60% | 34.08% | 49.58% | 66.76% |
| JSSP14 | obj | Best | 2.18E+03 | **1.69E+03** | 2.11E+03 | 2.15E+03 | 2.11E+03 | 1.89E+03 | 2.31E+03 | 2.91E+03 |
| | | Mean | 2.18E+03 | **1.69E+03** | 2.11E+03 | 2.28E+03 | 2.19E+03 | 1.92E+03 | 2.48E+03 | 3.32E+03 |
| | gap | Best | 40.81% | **23.38%** | 38.84% | 40.06% | 38.67% | 31.51% | 44.02% | 55.70% |
| | | Mean | 40.83% | **23.66%** | 38.84% | 43.37% | 40.87% | 32.72% | 47.91% | 60.62% |
| JSSP15 | obj | Best | 2.09E+03 | **1.63E+03** | 2.10E+03 | 1.97E+03 | 1.96E+03 | 1.77E+03 | 2.11E+03 | 3.04E+03 |
| | | Mean | 2.09E+03 | **1.64E+03** | 2.15E+03 | 2.23E+03 | 2.13E+03 | 1.82E+03 | 2.36E+03 | 3.85E+03 |
| | gap | Best | 41.29% | **24.86%** | 41.54% | 37.56% | 37.27% | 30.72% | 41.85% | 59.62% |
| | | Mean | 41.29% | **24.97%** | 42.86% | 44.74% | 41.89% | 32.66% | 47.64% | 67.10% |
| JSSP16 | obj | Best | 2.47E+03 | **1.76E+03** | 1.76E+04 | 2.24E+03 | 2.13E+03 | 1.93E+03 | 2.57E+03 | 3.17E+03 |
| | | Mean | 2.47E+03 | **1.77E+03** | 1.76E+04 | 2.36E+03 | 2.27E+03 | 1.98E+03 | 2.63E+03 | 3.39E+03 |
| | gap | Best | 59.92% | **43.88%** | 94.37% | 55.82% | 53.43% | 48.78% | 61.49% | 68.72% |
| | | Mean | 59.92% | **44.07%** | 94.37% | 57.96% | 56.26% | 50.03% | 62.35% | 70.74% |
| JSSP17 | obj | Best | 2.44E+03 | **1.84E+03** | 1.67E+04 | 2.22E+03 | 2.29E+03 | 2.01E+03 | 2.61E+03 | 3.14E+03 |
| | | Mean | 2.44E+03 | **1.87E+03** | 1.67E+04 | 2.31E+03 | 2.38E+03 | 2.04E+03 | 2.68E+03 | 3.71E+03 |
| | gap | Best | 60.07% | **46.98%** | 94.16% | 56.04% | 57.44% | 51.40% | 62.66% | 68.90% |
| | | Mean | 60.07% | **47.72%** | 94.16% | 57.74% | 59.00% | 52.26% | 63.60% | 73.40% |
| JSSP18 | obj | Best | 2.53E+03 | **1.82E+03** | 1.80E+04 | 2.36E+03 | 2.28E+03 | 2.03E+03 | 2.58E+03 | 3.07E+03 |
| | | Mean | 2.53E+03 | **1.83E+03** | 1.80E+04 | 2.45E+03 | 2.32E+03 | 2.05E+03 | 2.69E+03 | 3.30E+03 |
| | gap | Best | 60.96% | **45.68%** | 94.51% | 58.05% | 56.70% | 51.26% | 61.76% | 67.86% |
| | | Mean | 60.96% | **45.87%** | 94.51% | 59.68% | 57.45% | 51.79% | 63.25% | 69.75% |
| JSSP19 | obj | Best | 2.50E+03 | **1.80E+03** | NAN | 2.35E+03 | 2.20E+03 | 1.99E+03 | 2.49E+03 | 2.20E+03 |
| | | Mean | 2.50E+03 | **1.80E+03** | NAN | 2.44E+03 | 2.38E+03 | 2.04E+03 | 2.64E+03 | 2.53E+03 |
| | gap | Best | 58.25% | **41.78%** | NAN | 55.57% | 52.50% | 47.36% | 58.03% | 52.39% |
| | | Mean | 58.25% | **42.01%** | NAN | 57.13% | 55.89% | 48.86% | 60.29% | 58.23% |
| JSSP20 | obj | Best | 2.53E+03 | **1.80E+03** | 1.48E+04 | 2.28E+03 | 2.29E+03 | 2.02E+03 | 2.46E+03 | 2.31E+03 |
| | | Mean | 2.53E+03 | **1.80E+03** | 1.48E+04 | 2.39E+03 | 2.37E+03 | 2.04E+03 | 2.60E+03 | 2.68E+03 |
| | gap | Best | 64.19% | **49.58%** | 93.87% | 60.24% | 60.45% | 55.11% | 63.27% | 60.77% |
| | | Mean | 64.19% | **49.58%** | 93.87% | 62.12% | 61.84% | 55.64% | 65.10% | 65.35% |
| JSSP21 | obj | Best | 2.73E+03 | **2.03E+03** | 2.39E+04 | 2.74E+03 | 2.72E+03 | 2.51E+03 | 2.91E+03 | 3.60E+03 |
| | | Mean | 2.73E+03 | **2.06E+03** | 2.39E+04 | 2.95E+03 | 2.86E+03 | 2.59E+03 | 3.08E+03 | 3.68E+03 |

| Pro. | Metric | Status | GUROBI | OR-TOOLS | SCIP | SA | VNS | LNS | TS | GA |
|---|---|---|---|---|---|---|---|---|---|---|
| | gap | Best | 54.90% | **39.31%** | 94.85% | 54.99% | 54.69% | 50.96% | 57.63% | 65.82% |
| | | Mean | 54.90% | **40.08%** | 94.85% | 58.01% | 56.87% | 52.40% | 60.01% | 66.51% |
| JSSP22 | obj | Best | 2.71E+03 | **1.90E+03** | 2.37E+04 | 2.77E+03 | 2.38E+03 | 2.34E+03 | 2.95E+03 | 3.47E+03 |
| | | Mean | 2.71E+03 | **1.92E+03** | 2.37E+04 | 2.99E+03 | 2.68E+03 | 2.38E+03 | 3.16E+03 | 3.61E+03 |
| | gap | Best | 54.63% | **35.33%** | 94.82% | 55.63% | 48.41% | 47.37% | 58.33% | 64.55% |
| | | Mean | 54.63% | **35.85%** | 94.82% | 58.61% | 53.87% | 48.39% | 61.00% | 65.91% |
| JSSP23 | obj | Best | 2.79E+03 | **2.01E+03** | 2.18E+04 | 2.72E+03 | 2.58E+03 | 2.58E+03 | 3.06E+03 | 3.33E+03 |
| | | Mean | 2.79E+03 | **2.02E+03** | 2.18E+04 | 2.92E+03 | 2.70E+03 | 2.63E+03 | 3.15E+03 | 3.69E+03 |
| | gap | Best | 55.11% | **37.75%** | 94.26% | 53.98% | 51.49% | 51.34% | 59.04% | 62.34% |
| | | Mean | 55.11% | **37.88%** | 94.26% | 57.08% | 53.53% | 52.28% | 60.18% | 65.95% |
| JSSP24 | obj | Best | 2.73E+03 | **1.98E+03** | 2.41E+04 | 2.87E+03 | 2.72E+03 | 2.40E+03 | 3.01E+03 | 3.92E+03 |
| | | Mean | 2.73E+03 | **2.00E+03** | 2.41E+04 | 2.93E+03 | 2.77E+03 | 2.48E+03 | 3.14E+03 | 4.03E+03 |
| | gap | Best | 52.95% | **35.12%** | 94.68% | 55.39% | 52.92% | 46.49% | 57.37% | 67.31% |
| | | Mean | 53.00% | **35.79%** | 94.68% | 56.20% | 53.77% | 48.21% | 59.16% | 68.18% |
| JSSP25 | obj | Best | 2.83E+03 | **2.01E+03** | 2.10E+04 | 2.83E+03 | 2.73E+03 | 2.37E+03 | 2.88E+03 | 3.63E+03 |
| | | Mean | 2.83E+03 | **2.03E+03** | 2.10E+04 | 2.97E+03 | 2.94E+03 | 2.47E+03 | 3.11E+03 | 5.86E+03 |
| | gap | Best | 57.91% | **40.65%** | 94.34% | 57.97% | 56.43% | 49.79% | 58.69% | 67.19% |
| | | Mean | 57.91% | **41.34%** | 94.34% | 59.84% | 59.42% | 51.72% | 61.59% | 78.30% |
| JSSP26 | obj | Best | 3.91E+03 | **2.76E+03** | 3.00E+04 | 3.50E+03 | 4.24E+03 | 3.42E+03 | 4.13E+03 | 5.39E+03 |
| | | Mean | 3.91E+03 | **2.76E+03** | 3.00E+04 | 3.86E+03 | 4.35E+03 | 3.58E+03 | 4.26E+03 | 5.56E+03 |
| | gap | Best | 71.96% | **60.29%** | 96.34% | 68.69% | 74.15% | 67.94% | 73.44% | 79.66% |
| | | Mean | 71.96% | **60.29%** | 96.34% | 71.51% | 74.78% | 69.31% | 74.29% | 80.29% |
| JSSP27 | obj | Best | 3.60E+03 | **2.76E+03** | 2.84E+04 | 3.66E+03 | 3.93E+03 | 3.38E+03 | 4.14E+03 | 5.33E+03 |
| | | Mean | 3.60E+03 | **2.76E+03** | 2.84E+04 | 4.61E+03 | 4.11E+03 | 3.47E+03 | 4.32E+03 | 5.56E+03 |
| | gap | Best | 70.81% | **61.92%** | 96.31% | 71.31% | 73.30% | 68.93% | 74.66% | 80.29% |
| | | Mean | 70.81% | **61.92%** | 96.31% | 75.19% | 74.47% | 69.78% | 75.67% | 81.09% |
| JSSP28 | obj | Best | 3.89E+03 | **2.68E+03** | 2.75E+04 | 3.64E+03 | 3.76E+03 | 3.23E+03 | 3.84E+03 | 5.13E+03 |
| | | Mean | 3.89E+03 | **2.68E+03** | 2.75E+04 | 5.78E+03 | 3.88E+03 | 3.28E+03 | 4.20E+03 | 5.65E+03 |
| | gap | Best | 72.59% | **60.25%** | 96.13% | 70.70% | 71.68% | 67.04% | 72.25% | 79.23% |
| | | Mean | 72.59% | **60.25%** | 96.13% | 76.04% | 72.53% | 67.57% | 74.59% | 81.05% |
| JSSP29 | obj | Best | 3.88E+03 | **2.78E+03** | 3.08E+04 | 3.79E+03 | 3.61E+03 | 3.24E+03 | 4.05E+03 | 5.11E+03 |
| | | Mean | 3.88E+03 | **2.78E+03** | 3.08E+04 | 6.10E+03 | 4.06E+03 | 3.36E+03 | 4.24E+03 | 6.60E+03 |
| | gap | Best | 72.94% | **62.24%** | 96.59% | 72.27% | 70.87% | 67.55% | 74.07% | 79.46% |
| | | Mean | 72.94% | **62.24%** | 96.59% | 76.96% | 74.01% | 68.71% | 75.23% | 83.38% |
| JSSP30 | obj | Best | 3.85E+03 | **2.72E+03** | 2.88E+04 | 3.75E+03 | 3.45E+03 | 3.15E+03 | 4.09E+03 | 5.09E+03 |
| | | Mean | 3.85E+03 | **2.72E+03** | 2.88E+04 | 3.82E+03 | 3.90E+03 | 3.30E+03 | 4.22E+03 | 6.05E+03 |
| | gap | Best | 69.57% | **56.96%** | 95.93% | 68.78% | 66.05% | 62.77% | 71.34% | 76.97% |
| | | Mean | 69.57% | **56.96%** | 95.93% | 69.27% | 69.82% | 64.47% | 72.18% | 79.90% |
| JSSP31 | obj | Best | 4.04E+03 | **2.76E+03** | NAN | 5.01E+03 | 4.91E+03 | 4.52E+03 | 5.45E+03 | 9.56E+03 |
| | | Mean | 4.04E+03 | **2.76E+03** | NAN | 5.44E+03 | 5.37E+03 | 4.75E+03 | 5.71E+03 | 1.10E+04 |
| | gap | Best | 68.12% | **53.21%** | NAN | 74.29% | 73.75% | 71.49% | 76.36% | 86.51% |
| | | Mean | 68.12% | **53.27%** | NAN | 76.22% | 75.95% | 72.81% | 77.41% | 88.14% |
| JSSP32 | obj | Best | 4.34E+03 | **2.87E+03** | 4.02E+04 | 5.38E+03 | 4.48E+03 | 4.47E+03 | 5.46E+03 | 8.95E+03 |
| | | Mean | 4.34E+03 | **2.89E+03** | 4.02E+04 | 5.76E+03 | 4.66E+03 | 4.84E+03 | 5.61E+03 | 1.05E+04 |
| | gap | Best | 70.44% | **55.23%** | 96.81% | 76.11% | 71.32% | 71.30% | 76.48% | 85.66% |
| | | Mean | 70.44% | **55.49%** | 96.81% | 77.66% | 72.38% | 73.38% | 77.10% | 87.64% |

| Pro. | Metric | Status | GUROBI | OR-TOOLS | SCIP | SA | VNS | LNS | TS | GA |
|---|---|---|---|---|---|---|---|---|---|---|
| JSSP33 | obj | Best | 4.01E+03 | **2.70E+03** | NAN | 5.45E+03 | 4.24E+03 | 4.47E+03 | 5.11E+03 | 9.71E+03 |
| | | Mean | 4.01E+03 | **2.70E+03** | NAN | 5.73E+03 | 4.31E+03 | 4.66E+03 | 5.24E+03 | 1.12E+04 |
| | gap | Best | 66.74% | **50.60%** | NAN | 75.52% | 68.53% | 70.16% | 73.86% | 86.25% |
| | | Mean | 66.74% | **50.60%** | NAN | 76.69% | 69.06% | 71.33% | 74.50% | 87.96% |
| JSSP34 | obj | Best | 4.31E+03 | **2.85E+03** | 3.94E+04 | 5.61E+03 | 4.77E+03 | 4.61E+03 | 5.57E+03 | 9.41E+03 |
| | | Mean | 4.31E+03 | **2.86E+03** | 3.94E+04 | 5.89E+03 | 4.97E+03 | 4.83E+03 | 5.70E+03 | 1.10E+04 |
| | gap | Best | 68.86% | **52.84%** | 96.59% | 76.07% | 71.86% | 70.89% | 75.89% | 85.74% |
| | | Mean | 68.86% | **53.00%** | 96.59% | 77.18% | 72.97% | 72.18% | 76.45% | 87.59% |
| JSSP35 | obj | Best | 4.14E+03 | **2.78E+03** | NAN | 5.64E+03 | 6.84E+03 | 4.40E+03 | 5.34E+03 | 8.93E+03 |
| | | Mean | 4.14E+03 | **2.79E+03** | NAN | 5.77E+03 | 7.35E+03 | 4.62E+03 | 5.88E+03 | 1.11E+04 |
| | gap | Best | 67.57% | **51.76%** | NAN | 76.17% | 80.37% | 69.46% | 74.85% | 84.95% |
| | | Mean | 67.57% | **51.79%** | NAN | 76.69% | 81.70% | 70.91% | 77.06% | 87.72% |

### 3.10 Graph coloring problem (GC)

The experimental results for GC test suit are presented in Table S-20.

**Table S-20** Experimental results on GC test suit.

| Pro. | Metric | Status | GUROBI | OR-TOOLS | SCIP | SA | VNS | LNS | TS | GA |
|---|---|---|---|---|---|---|---|---|---|---|
| GC01 | obj | Best | 2.20E+01 | **1.60E+01** | 2.00E+01 | 1.80E+01 | 1.70E+01 | 1.70E+01 | 1.80E+01 | 1.80E+01 |
| | | Mean | 2.20E+01 | **1.60E+01** | 2.04E+01 | 1.84E+01 | 1.76E+01 | 1.82E+01 | 1.84E+01 | 1.84E+01 |
| | gap | Best | 54.55% | **37.50%** | 50.00% | 44.44% | 41.18% | 41.18% | 44.44% | 44.44% |
| | | Mean | 54.55% | **37.50%** | 50.95% | 45.61% | 43.14% | 44.96% | 45.61% | 45.61% |
| GC02 | obj | Best | 2.10E+01 | **1.60E+01** | 2.30E+01 | 1.80E+01 | 1.80E+01 | 1.80E+01 | 1.80E+01 | 1.80E+01 |
| | | Mean | 2.10E+01 | **1.60E+01** | 2.30E+01 | 1.80E+01 | 1.80E+01 | 1.80E+01 | 1.86E+01 | 1.86E+01 |
| | gap | Best | 47.62% | **31.25%** | 52.17% | 38.89% | 38.89% | 38.89% | 38.89% | 38.89% |
| | | Mean | 47.62% | **31.25%** | 52.17% | 38.89% | 38.89% | 38.89% | 40.82% | 40.82% |
| GC03 | obj | Best | 1.80E+01 | **1.50E+01** | 2.30E+01 | 1.90E+01 | 1.80E+01 | 1.70E+01 | 1.90E+01 | 1.80E+01 |
| | | Mean | 1.80E+01 | **1.56E+01** | 2.30E+01 | 1.90E+01 | 1.80E+01 | 1.80E+01 | 1.90E+01 | 1.84E+01 |
| | gap | Best | 38.89% | **26.67%** | 52.17% | 42.11% | 38.89% | 35.29% | 42.11% | 38.89% |
| | | Mean | 38.89% | **29.42%** | 52.17% | 42.11% | 38.89% | 38.81% | 42.11% | 40.18% |
| GC04 | obj | Best | 1.90E+01 | **1.60E+01** | 2.30E+01 | 1.80E+01 | 1.70E+01 | **1.60E+01** | 1.80E+01 | 1.80E+01 |
| | | Mean | 1.90E+01 | **1.60E+01** | 2.30E+01 | 1.88E+01 | 1.76E+01 | 1.80E+01 | 1.90E+01 | 1.84E+01 |
| | gap | Best | 52.63% | **43.75%** | 60.87% | 50.00% | 47.06% | **43.75%** | 50.00% | 50.00% |
| | | Mean | 52.63% | **43.75%** | 60.87% | 52.11% | 48.82% | 49.80% | 52.58% | 51.05% |
| GC05 | obj | Best | 1.70E+01 | **1.50E+01** | 2.10E+01 | 1.80E+01 | 1.70E+01 | 1.70E+01 | 1.80E+01 | 1.80E+01 |
| | | Mean | 1.72E+01 | **1.58E+01** | 2.14E+01 | 1.82E+01 | 1.74E+01 | 1.78E+01 | 1.82E+01 | 1.86E+01 |
| | gap | Best | 47.06% | **40.00%** | 57.14% | 50.00% | 47.06% | 47.06% | 50.00% | 50.00% |
| | | Mean | 47.65% | **43.00%** | 57.92% | 50.53% | 48.24% | 49.41% | 50.53% | 51.58% |
| GC06 | obj | Best | 1.80E+01 | **1.60E+01** | 2.20E+01 | 1.80E+01 | 1.70E+01 | 1.70E+01 | 1.90E+01 | 1.80E+01 |
| | | Mean | 1.80E+01 | **1.60E+01** | 2.20E+01 | 1.88E+01 | 1.80E+01 | 1.82E+01 | 1.90E+01 | 1.88E+01 |
| | gap | Best | 38.89% | **31.25%** | 50.00% | 38.89% | 35.29% | 35.29% | 42.11% | 38.89% |
| | | Mean | 38.89% | **31.25%** | 50.00% | 41.46% | 38.81% | 39.46% | 42.11% | 41.46% |
| GC07 | obj | Best | 1.80E+01 | **1.60E+01** | 2.30E+01 | 1.80E+01 | 1.80E+01 | 1.70E+01 | 1.80E+01 | 1.80E+01 |

| Pro. | Metric | Status | GUROBI | OR-TOOLS | SCIP | SA | VNS | LNS | TS | GA |
|---|---|---|---|---|---|---|---|---|---|---|
| | | Mean | 1.80E+01 | **1.60E+01** | 2.30E+01 | 1.84E+01 | 1.80E+01 | 1.80E+01 | 1.88E+01 | 1.88E+01 |
| | gap | Best | 38.89% | **31.25%** | 52.17% | 38.89% | 38.89% | 35.29% | 38.89% | 38.89% |
| | | Mean | 38.89% | **31.25%** | 52.17% | 40.18% | 38.89% | 38.81% | 41.46% | 41.46% |
| GC08 | obj | Best | 1.80E+01 | **1.60E+01** | 2.20E+01 | 1.80E+01 | 1.70E+01 | 1.70E+01 | 1.70E+01 | 1.80E+01 |
| | | Mean | 1.82E+01 | **1.60E+01** | 2.20E+01 | 1.84E+01 | 1.74E+01 | 1.72E+01 | 1.78E+01 | 1.86E+01 |
| | gap | Best | 38.89% | **31.25%** | 50.00% | 38.89% | 35.29% | 35.29% | 35.29% | 38.89% |
| | | Mean | 39.53% | **31.25%** | 50.00% | 40.18% | 36.73% | 36.01% | 38.09% | 40.82% |
| GC09 | obj | Best | 1.70E+01 | **1.60E+01** | 2.20E+01 | 1.70E+01 | 1.70E+01 | 1.70E+01 | 1.70E+01 | 1.80E+01 |
| | | Mean | 1.70E+01 | **1.60E+01** | 2.20E+01 | 1.82E+01 | 1.76E+01 | 1.74E+01 | 1.84E+01 | 1.88E+01 |
| | gap | Best | 35.29% | **31.25%** | 50.00% | 35.29% | 35.29% | 35.29% | 35.29% | 38.89% |
| | | Mean | 35.29% | **31.25%** | 50.00% | 39.46% | 37.45% | 36.73% | 40.10% | 41.46% |
| GC10 | obj | Best | 1.80E+01 | **1.60E+01** | 2.60E+01 | 1.80E+01 | 1.70E+01 | 1.70E+01 | 1.80E+01 | 1.80E+01 |
| | | Mean | 1.80E+01 | **1.60E+01** | 2.60E+01 | 1.84E+01 | 1.78E+01 | 1.78E+01 | 1.84E+01 | 1.84E+01 |
| | gap | Best | 38.89% | **31.25%** | 57.69% | 38.89% | 35.29% | 35.29% | 38.89% | 38.89% |
| | | Mean | 38.89% | **31.25%** | 57.69% | 40.18% | 38.17% | 38.17% | 40.18% | 40.18% |
| GC11 | obj | Best | 1.80E+01 | **1.50E+01** | 2.40E+01 | 1.80E+01 | 1.80E+01 | 1.70E+01 | 1.80E+01 | 1.70E+01 |
| | | Mean | 1.80E+01 | **1.50E+01** | 2.48E+01 | 1.88E+01 | 1.80E+01 | 1.76E+01 | 1.84E+01 | 1.82E+01 |
| | gap | Best | 38.89% | **26.67%** | 54.17% | 38.89% | 38.89% | 35.29% | 38.89% | 35.29% |
| | | Mean | 38.89% | **26.67%** | 55.58% | 41.46% | 38.89% | 37.38% | 40.18% | 39.46% |
| GC12 | obj | Best | 1.90E+01 | **1.60E+01** | 2.80E+01 | 1.80E+01 | 1.70E+01 | 1.80E+01 | 1.80E+01 | 1.70E+01 |
| | | Mean | 1.90E+01 | **1.60E+01** | 2.80E+01 | 1.88E+01 | 1.78E+01 | 1.82E+01 | 1.88E+01 | 1.82E+01 |
| | gap | Best | 52.63% | **43.75%** | 67.86% | 50.00% | 47.06% | 50.00% | 50.00% | 47.06% |
| | | Mean | 52.63% | **43.75%** | 67.86% | 52.11% | 49.41% | 50.53% | 52.11% | 50.46% |
| GC13 | obj | Best | 2.20E+01 | **1.50E+01** | 2.10E+01 | 1.80E+01 | 1.70E+01 | 1.60E+01 | 1.80E+01 | 1.80E+01 |
| | | Mean | 2.20E+01 | **1.54E+01** | 2.10E+01 | 1.86E+01 | 1.78E+01 | 1.72E+01 | 1.80E+01 | 1.82E+01 |
| | gap | Best | 59.09% | **40.00%** | 57.14% | 50.00% | 47.06% | 43.75% | 50.00% | 50.00% |
| | | Mean | 59.09% | **41.50%** | 57.14% | 51.58% | 49.41% | 47.57% | 50.00% | 50.53% |
| GC14 | obj | Best | 1.80E+01 | **1.60E+01** | 2.30E+01 | 1.80E+01 | 1.80E+01 | 1.80E+01 | 1.80E+01 | 1.80E+01 |
| | | Mean | 1.88E+01 | **1.60E+01** | 2.30E+01 | 1.86E+01 | 1.80E+01 | 1.86E+01 | 1.86E+01 | 1.84E+01 |
| | gap | Best | 38.89% | **31.25%** | 52.17% | 38.89% | 38.89% | 38.89% | 38.89% | 38.89% |
| | | Mean | 41.33% | **31.25%** | 52.17% | 40.82% | 38.89% | 40.82% | 40.82% | 40.18% |
| GC15 | obj | Best | 2.10E+01 | **1.60E+01** | 2.20E+01 | 1.80E+01 | 1.70E+01 | 1.70E+01 | 1.80E+01 | 1.90E+01 |
| | | Mean | 2.10E+01 | **1.60E+01** | 2.22E+01 | 1.88E+01 | 1.78E+01 | 1.80E+01 | 1.86E+01 | 1.90E+01 |
| | gap | Best | 47.62% | **31.25%** | 50.00% | 38.89% | 35.29% | 35.29% | 38.89% | 42.11% |
| | | Mean | 47.62% | **31.25%** | 50.43% | 41.46% | 38.09% | 38.74% | 40.82% | 42.11% |
| GC16 | obj | Best | 2.00E+01 | **1.50E+01** | 2.10E+01 | 1.80E+01 | 1.70E+01 | 1.70E+01 | 1.80E+01 | 1.80E+01 |
| | | Mean | 2.00E+01 | **1.58E+01** | 2.14E+01 | 1.82E+01 | 1.74E+01 | 1.74E+01 | 1.84E+01 | 1.88E+01 |
| | gap | Best | 45.00% | **26.67%** | 47.62% | 38.89% | 35.29% | 35.29% | 38.89% | 38.89% |
| | | Mean | 45.00% | **30.33%** | 48.57% | 39.53% | 36.73% | 36.73% | 40.18% | 41.40% |
| GC17 | obj | Best | 1.90E+01 | **1.60E+01** | 2.20E+01 | 1.90E+01 | 1.80E+01 | 1.70E+01 | 1.80E+01 | 1.80E+01 |
| | | Mean | 1.90E+01 | **1.60E+01** | 2.20E+01 | 1.90E+01 | 1.84E+01 | 1.82E+01 | 1.86E+01 | 1.90E+01 |
| | gap | Best | 36.84% | **25.00%** | 45.45% | 36.84% | 33.33% | 29.41% | 33.33% | 33.33% |

| Pro. | Metric | Status | GUROBI | OR-TOOLS | SCIP | SA | VNS | LNS | TS | GA |
|---|---|---|---|---|---|---|---|---|---|---|
| | | Mean | 36.84% | **25.00%** | 45.45% | 36.84% | 34.74% | 33.95% | 35.44% | 36.77% |
| GC18 | obj | Best | 1.80E+01 | **1.60E+01** | 2.40E+01 | 1.70E+01 | 1.70E+01 | 1.70E+01 | 1.80E+01 | 1.80E+01 |
| | | Mean | 1.80E+01 | **1.60E+01** | 2.40E+01 | 1.84E+01 | 1.76E+01 | 1.80E+01 | 1.84E+01 | 1.86E+01 |
| | gap | Best | 38.89% | **31.25%** | 54.17% | 35.29% | 35.29% | 35.29% | 38.89% | 38.89% |
| | | Mean | 38.89% | **31.25%** | 54.17% | 40.10% | 37.45% | 38.81% | 40.18% | 40.82% |
| GC19 | obj | Best | 2.20E+01 | **1.60E+01** | 2.40E+01 | 1.80E+01 | 1.80E+01 | 1.70E+01 | 1.80E+01 | 1.80E+01 |
| | | Mean | 2.20E+01 | **1.60E+01** | 2.40E+01 | 1.88E+01 | 1.82E+01 | 1.82E+01 | 1.88E+01 | 1.88E+01 |
| | gap | Best | 59.09% | **43.75%** | 62.50% | 50.00% | 50.00% | 47.06% | 50.00% | 50.00% |
| | | Mean | 59.09% | **43.75%** | 62.50% | 52.11% | 50.53% | 50.46% | 52.11% | 52.11% |
| GC20 | obj | Best | 1.80E+01 | **1.50E+01** | 2.60E+01 | 1.70E+01 | 1.70E+01 | 1.60E+01 | 1.70E+01 | 1.70E+01 |
| | | Mean | 1.80E+01 | **1.50E+01** | 2.68E+01 | 1.76E+01 | 1.76E+01 | 1.66E+01 | 1.78E+01 | 1.84E+01 |
| | gap | Best | 44.44% | **33.33%** | 61.54% | 41.18% | 41.18% | 37.50% | 41.18% | 41.18% |
| | | Mean | 44.44% | **33.33%** | 62.64% | 43.14% | 43.14% | 39.71% | 43.79% | 45.49% |
| GC21 | obj | Best | NAN | **3.80E+01** | 7.90E+01 | 4.30E+01 | 4.20E+01 | 4.50E+01 | 4.30E+01 | 4.50E+01 |
| | | Mean | NAN | **3.90E+01** | 7.90E+01 | 4.46E+01 | 4.36E+01 | 4.52E+01 | 4.46E+01 | 4.66E+01 |
| | gap | Best | NAN | **68.42%** | 84.81% | 72.09% | 71.43% | 73.33% | 72.09% | 73.33% |
| | | Mean | NAN | **69.22%** | 84.81% | 73.08% | 72.47% | 73.45% | 73.08% | 74.23% |
| GC22 | obj | Best | NAN | **4.00E+01** | 7.30E+01 | 4.50E+01 | 4.30E+01 | 4.60E+01 | 4.40E+01 | 4.60E+01 |
| | | Mean | NAN | **4.00E+01** | 7.40E+01 | 4.58E+01 | 4.38E+01 | 4.70E+01 | 4.56E+01 | 4.64E+01 |
| | gap | Best | NAN | **72.50%** | 84.93% | 75.56% | 74.42% | 76.09% | 75.00% | 76.09% |
| | | Mean | NAN | **72.50%** | 85.13% | 75.98% | 74.88% | 76.59% | 75.87% | 76.29% |
| GC23 | obj | Best | NAN | **3.80E+01** | 7.90E+01 | 4.30E+01 | 4.40E+01 | 4.50E+01 | 4.30E+01 | 4.40E+01 |
| | | Mean | NAN | **3.92E+01** | 7.90E+01 | 4.50E+01 | 4.40E+01 | 4.60E+01 | 4.44E+01 | 4.62E+01 |
| | gap | Best | NAN | **76.32%** | 88.61% | 79.07% | 79.55% | 80.00% | 79.07% | 79.55% |
| | | Mean | NAN | **77.03%** | 88.61% | 79.99% | 79.55% | 80.43% | 79.72% | 80.51% |
| GC24 | obj | Best | NAN | **3.90E+01** | 7.20E+01 | 4.40E+01 | 4.40E+01 | 4.50E+01 | 4.40E+01 | 4.50E+01 |
| | | Mean | NAN | **3.96E+01** | 7.22E+01 | 4.48E+01 | 4.40E+01 | 4.60E+01 | 4.52E+01 | 4.64E+01 |
| | gap | Best | NAN | **74.36%** | 86.11% | 77.27% | 77.27% | 77.78% | 77.27% | 77.78% |
| | | Mean | NAN | **74.74%** | 86.15% | 77.68% | 77.27% | 78.26% | 77.87% | 78.44% |
| GC25 | obj | Best | NAN | **3.80E+01** | 7.90E+01 | 4.30E+01 | 4.20E+01 | 4.40E+01 | 4.40E+01 | 4.60E+01 |
| | | Mean | NAN | **3.84E+01** | 7.90E+01 | 4.40E+01 | 4.30E+01 | 4.56E+01 | 4.50E+01 | 4.66E+01 |
| | gap | Best | NAN | **73.68%** | 87.34% | 76.74% | 76.19% | 77.27% | 77.27% | 78.26% |
| | | Mean | NAN | **73.95%** | 87.34% | 77.27% | 76.73% | 78.06% | 77.77% | 78.53% |
| GC26 | obj | Best | NAN | **4.00E+01** | 7.90E+01 | 4.30E+01 | 4.30E+01 | 4.60E+01 | 4.50E+01 | 4.60E+01 |
| | | Mean | NAN | **4.00E+01** | 7.90E+01 | 4.44E+01 | 4.38E+01 | 4.70E+01 | 4.56E+01 | 4.68E+01 |
| | gap | Best | NAN | **75.00%** | 87.34% | 76.74% | 76.74% | 78.26% | 77.78% | 78.26% |
| | | Mean | NAN | **75.00%** | 87.34% | 77.47% | 77.17% | 78.72% | 78.07% | 78.63% |
| GC27 | obj | Best | NAN | **3.80E+01** | 7.00E+01 | 4.40E+01 | 4.20E+01 | 4.60E+01 | 4.30E+01 | 4.40E+01 |
| | | Mean | NAN | **3.88E+01** | 7.10E+01 | 4.46E+01 | 4.34E+01 | 4.64E+01 | 4.48E+01 | 4.56E+01 |
| | gap | Best | NAN | **71.05%** | 84.29% | 75.00% | 73.81% | 76.09% | 74.42% | 75.00% |
| | | Mean | NAN | **71.65%** | 84.51% | 75.33% | 74.65% | 76.29% | 75.43% | 75.87% |
| GC28 | obj | Best | NAN | **3.90E+01** | 7.10E+01 | 4.30E+01 | 4.40E+01 | 4.40E+01 | 4.50E+01 | 4.60E+01 |

| Pro. | Metric | Status | GUROBI | OR-TOOLS | SCIP | SA | VNS | LNS | TS | GA |
|---|---|---|---|---|---|---|---|---|---|---|
| | | Mean | NAN | **3.90E+01** | 7.22E+01 | 4.38E+01 | 4.40E+01 | 4.52E+01 | 4.56E+01 | 5.12E+01 |
| | gap | Best | NAN | **74.36%** | 85.92% | 76.74% | 77.27% | 77.27% | 77.78% | 78.26% |
| | | Mean | NAN | **74.36%** | 86.15% | 77.17% | 77.27% | 77.87% | 78.07% | 80.41% |
| GC29 | obj | Best | NAN | **3.80E+01** | 8.00E+01 | 4.50E+01 | 4.40E+01 | 4.50E+01 | 4.30E+01 | 4.60E+01 |
| | | Mean | NAN | **3.88E+01** | 8.00E+01 | 4.56E+01 | 4.44E+01 | 4.64E+01 | 4.48E+01 | 4.80E+01 |
| | gap | Best | NAN | **73.68%** | 87.50% | 77.78% | 77.27% | 77.78% | 76.74% | 78.26% |
| | | Mean | NAN | **74.22%** | 87.50% | 78.07% | 77.47% | 78.43% | 77.67% | 79.15% |
| GC30 | obj | Best | NAN | **4.00E+01** | 7.20E+01 | 4.50E+01 | 4.30E+01 | 4.40E+01 | 4.40E+01 | 4.80E+01 |
| | | Mean | NAN | **4.00E+01** | 7.30E+01 | 4.50E+01 | 4.38E+01 | 4.50E+01 | 4.48E+01 | 4.94E+01 |
| | gap | Best | NAN | **75.00%** | 86.11% | 77.78% | 76.74% | 77.27% | 77.27% | 79.17% |
| | | Mean | NAN | **75.00%** | 86.30% | 77.78% | 77.16% | 77.76% | 77.68% | 79.75% |

3.11 Radar chart and convergence curve

Fig. S-1 illustrates the radar chart of the mean gap values obtained by 5 metaheuristic algorithms across 10 problems. Among these charts, a point closer to the center of the circle indicates better mean gap values achieved by an algorithm for a given instance.

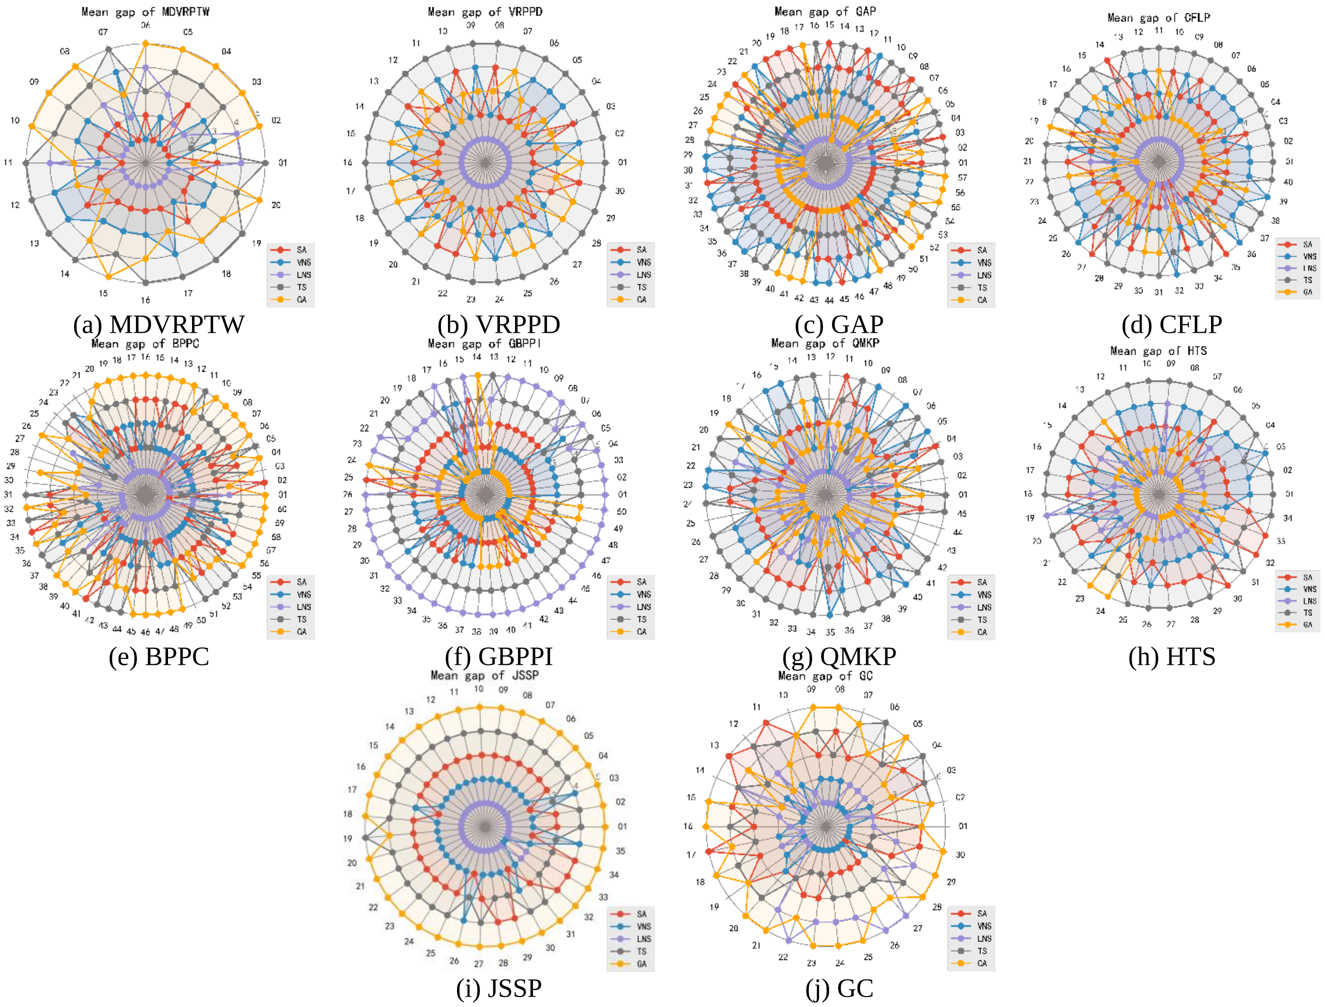


**Fig. S-1** Radar chart of mean gap for 5 metaheuristic algorithms on 10 problems.

Fig. S-2 to Fig. S-11 respectively display the convergence curve for 5 metaheuristic algorithms on 4 instances for the 10 problem types.

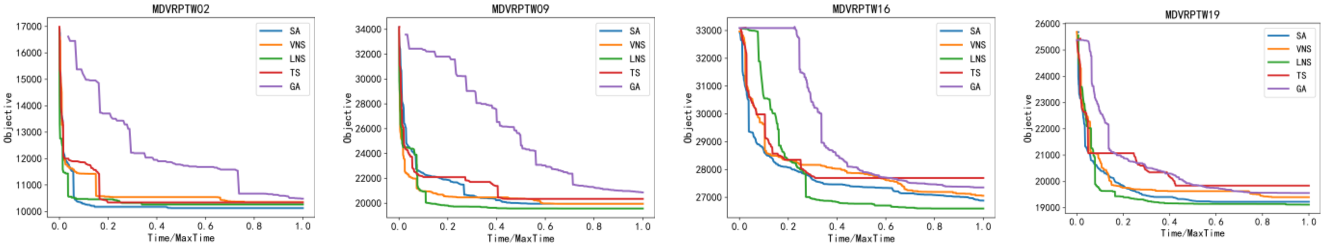


(a) MDVRPTW02 (b) MDVRPTW09 (c) MDVRPTW16 (d) MDVRPTW19

**Fig. S-2** Convergence curve for 5 metaheuristic algorithms on 4 typical MDVRPTW instances.

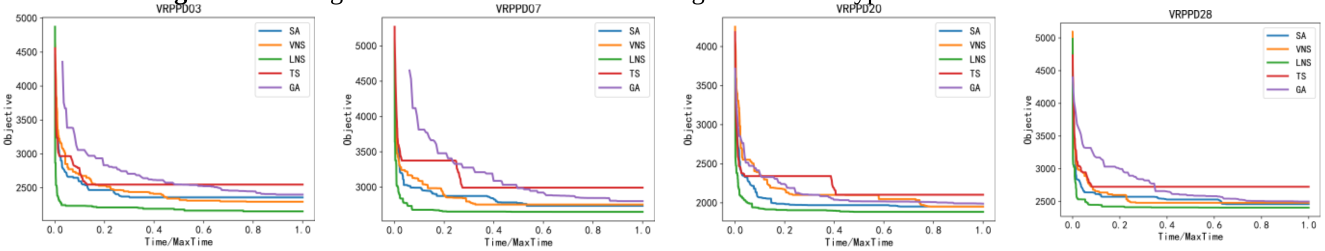


(a) VRPPD03 (b) VRPPD07 (c) VRPPD20 (d) VRPPD28

**Fig. S-3** Convergence curve for 5 metaheuristic algorithms on 4 typical VRPPD instances.

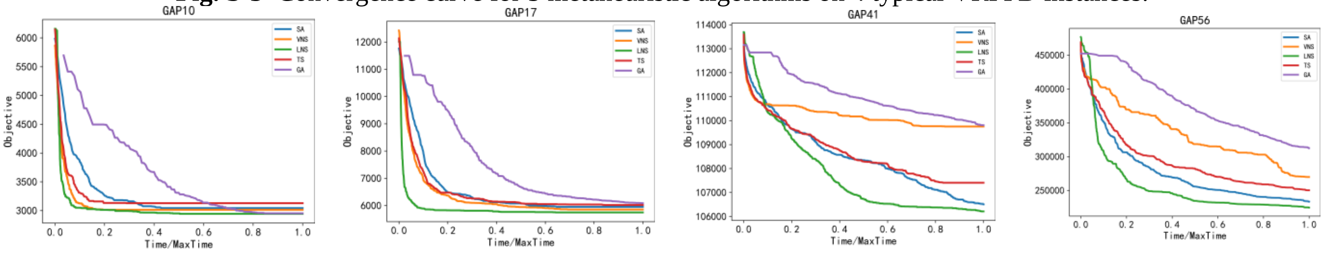


(a) GAP10 (b) GAP17 (c) GAP41 (d) GAP56

**Fig. S-4** Convergence curve for 5 metaheuristic algorithms on 4 typical GAP instances.

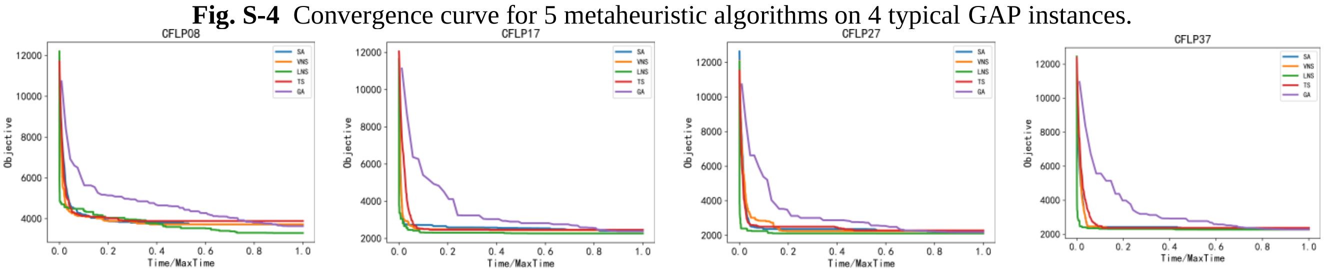


(a) CFLP08 (b) CFLP17 (c) CFLP27 (d) CFLP37

**Fig. S-5** Convergence curve for 5 metaheuristic algorithms on 4 typical CFLP instances.

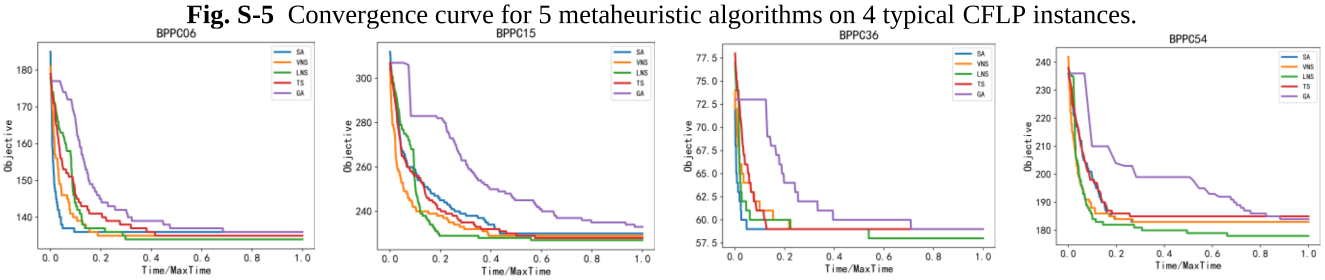


(a) BPPC06 (b) BPPC15 (c) BPPC36 (d) BPPC54

**Fig. S-6** Convergence curve for 5 metaheuristic algorithms on 4 typical BPPC instances.

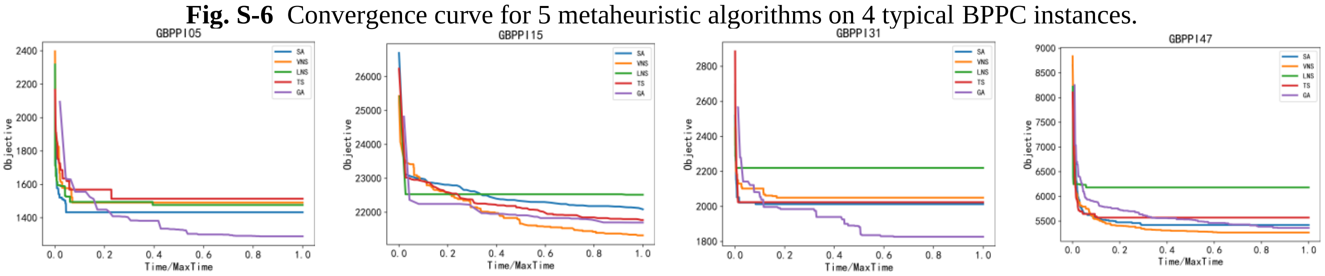


(a) GBPPI05 (b) GBPPI15 (c) GBPPI31 (d) GBPPI47

**Fig. S-7** Convergence curve for 5 metaheuristic algorithms on 4 typical GBPPI instances.

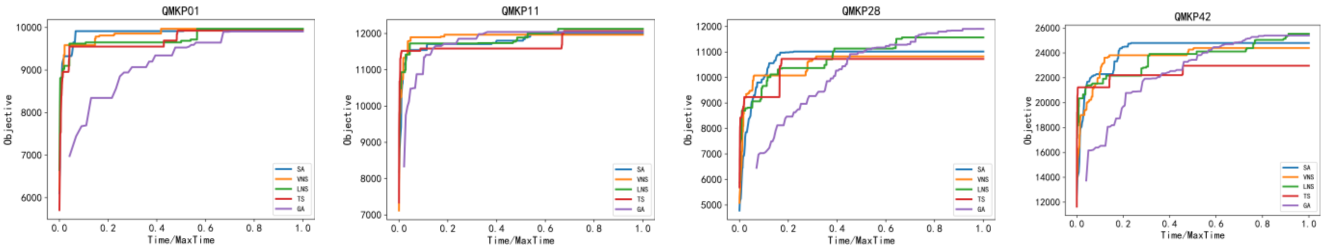


(a) QMKP01 (b) QMKP11 (c) QMKP28 (d) QMKP42

**Fig. S-8** Convergence curve for 5 metaheuristic algorithms on 4 typical QMKP instances.

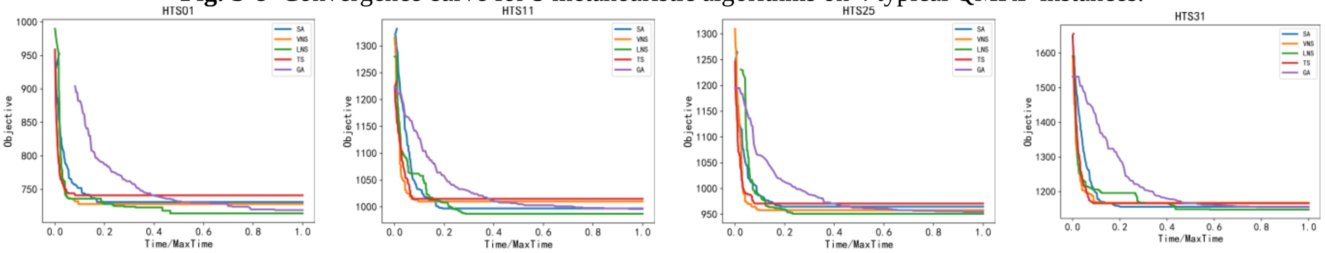


(a) HTS01 (b) HTS11 (c) HTS25 (d) HTS31

**Fig. S-9** Convergence curve for 5 metaheuristic algorithms on 4 typical HTS instances.

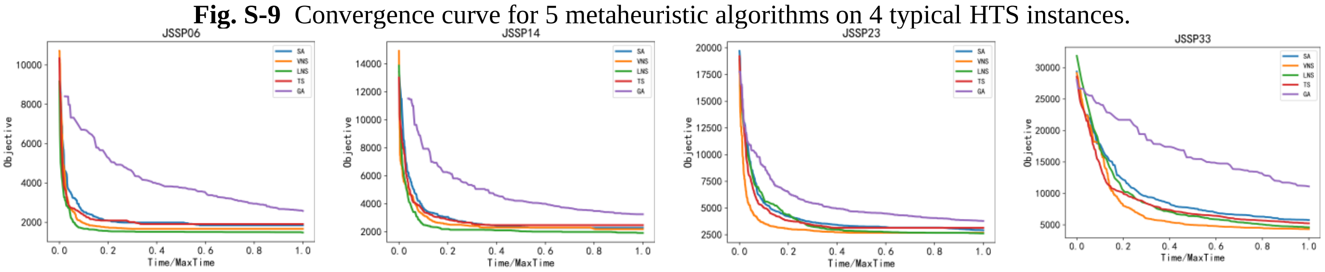


(a) JSSP06 (b) JSSP14 (c) JSSP23 (d) JSSP33

**Fig. S-10** Convergence curve for 5 metaheuristic algorithms on 4 typical JSSP instances.

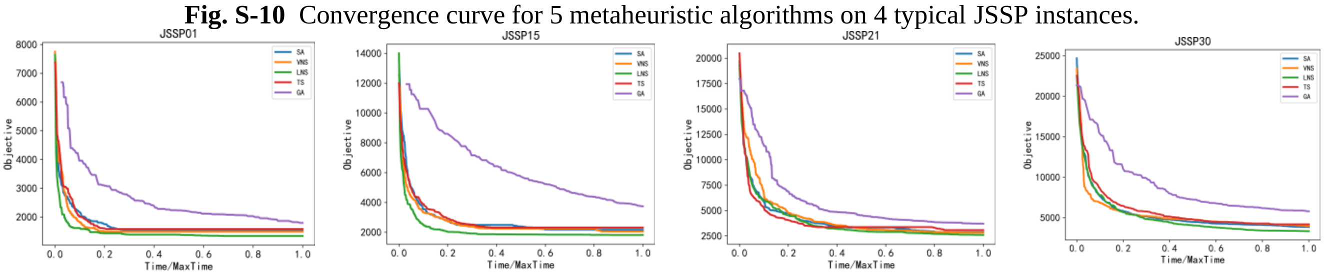


(a) GC01 (b) GC15 (c) GC21 (d) GC30

**Fig. S-11** Convergence curve for 5 metaheuristic algorithms on 4 typical GC instances.

Fig. S-12 to Fig. S-21 respectively show the convergence curve for 8 algorithms on 4 typical instances for each problem type.

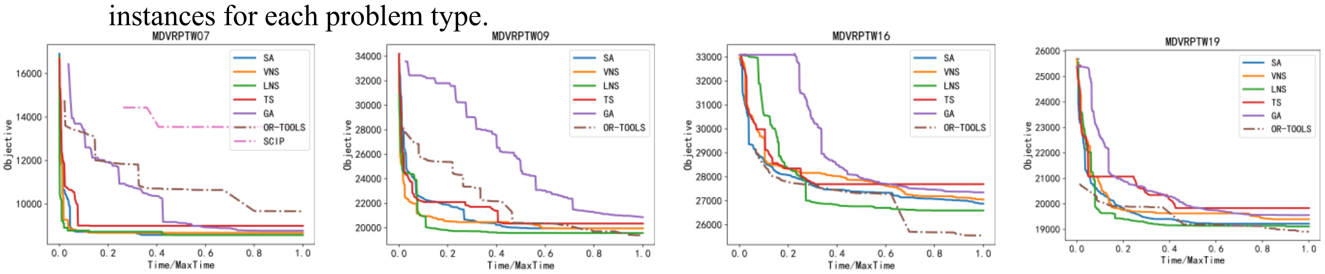


(a) MDVRPTW07 (b) MDVRPTW09 (c) MDVRPTW16 (d) MDVRPTW19

**Fig. S-12** Convergence curve for 8 metaheuristic algorithms on 4 typical MDVRPTW instances.

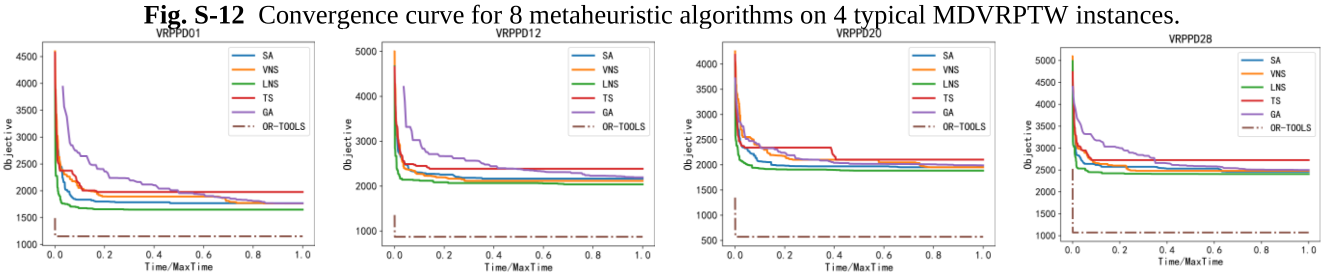


(a) VRPPD01 (b) VRPPD12 (c) VRPPD20 (d) VRPPD28

**Fig. S-13** Convergence curve for 8 metaheuristic algorithms on 4 typical VRPPD instances.

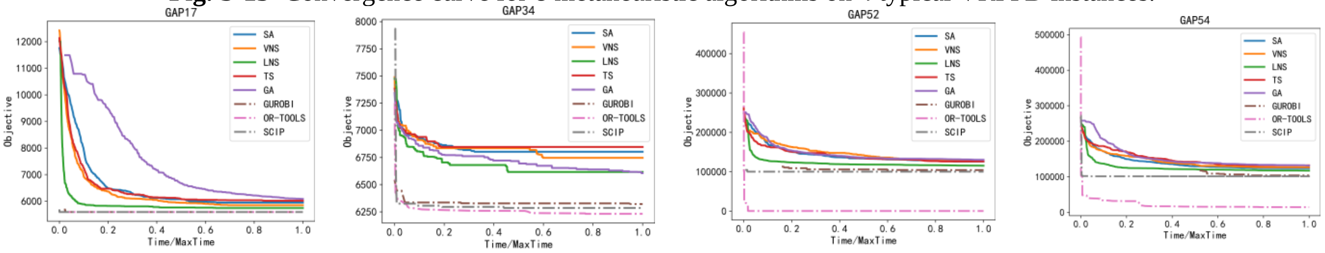


(a) GAP17 (b) GAP34 (c) GAP52 (d) GAP54

**Fig. S-14** Convergence curve for 8 metaheuristic algorithms on 4 typical GAP instances.

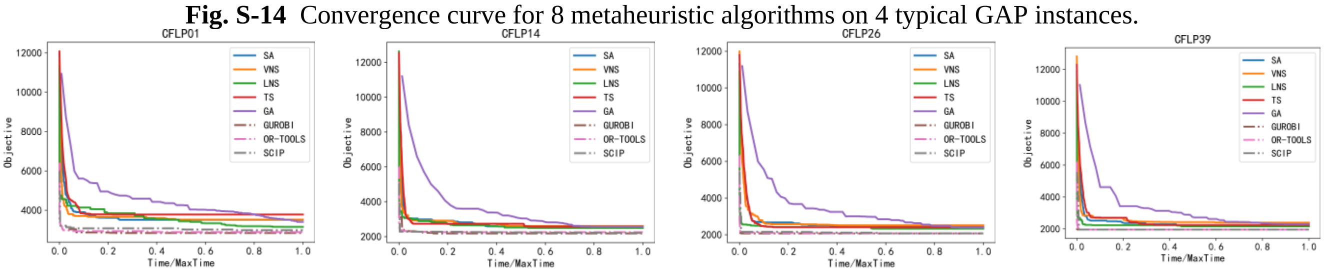


(a) CFLP01 (b) CFLP14 (c) CFLP26 (d) CFLP39

**Fig. S-15** Convergence curve for 8 metaheuristic algorithms on 4 typical CFLP instances.

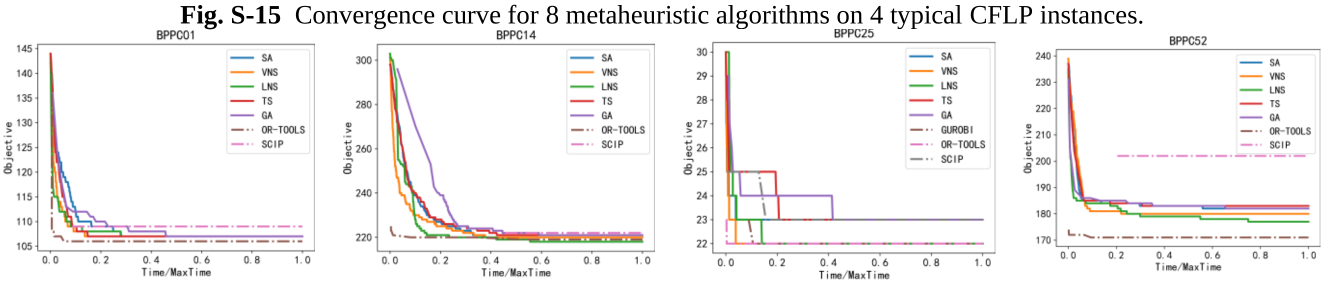


(a) BPPC01 (b) BPPC14 (c) BPPC25 (d) BPPC52

**Fig. S-16** Convergence curve for 8 metaheuristic algorithms on 4 typical BPPC problems.

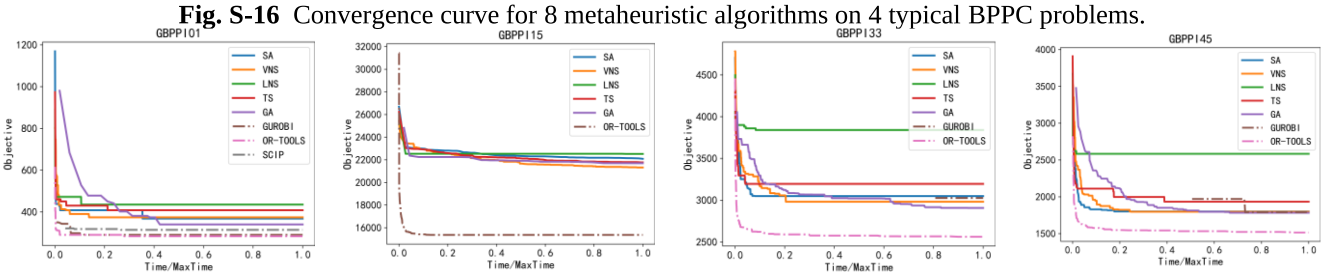


(a) GBPPI01 (b) GBPPI15 (c) GBPPI33 (d) GBPPI45

**Fig. S-17** Convergence curve for 8 metaheuristic algorithms on 4 typical GBPPI instances.

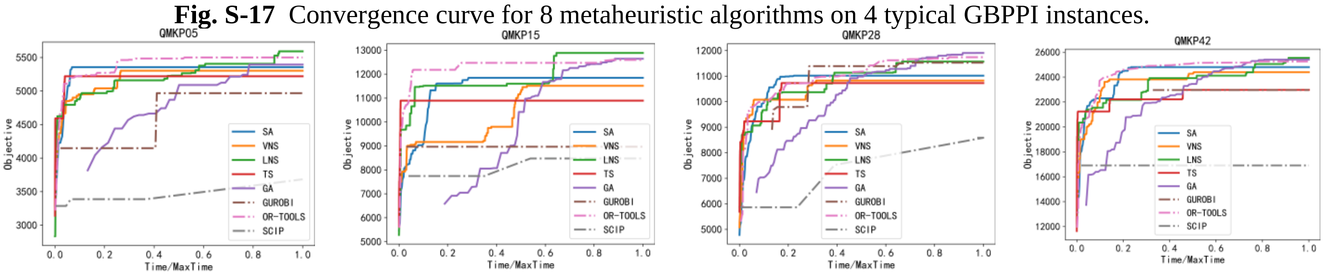


(a) QMKP05 (b) QMKP15 (c) QMKP28 (d) QMKP42

**Fig. S-18** Convergence curve for 8 metaheuristic algorithms on 4 typical QMKP instances.

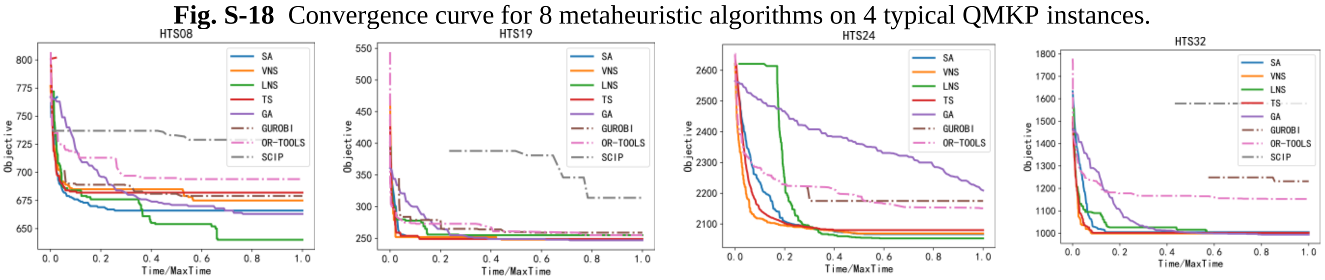


(a) HTS08 (b) HTS19 (c) HTS24 (d) HTS32

**Fig. S-19** Convergence curve for 8 metaheuristic algorithms on 4 typical HTS instances.

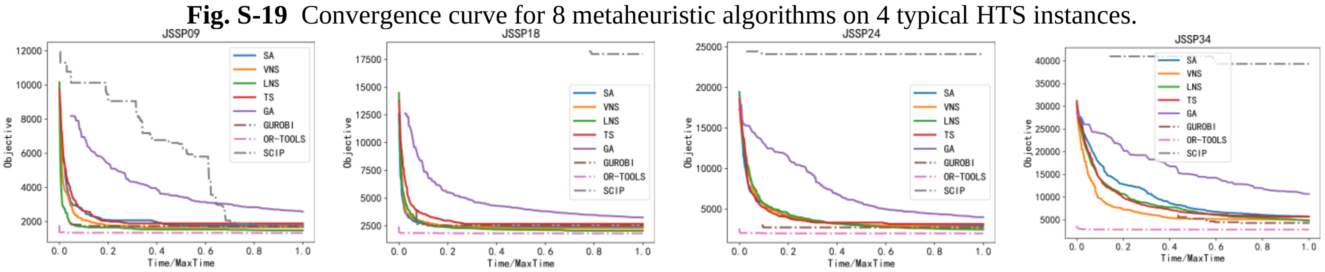


(a) JSSP09 (b) JSSP18 (c) JSSP24 (d) JSSP34

**Fig. S-20** Convergence curve for 8 metaheuristic algorithms on 4 typical JSSP instances.

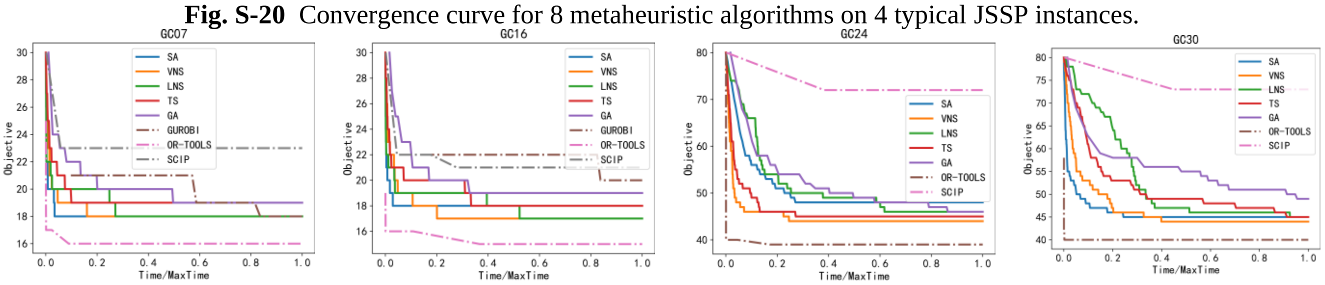


(a) GC07 (b) GC16 (c) GC24 (d) GC30

**Fig. S-21** Convergence curve for 8 metaheuristic algorithms on 4 typical GC instances.

## Reference

[1] Zhen T, Zhang Q. A hybrid metaheuristic algorithm for the multi-depot vehicle routing problem with time windows[C]//. 2009 International Conference on Networks Security, Wireless Communications and Trusted Computing: IEEE, 2009: 798-801.
[2] Van Breedam A. Comparing descent heuristics and metaheuristics for the vehicle routing problem[J]. Computers & Operations Research, 2001, 28(4): 289-315.
[3] Osman I H. Heuristics for the generalised assignment problem: simulated annealing and tabu search approaches[J]. Operations Research Spektrum, 1995, 17: 211-225.
[4] Sridharan R. The capacitated plant location problem[J]. European Journal of Operational Research, 1995, 87(2): 203-213.
[5] Muritiba A E F, Iori M, Malaguti E, et al. Algorithms for the bin packing problem with conflicts[J]. Informs Journal on Computing, 2010, 22(3): 401-415.
[6] Baldi M M, Manerba D, Perboli G, et al. A generalized bin packing problem for parcel delivery in last-mile logistics[J]. European Journal of Operational Research, 2019, 274(3): 990-999.
[7] Galli L, Martello S, Rey C, et al. Polynomial-size formulations and relaxations for the quadratic multiple knapsack problem[J]. European Journal of Operational Research, 2021, 291(3): 871-882.
[8] Saviniec L, Constantino A A. Effective local search algorithms for high school timetabling problems[J]. Applied Soft Computing, 2017, 60: 363-373.
[9] Taillard E. Benchmarks for basic scheduling problems[J]. European Journal of Operational Research, 1993, 64(2): 278-285.
[10] Fleurent C, Ferland J A. Genetic and hybrid algorithms for graph coloring[J]. Annals of Operations Research, 1996, 63(3): 437-461.
